# Supplementary material for: Collatz/Ba\v{r}ina a$n$+b conjecture proofs by 16/64: Cayley a$n$+b tree not Cantor-G\"odel-Conway-Wolfram undecidable
Source: arXiv:2008.13643 ancillary file (2026-10-21)
Supplement: Supplementary file 1 [file SupplementAutCollatzTree.pdf]

# Supplementary Materials

“The Collatz tree as an automorphism graph:  
a cotree density proof of the  $3n + 1$  conjecture”

*Jan Kleinnijenhuis, Alissa M. Kleinnijenhuis & Mustafa G. Aydogan*

## Contents

|                                                                                               |    |
|-----------------------------------------------------------------------------------------------|----|
| Detailing the cotree density method .....                                                     | 2  |
| Extended Data Fig. 1   Paired upward subtrees and cotrees .....                               | 5  |
| Extended Data Fig. 2   Paired rightward subtrees and cotrees .....                            | 7  |
| Extended Data Fig. 3   Argument expansion by 3 yields periodic rightward iterates .....       | 8  |
| Extended Definition 4   Subtree and cotree congruence classes in the automorphism graph ..... | 9  |
| Acknowledgements and references .....                                                         | 10 |

The density proof here is a variant on the density proof based on node subsets removed from a binary Collatz tree of odd numbers  $[1,5]_6$  in <https://arxiv.org/abs/2008.13643>, v1 (August 2020), in which the correspondence between removed subsets and the node sets of cotrees in the automorphism graph of the binary tree was implicit.

The functions to define and depict the Collatz tree are included in the supplementary Mathematica notebook Math12AutCollatztree.nb, of which a pdf-version (91p.) is included also. The functions are preceded by short explanations. The Mathematica notebook underlies the Tables and Figures in the main text and in the supplementary materials.

## Detailing the cotree density method

Conducting an assessment of the cumulative density of congruence classes of upward and rightward cotrees in the automorphism graph of the binary tree (Def. 4, Fig.5, Propositions 5-7) is our method of proving the Collatz conjecture. The Extended Data Figures 1-2 visualise, in addition to Figs.3-4, the definition of cotrees  $T_j = R_j U_0^j(T_{\geq 0})$  and  $t_k = U_k R_0^k(T_{\geq 0})$ . The Extended Data Table 1 extends the specification of the (numbers of) congruence classes in Figure 5 and Propositions (5-7) to all subtrees and cotrees in the automorphism graph, based on their derivations below. Detailed attention is given to rightward argument expansions by  $\theta_R = 16/3$  to derive the congruence classes of rightward subtrees and cotrees (Extended Data Fig. 3).

### Upward subtrees and cotrees

The first even upward cotree  $T_2$  (Proposition 5), based on the upward density decay  $r_{U_2} = 1/2^{3 \cdot 2}$  and  $U_0^2(n) = 2^{3 \cdot 2}n$ , is a special case of any even upward cotree  $T_j$  (Proposition 9), based on the even upward periodicity factor  $r_{U_j} = 1/2^{3j}$  and  $U_0^j(n) = 2^{3j}n$  for even  $j = 0, 2, 4, \dots$

$$\begin{aligned} T_{j \in 0, 2, 4, \dots}[\square, \square]_{\square} &= R_j U_0^j(T_{\geq 0}[c5, c27]_{288}) = \dots \\ &= R_j(T_{\geq j}[(c5, c27) \cdot 2^{3j}]_{288 \cdot 2^{3j}}) = T_j[c27 \cdot 2^{3j}]_{288 \cdot 2^{3j}} \\ \text{Density even upward cotree } \rho(T_j) &= 27/(288 \cdot 2^{3j}) \end{aligned} \tag{9}$$

For example, since  $[22]_{288}$  is a  $c27$  congruence class,  $[22 \cdot 2^{3 \cdot 4}]_{288 \cdot 2^{3 \cdot 4}} = [90 \ 112]_{1 \ 179 \ 648}$  is a congruence class both of subtree  $T_{\geq 4}$  and cotree  $T_4$ .

Given the definition of the congruence classes of the first odd subtree  $T_{\geq 1}[c8, c72]_{288 \cdot 2^4}$  in proposition 6, applying the density decay factor  $r_{U_2} = 1/2^{3 \cdot 2}$  yields the upward periodicity factor  $r_{U_i} = 1/2^{3i-3}$  and  $U_0^i(n) = 2^{3i+1}n$  for odd  $i = 1, 3, 5, \dots$  (Proposition 10).

$$\begin{aligned} T_{i \in 1, 3, 5, \dots}[\square, \square]_{\square} &= R_i U_0^i(T_{\geq 0}[c5, c27]_{288}) = \dots \\ &= R_i(T_{\geq i}[(c8, c72) \cdot 2^{3i-3}]_{288 \cdot 2^{3i+1}}) = T_i[c72 \cdot 2^{3i-3}]_{288 \cdot 2^{3i+1}} \\ \text{Density odd upward cotree } \rho(T_i) &= 72/(288 \cdot 2^{3i+1}) \end{aligned} \tag{10}$$

For example, since  $[88]_{288 \cdot 2^4}$  is a  $c72$  congruence class,  $[88 \cdot 2^{3 \cdot 5-3}]_{288 \cdot 2^{3 \cdot 5+1}} = [360 \ 488]_{16 \ 777 \ 216}$  is a congruence class both of subtree  $T_{\geq 5}$  and cotree  $T_5$ .

In short, upward iterates amount to multiplications by powers of two, which give an easy numerical specification of either 27 congruence classes of even cotrees or 72 congruence classes of odd upward cotrees.

### *Rightward cotrees*

At each iteration towards rightward subtrees  $t_{\geq k} = R_0^k(T_{\geq 0})$ , the argument periodicity is expanded by 3 to arrive at an output periodicity expansion of  $3\theta_R = 2^4$  (Def. 2). Equation (11) below explicates the multiplication of  $r6$  partitions of  $3c5$  and  $3c27$  (Table 1) by the rightward alignment vector  $\vec{h}_R$  | (Def. 2) in (7).

$$\begin{aligned}
t_1[\square, \square]_{\square} &= U_1 R_0^1(T_{\geq 0}[c5, c27]_{288}) = U_1 R_0^1(T_{\geq 0}[3c5, 3c27]_{288 \cdot 3}) = \dots \\
&= U_1 t_{\geq 1} \left[ \begin{array}{c} 3c5[1,4,1,4,1,4]_{\#r6} \times \vec{h}_R[4,2,1,8,4,8] \cdot \mathbf{T} \\ 3c27[15,12,15,12,15,12]_{\#r6} \times \vec{h}_R[4,2,1,8,4,8] \cdot \mathbf{T} \end{array} \right]_{288 \cdot 3 \cdot 2^4} \\
&= U_1 t_{\geq 1} \left[ \begin{array}{c} c81[15,12,15,12,15,12]_{\#r6} \\ c351[69,48,69,48,69,48]_{\#r6} \end{array} \right]_{288 \cdot 3 \cdot 2^4} \\
&= t_1[c81]_{288 \cdot 2^4}
\end{aligned} \tag{11}$$

Rightward iterates amount to an increasing number of congruence classes of cotrees  $t_k$  for  $k > 1$  without a common specification in terms of a power series (see Extended Data Figure 3). Therefore, the specification of the density decay of rightward cotrees is based on their *number* of congruence classes: from 81 in cotree  $t_{\geq 1}[c81]_{288 \cdot 2^4}$  to  $81 \cdot 13^{k-1}$  in any rightward cotree, denoted as  $t_k[c81\#13^{k-1}]_{288 \cdot 2^{4k}}$  (Suppl. Data Table 1). The actual congruence classes derive from the output expansion factor  $3\theta_R = 2^4$  (Def. 2), partitions of arguments by  $r6$  (Table 1) and multiplication by the rightward alignment vector (Def. 2) (as described earlier in the main text). Matrix multiplication by the  $r6 \times r6$  argument-output transformation matrix  $\mathbf{T}$  connects each argument subclass at the current rightward iteration to three different argument subclasses at the next one (Fig. 2, Def. 2). Using a placeholder box notation for the partitions of congruence classes by  $r6$ , we obtain:

$$\begin{aligned}
t_{\geq 1} \left[ \begin{array}{c} \square, \\ \square \end{array} \right]_{\#r_6} &= T_{\geq 0} \left[ \begin{array}{c} (1,4,1,4,1,4), \\ (15,12,15,15,12) \end{array} \right]_{\#r_6} \vec{h}_R \cdot \mathbf{T} \\
&= t_{\geq 1} \left[ \begin{array}{c} 3(15,12,15,15,12), \\ 3(69,48,69,48,69,48) \end{array} \right]_{\#r_6}
\end{aligned} \tag{12}$$

Each further rightward iteration  $k$ , which also involves multiplication by  $\vec{h}_R$  and matrix multiplication by  $\mathbf{T}$ , invariably yields partitions of the triple-expanded number of output congruence classes by  $r_6$  into  $13^{k-1}$  multiples of the three pairs of 15-12 classes and 69-48 classes above.

$$\begin{aligned}
t_{\geq k \in 1,2,3,\dots} \left[ \begin{array}{c} \square, \\ \square \end{array} \right]_{\#r_6} &= t_{\geq k-1} \left[ \begin{array}{c} \square, \\ \square \end{array} \right]_{\#r_6} \vec{h}_R \cdot \mathbf{T}, \text{ given} \\
t_{\geq 1} \left[ \begin{array}{c} 3(15,12,15,12,15,12), \\ 3(69,48,69,48,69,48) \end{array} \right]_{\#r_6} \\
&= t_{\geq k} \left[ \begin{array}{c} (15,12,15,12,15,12) \cdot 3 \cdot 13^{k-1}, \\ (69,48,69,48,69,48) \cdot 3 \cdot 13^{k-1} \end{array} \right]_{\#r_6} \text{ denoted as} \\
&= t_{\geq k} [(c81, c351) \# 13^{k-1}]_{288 \cdot 2^{4k}} \text{ in Suppl. Data Table 1} \\
&\text{(without triple expansion and } r_6 \text{ partition, with periodicity } 288 \cdot 2^{4k})
\end{aligned} \tag{13}$$

For example,  $13^{k-1}$  multiples of the three pairs of 15-12 classes amount at the next iteration to  $13^{k-1}(15,12,15,12,15,12) \times \vec{h}_R \cdot \mathbf{T} = 13^{k-1}(60,24,15,96,60,96) \cdot \mathbf{T}$  classes, which are  $13^{k-1}$  multiples of three pairs of  $(60 + 24 + 15 + 96) = 195 = 15 \cdot 13$  and  $(60 + 96) = 156 = 12 \cdot 13$  classes, which are  $13^k$  multiples of three pairs of 15-12 classes. The number of congruence classes in the rightward cotrees  $t_k$  is therefore:

$$\begin{aligned}
t_{k \in 1,2,3,\dots} [\square, \square]_{\square} &= U_k(t_{\geq k} [(c81, c351) \# 13^{k-1}]_{288 \cdot 2^{4k}}) \\
&= t_k [c81 \# 13^{k-1}]_{288 \cdot 2^{4k}}
\end{aligned} \tag{14}$$

Equation (13) reveals 13 as the nominator of the rightward density decay factor  $r_R = 13/(3\theta_R) = 13/16$ .

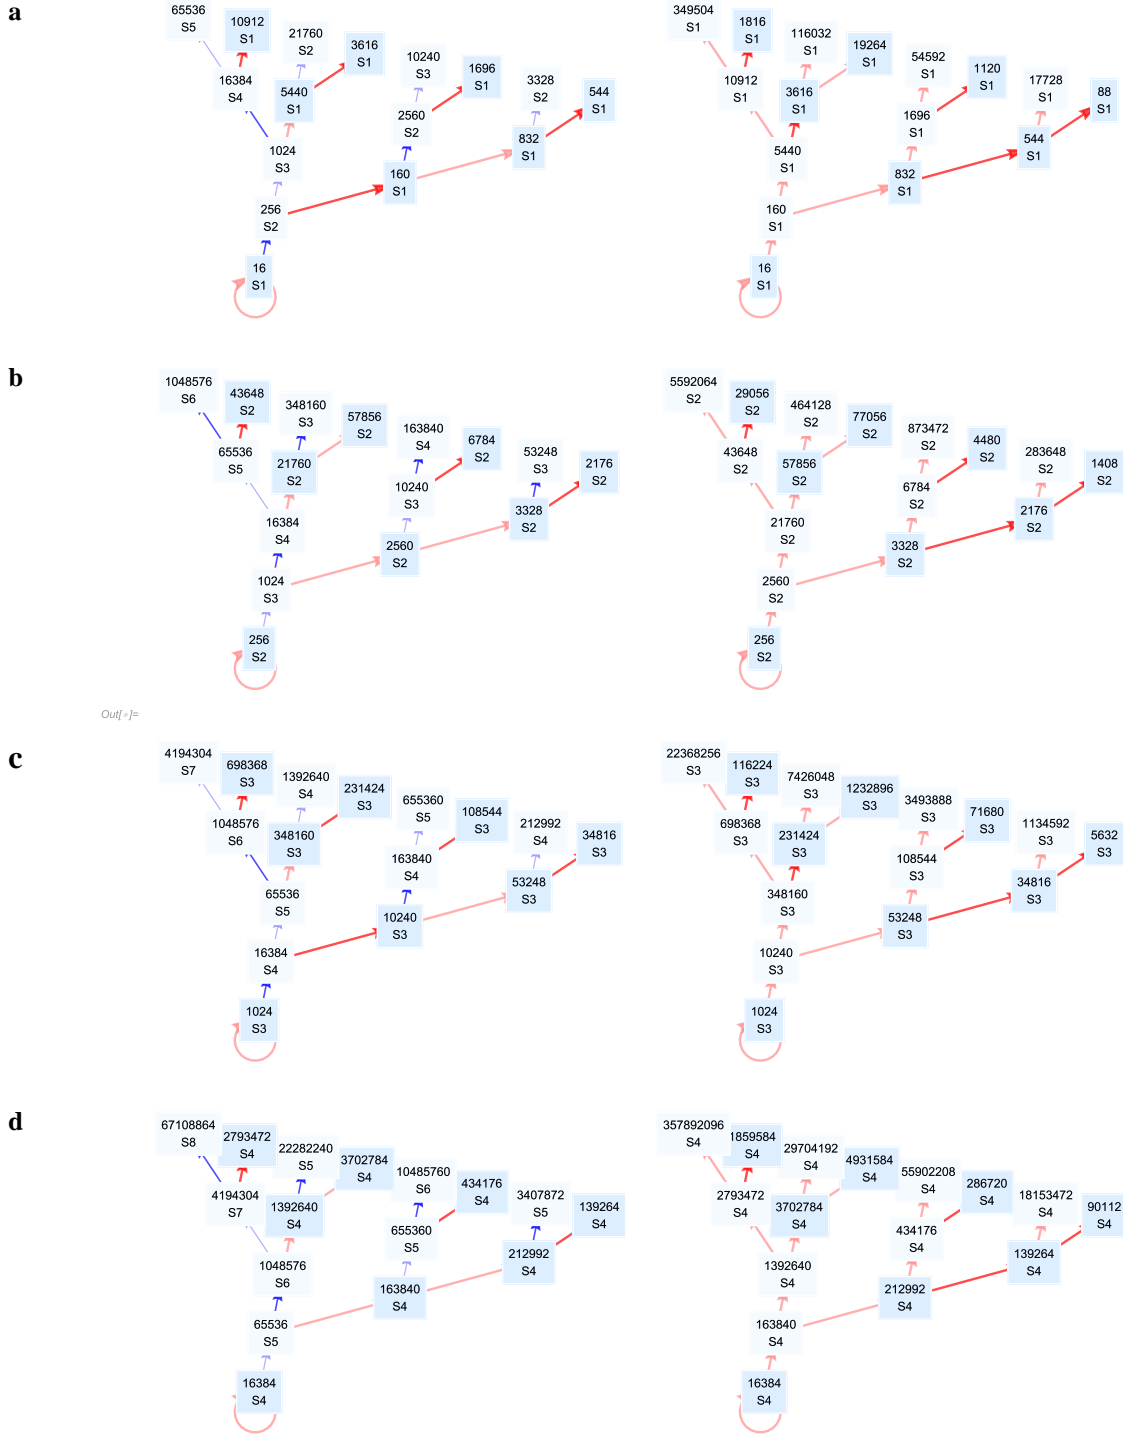

**Extended Data Fig. 1 | Paired upward subtrees and cotrees. a.** Subtree  $T_{\geq 1} = U_0^1(T_{\geq 0})$  and cotree  $T_1 = R_1 U_0^1(T_{\geq 0})$  with  $S_1$  nodes, **b.** subtree  $T_{\geq 2} = U_0^2(T_{\geq 0})$  and cotree  $T_2 = R_2 U_0^2(T_{\geq 0})$  with  $S_2$  nodes, **c.** subtree  $T_{\geq 3} = U_0^3(T_{\geq 0})$  and cotree  $T_3 = R_1 U_0^3(T_{\geq 0})$  with  $S_3$  nodes, **d.** subtree  $T_{\geq 4} = U_0^4(T_{\geq 0})$  and cotree  $T_3 = R_1 U_0^1(T_{\geq 0})$  with  $S_4$  nodes. Tree numbers can be used to verify their congruence classes (Extended Table 3). For example, 212 992 in  $T_4$  divided by  $2^{3 \cdot 4}$  is a  $c27$  class 52 listed in Table 1, which can also be seen by following numbers on corresponding nodes in ancestor trees  $T_{\geq 4} \dots T_{\geq 1}$  back to  $T_{\geq 0}$  (Fig.1b).

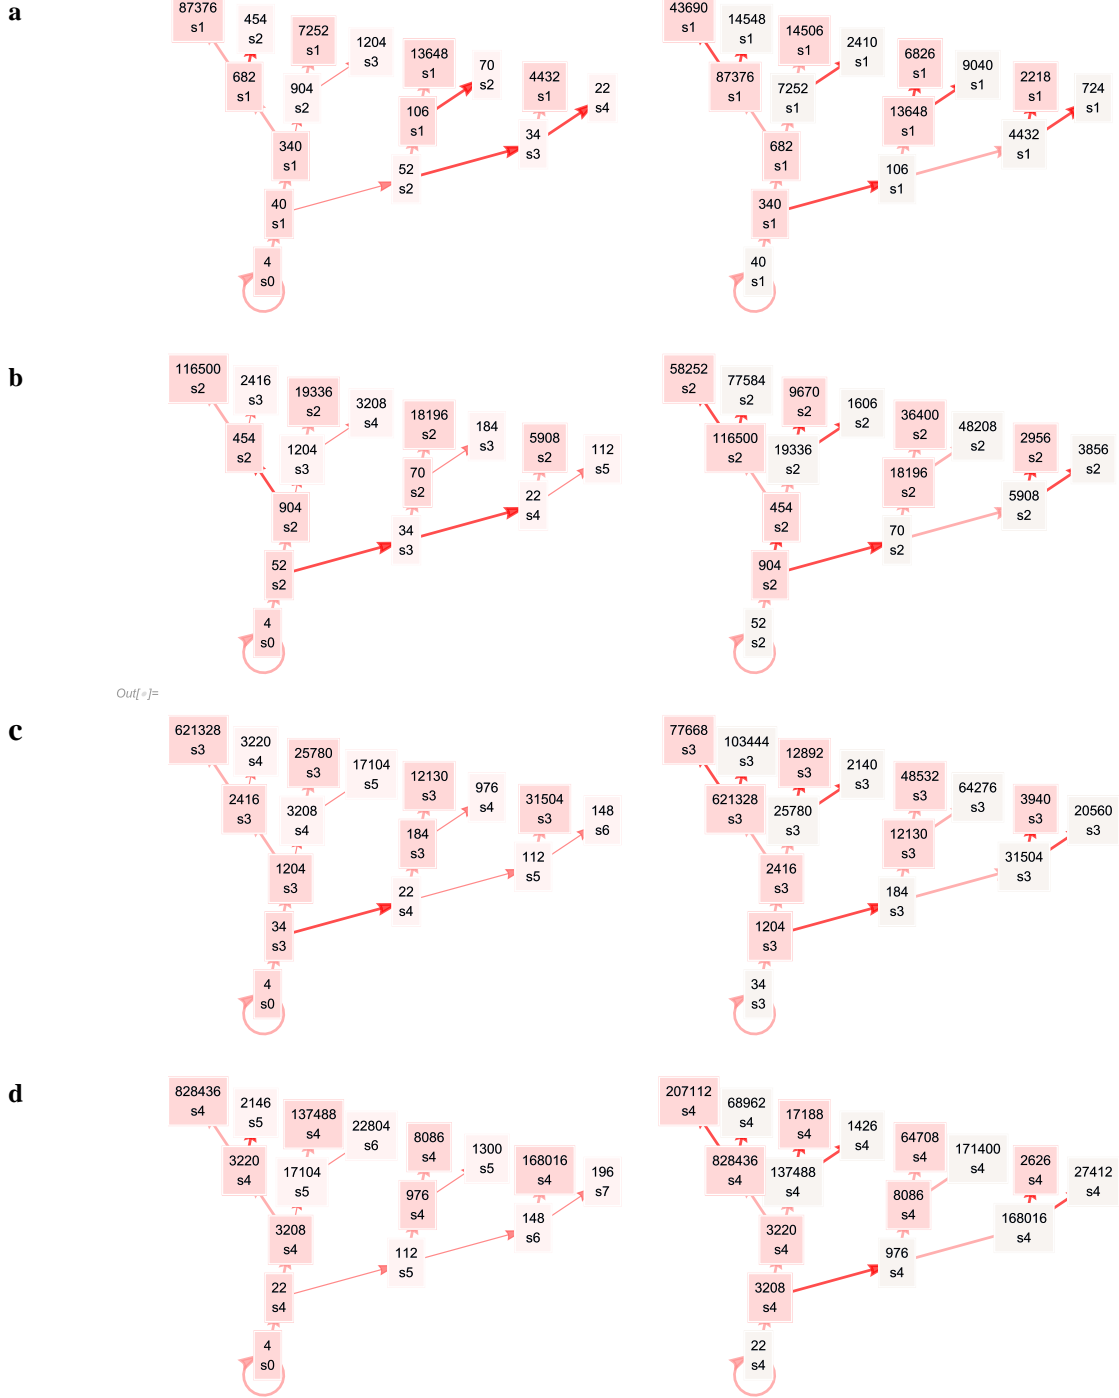

**Extended Data Fig. 2 | Paired rightward subtrees and cotrees.** **a.** Subtree  $t_{\geq 1} = R_0^1(T_{\geq 0})$  and cotree  $t_1 = U_1 R_0^1(T_{\geq 0})$  with  $s_1$  nodes, **b.** subtree  $t_{\geq 2} = R_0^2(T_{\geq 0})$  and cotree  $t_2 = U_1 R_0^2(T_{\geq 0})$  with  $s_2$  nodes, **c.** subtree  $t_{\geq 3} = R_0^3(T_{\geq 0})$  and cotree  $t_3 = U_1 R_0^3(T_{\geq 0})$  with  $s_3$  nodes, **d.** subtree  $t_{\geq 4} = R_0^4(T_{\geq 0})$  and cotree  $t_4 = U_1 R_0^4(T_{\geq 0})$  with node set  $s_4$ . Direct verification of the congruence classes of numbers in trees is harder (Extended Table 3), yet, it is simple to follow subtree generation paths. For example, the node of 3220 in  $t_4$  can be followed back in ancestor trees  $t_{\geq 4} \dots t_{\geq 1}$  back to **a.** 40 in tree  $t_{\geq 1}$ , 256 in tree  $T_{\geq 0}$  (Fig.1b) and by using  $t_4 = R_0^4 U_0(T_{\geq 0})$  (Def. 4),  $U_1[1024] = 1024$  (Fig.1b) **d.** back to  $R_0^4[1024] = 3220$ .

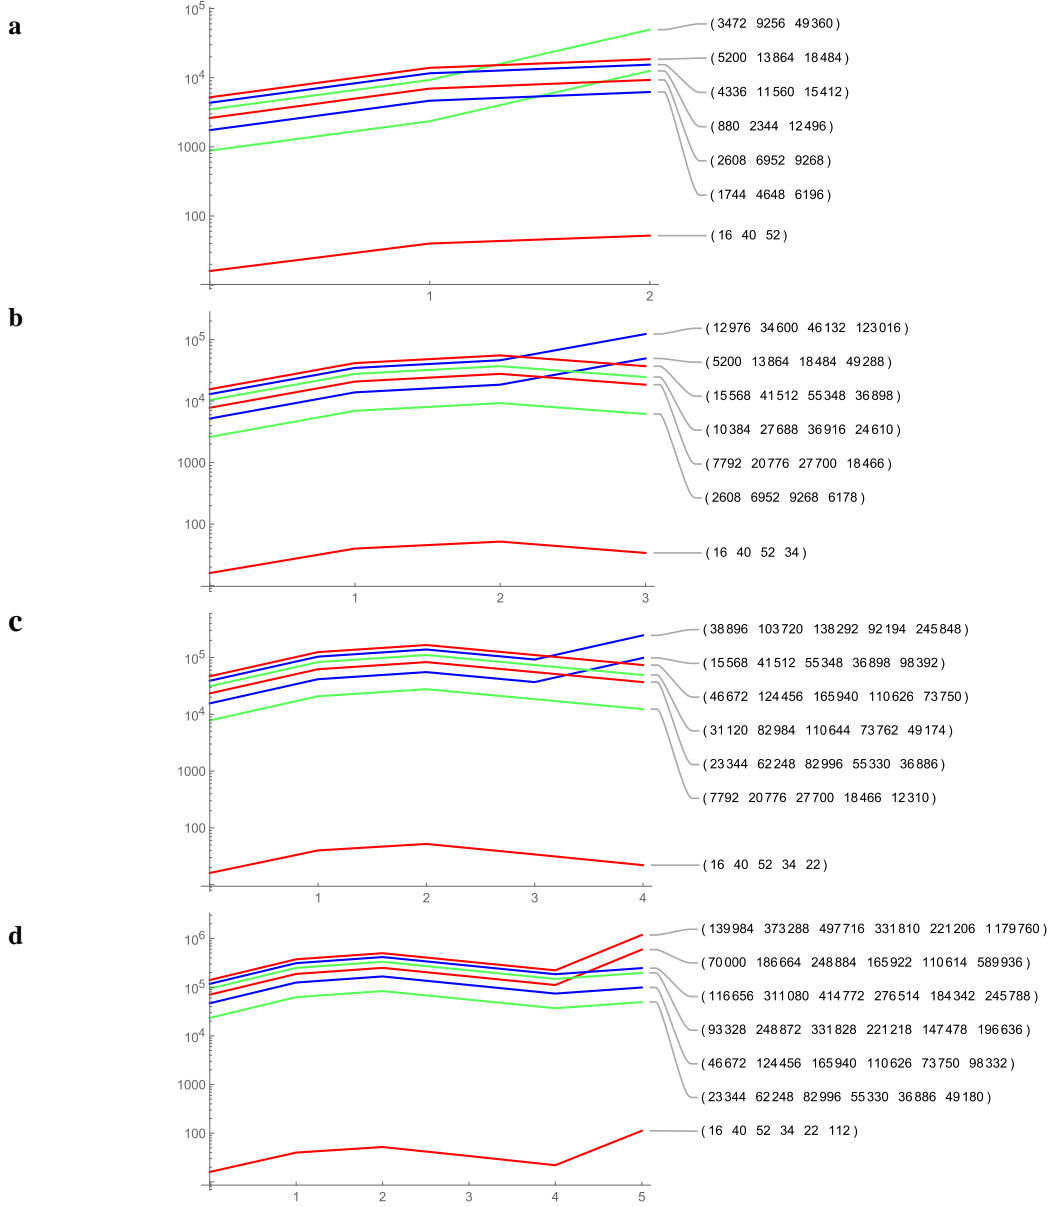

**Extended Data Fig. 3 | Argument expansion by 3 yields periodic rightward iterates.** Panels a, b, c and d show rightward iterations  $k = 1, 2, 3, 4$  applied to seven arguments,  $a_0 = 16$  and six successive arguments  $a_i = a_0 + i$  ( $288 \cdot 3^k$ ) that yield periodic rightward outputs until  $k$ . At iteration  $k + 1$  (most rightward values), every third (same colour) rightward orbit is still periodic. Periodic rightward orbits share at each iteration their congruence class modulo 54 and their  $p$ -value, giving identical slopes (Fig.2, Def.2: 1 = contraction ... 4 = steep expansion). This pattern can be exemplified by comparing a few values at each iteration (right of Figure) to their explanation below.

|                              | rightward argument<br>periodicity<br>$a_1 - a_0$ | $p(R_0^k)$ | rightward output periodicity $k$<br>$R_0^k(a_1) - R_0^k(a_0)$ | $p(R_0^{k+1})$ | triple rightward output (same<br>colour) periodicity $k+1$<br>$R_0^{k+1}(a_3) - R_0^{k+1}(a_0)$ |
|------------------------------|--------------------------------------------------|------------|---------------------------------------------------------------|----------------|-------------------------------------------------------------------------------------------------|
| <b>a. <math>k = 1</math></b> | $880 - 16 = 288 \cdot 3^1$                       | 3          | $2344 - 40 = 2^8 3^2$                                         | 2              | $9268 - 52 = 2^{10} 3^2$                                                                        |
| <b>b. <math>k = 2</math></b> | $2608 - 16 = 288 \cdot 3^2$                      | 2          | $9268 - 52 = 2^{10} 3^2$                                      | 1              | $18466 - 34 = 2^{11} 3^2$                                                                       |
| <b>c. <math>k = 3</math></b> | $7792 - 16 = 288 \cdot 3^3$                      | 1          | $18466 - 34 = 2^{11} 3^2$                                     | 1              | $36886 - 22 = 2^{12} 3^2$                                                                       |
| <b>d. <math>k = 4</math></b> | $23344 - 16 = 288 \cdot 3^4$                     | 1          | $36886 - 22 = 2^{12} 3^2$                                     | 4              | $589936 - 112 = 2^{16} 3^2$                                                                     |

**Automorphism graph  $\text{Aut}(T_{\geq 0}, U_0, R_0)$ :**

Binary root tree:  $T_{\geq 0} \left( \begin{array}{c} [c5, c27]_{288} \\ [U_0, R_0] \end{array} \right)$

Upward subtrees:  $T_{\geq j} = U_0^j(T_{\geq 0})$  yields

even upward  $T_{\geq j \in 0, 2, 4, \dots} \left( \begin{array}{c} [(c5, c27) \cdot 2^{3j}]_{288 \cdot 2^{3j}} \\ [U_0, R_j] \end{array} \right)$

odd upward  $T_{\geq i \in 1, 3, 5, \dots} \left( \begin{array}{c} [(c8, c72) \cdot 2^{3i-3}]_{288 \cdot 2^{3i+1}} \\ [U_0, R_i] \end{array} \right)$

Upward cotrees:  $T_j = U_0^j R_0^1(T_{\geq 0}) = R_1 U_0^j(T_{\geq 0})$  yields

even upward  $T_{\geq j \in 0, 2, 4, \dots} \left( \begin{array}{c} [c27 \cdot 2^{3j}]_{288 \cdot 2^{3j}} \\ [U_{j,1}, R_j] \end{array} \right)$

odd upward  $T_{i \in 1, 3, 5, \dots} \left( \begin{array}{c} [c72 \cdot 2^{3i-3}]_{288 \cdot 2^{3i+1}} \\ [U_{i,1}, R_i] \end{array} \right)$

Rightward subtrees:  $T_{\geq j} = U_0^j(T_{\geq 0})$  yields

$$t_{k \in 1, 2, 3, \dots} \left( \begin{array}{c} [(c81, c351) \# 13^{k-1}]_{288 \cdot 2^{4k}} \\ [U_k, R_0] \end{array} \right)$$

Rightward cotrees:  $t_k = U_1 R_0^k(T_{\geq 0}) = R_0^k U_0^1(T_{\geq 0})$  yields

$$t_{k \in 1, 2, 3, \dots} \left( \begin{array}{c} [c81 \# 13^{k-1}]_{288 \cdot 2^{4k}} \\ [U_k, R_0] \end{array} \right)$$

Identity non-moves:  $U_0^0, R_0^0, U_j^0, R_k^0$

Identities (dual names):  $T_{\geq 0} = t_{\geq 0}, T_{\geq 1} = t_0, t_{\geq 1} = T_0$

Conjugate functions:  $R_j = U^j R_0 U^{-j} \quad U_k = R^k U_0 R^{-k},$   
 $U_{j,1} = R^j (U_0^1 R_0 U_0^{-1}) R^{-j} \quad R_{k,1} = U^k (R_0^1 U_0 R_0^{-1}) U^{-k}$

**Extended Definition 4 | Subtree and cotree congruence classes in the automorphism graph.**

Trees are denoted in a  $G([V], [E])$  notation, in which the *Edges* are functions that generate the inner arrows, which the congruence classes  $V$  of numbers on inner nodes as domain and codomain. Node sets  $c5, c27, c8, c72, c81$  and  $c351$  are listed in Table 1 and partitioned by argument residue classes  $u2$  and  $r6$  to apply the upward and rightward functions. The congruence classes of upward subtrees and cotrees are denoted with a multiplication dot  $(c5, c27) \cdot 2^{3j}$ , expressing that they comprise the  $c5$  and  $c27$  classes multiplied by  $2^{3j}$ . The number of rightward congruence classes is denoted as  $c81 \# 13^{k-1}$ , expressing that long lists of  $351 \cdot 13^{k-1}$  and  $81 \cdot 13^{k-1}$  congruence classes are involved, which can be derived from the sets  $c351$  and  $c81$  by tree-generating functions, as explained in the context of Proposition 7.

## Acknowledgements

The authors are grateful for the constructive comments leading up to (improvements of) “The Collatz tree as a Hilbert hotel: a proof of the  $3x + 1$  conjecture” (arXiv.org/abs/2008.13643, v1 Mon, 31 Aug 2020). The density proof in “The Collatz tree as a Hilbert Hotel” was based on number subsets with a cumulative density of  $2/6$  that could be removed from a ever higher pruned binary Collatz tree with numbers from the odd classes  $[1,5]_6$  on its nodes. The automorphism graph with disjoint cotrees, each of which accommodated a removed subset, was still implicit. We are greatly indebted to the comments of Klaas Sikkels on pre-arXiv-drafts, also for the notation of different subtrees and node sets. We thank Christian Koch and Eldar Sultanow for comments, and also for implementing the binary Collatz tree in their Github repository (<https://github.com/c4ristian/collatz>). We quote the work to which the proof relates directly, but we are deeply indebted also to the enormous variety of contributions to the literature that clarified the Collatz conjecture, for example<sup>29-31</sup>. Fascination with automorphic successor relationships on the number line, in prime factorisation and among *wondrous numbers* is the legacy of Gödel, Escher and Bach.<sup>32</sup> The Online Encyclopedia of Integer Sequences<sup>5</sup> enabled the recognition of regular integer sequences, including sequences whose relationship to Collatz sequences is interesting in itself (e.g. the Van der Laan – Padovan architecture series A000931). Mathematica<sup>33</sup> enabled easy function definitions for numerical simulations and graph plots to explore the Collatz tree (Mathematica notebook included in the Ancillary Materials).

## Literature

- 1 Andersson, K. On the boundedness of Collatz sequences. <https://arxiv.org/abs/1403.7425> (2014).
- 2 Frogfanitw. <http://math.stackexchange.com/questions/1571469/collatz-modulo-18-partitions-of-collatz-3n1-trajectories> (2015).
- 3 Hofstadter, D. R. Gödel, Escher, Bach: an eternal golden braid (Basic Books, 1980).
- 4 Wolfram, S. Mathematica: a system for doing mathematics by computer (Addison Wesley Longman Publishing Co., Inc., 1991).
- 5 OEIS\_Inc. The On-line Encyclopedia of Integer Sequences <https://oeis.org>.
6. Sultanow, E., Koch, C. & Cox, S. Collatz sequences in the light of graph theory. Potsdam: Universität Potsdam. <https://doi.org/10.25932/publishup-43008>, <https://github.com/c4ristian/collatz>
