# Supplementary material for: Collatz/Ba\v{r}ina a$n$+b conjecture proofs by 16/64: Cayley a$n$+b tree not Cantor-G\"odel-Conway-Wolfram undecidable
Source: arXiv:2008.13643 ancillary file (2026-10-21)
Supplement: Supplementary file 2 [file Math12AutCollatzTree.pdf]

# The Collatz tree as an automorphism graph

a cotree density proof of the  $3x + 1$  conjecture

*Jan Kleinnijenhuis, Alissa M. Kleinnijenhuis & Mustafa G. Aydogan, Mathematica 12 version March 2022*

The functions in the notebook explore the Collatz tree. Each function or set of related functions is preceded by an introductory sentence. For some functions an example of their use is added, either in the same command separated by a semicolon (;), in the command thereafter, or in a separate subsection for interrelated functions.

The functions are not optimized for speed based on a minimum number of operations and interlinks. The functions do not warn against arguments from non-expected congruence classes; they will run forever (stop them with “Abort Evaluation” (Alt .), or give long output showing that the functions can’t handle fractions). Overlapping functions could have been integrated in generalized function with additional arguments.

The toggled comment Names below (Alt /) can be used to give, in alphabetical order, author defined names (among them many short names), and Mathematica names to handle them (most of the latter ending with \$).

```
In[2]:= (*Names["Global`*"]*)
```

The toggled comment MakeContents below from << AuthorTools' gives contents without page numbers in a separate TOC.nb-file, of which a modification is included on page 2

```
In[3]:= << AuthorTools`
```

```
In[4]:= (*MakeContents[NotebookFileName[], "Simple"]*)
```

*Contents (page numbers PDF March 2022)*

|                                                                               |    |    |
|-------------------------------------------------------------------------------|----|----|
| 1. Auxiliary functions                                                        | 3  |    |
| 2. The Collatz tree                                                           | 5  |    |
| 3. The binary Collatz tree $T \geq 0$                                         |    | 14 |
| Upward & rightward function, downward & leftward inverses                     | 14 |    |
| Upward, rightward, downward and leftward iteration functions                  | 15 |    |
| Examples of iterated binary tree functions                                    | 17 |    |
| Orbits and root paths                                                         | 19 |    |
| Finding least common multiple output congruence classes                       | 20 |    |
| 4. The Collatz clock                                                          | 27 |    |
| Congruence classes $C_5$ and $c_{27}$ and alignment vectors tree $T \geq 0$   | 27 |    |
| Congruence classes and periodicities of upward subtrees and cotrees           | 30 |    |
| Congruence classes and periodicities of rightward subtrees and cotrees        | 37 |    |
| Conjugated upward and rightward functions for nested and disjoint subtrees    | 59 |    |
| 5. Plots of the binary tree and its subtrees                                  | 61 |    |
| Auxiliary functions to plot trees                                             | 56 |    |
| Labels of edge sets and (sub) trees                                           | 62 |    |
| Edge generating functions for trees $T \geq j$ , $T_j$ and $t \geq k$ , $t_k$ | 63 |    |
| Plot functions for trees $T \geq j$ , $T_j$ and $t \geq k$ , $t_k$            | 64 |    |
| Plots of subtrees included in the main text and the supplementary materials   | 69 |    |
| 6. Excursion to the Syracuse tree                                             | 80 |    |
| 7. Densities subtrees and entire Collatz tree                                 | 85 |    |
| Plotting periodic rightward iterates                                          | 85 |    |
| Periodicity, cardinality, density                                             | 87 |    |
| Cumulative density entire Collatz tree amounts to 1                           | 91 |    |

# 1. Auxiliary functions

`factorInteger[n]` gives the usual symbolic representation of factorization provided by `FactorInteger[n]`;

```
In[5]:= factorInteger[n_] := Module[{fi},
  fi[e_] := e;
  fi[args__] := Times[args];
  fi @@ Superscript @@@ FactorInteger[n]
```

`integerFactor[superscript expression]` returns the integer that was factored with `integerFactor`

```
In[6]:= integerFactor[sup_] := If[Head[sup] != Superscript,
  Times @@ (First[#] ^ Last[#] & /@ (List @@ sup)),
  First[#] ^ Last[#] & /@ List[ (List @@ sup) ] // First]
```

`c2int` and `cl2int` are help functions that converts back a <coloured number | list of coloured numbers>, to an <integer | list of integers> .

Coloured Collatz lits of admissible integers produced by `coSeq` from the number  $n$  (see below) can be converted back to integers with: `coSeq[n] // cl2n`

```
In[7]:= c2n[colourInt_] := ToExpression[ToString[colourInt]]; cl2n[colourLst_] := c2n /@ colourLst
```

`m18[n]`, ..., `m4608[n]` are modulo 18,...,4608 functions that re-occur time and again in Collatz tree periodicities

```
In[8]:= m18[n_] := Mod[n, 18];
m96[n_] := Mod[n, 96];
m288[n_] := Mod[n, 288];
m864[n_] := Mod[n, 864];
m54[n_] := Mod[n, 54];
m4608[n_] := Mod[n, 4608]
```

`branchQ[n]` questions whether  $n$  is a number on a branching node from set  $S_{\geq 0}$ , either an u(pward) or r(ightward) number - see introduction main text

```
In[9]:= branchQ[n_] := MemberQ[{4, 16}, n // m18]
```

`upQ[n]` questions whether  $n$  is an upwards number from set  $S_{\geq 1}$  - cf definition 5 main text

```
In[10]:= upQ[n_] := MemberQ[{16, 88, 160, 232, 256}, Mod[n, 288]]
```

`n23Q[n]` questions whether  $n$  is an odd number not divisible by 2 or 3 connected by  $3n+1$  to the set of branching nodes from set  $S_{\geq 0}$  - cf test `branchQ[n]` above

```
In[11]:= n23Q[n_] := And[OddQ[n], Not[Divisible[n, 3]]];
```

up15Q questions whether  $n$  is an odd number not divisible by 2 or 3 from congruence classes  $[1, 5]_6$  connected by  $3n+1$  to an upward number from the set of branching nodes from set  $S_{\geq 0}$  - cf test branchQ[n] above

```
In[12]:= up15Q[n_] := MemberQ[{5, 29, 53, 77, 85}, Mod[n, 96]]
```

## 2. The Collatz tree

colPath gives the Collatz path starting for a positive integer  $x$  (see Figure 1 main text), obtained from ACL's contribution to <http://stackoverflow.com/questions/6535505/collatz-conjecture-in-mathematica>.

```
In[13]:= colPath[n_] := NestWhileList[
  Which[
    EvenQ[#], # / 2,
    True, 3 * # + 1] &,
  n,
  # ≠ 1 &]
```

Example: colPath[27] gives a relatively long path with a length or 'stopping time' of 112 nodes relative to the size of the argument node  $n=27$ .

```
In[14]:= colPath[27]
Out[14]= {27, 82, 41, 124, 62, 31, 94, 47, 142, 71, 214, 107, 322, 161, 484, 242, 121, 364, 182, 91, 274, 137, 412, 206, 103, 310, 155, 466, 233, 700, 350,
  175, 526, 263, 790, 395, 1186, 593, 1780, 890, 445, 1336, 668, 334, 167, 502, 251, 754, 377, 1132, 566, 283, 850, 425, 1276, 638, 319,
  958, 479, 1438, 719, 2158, 1079, 3238, 1619, 4858, 2429, 7288, 3644, 1822, 911, 2734, 1367, 4102, 2051, 6154, 3077, 9232, 4616, 2308,
  1154, 577, 1732, 866, 433, 1300, 650, 325, 976, 488, 244, 122, 61, 184, 92, 46, 23, 70, 35, 106, 53, 160, 80, 40, 20, 10, 5, 16, 8, 4, 2, 1}
```

```
In[15]:= colPath[27] // Length
Out[15]= 112
```

downtoBranch[ $n$ ] gives the number on the branching node  $S_{\geq 0}=\{4,16\} \equiv n \bmod 18$  to which iterations of the Collatz function lead a number on a non-branching node;  $n$  returns  $n$  in case  $n \in S_{\geq j}$ ; downtoBranch is a version of colPath with the stopping function branchQ[ $n$ ] whether  $n \in S_{\geq 0}$ .

```
In[16]:= downtoBranch[n_] := NestWhile[
  Which[
    EvenQ[#], # / 2,
    True, 3 * # + 1] &,
  n,
  branchQ[#] == False &]
```

uptoBranch[ $n$ ] gives the number on the branching node  $S_{\geq 0}=\{4,16\} \equiv n \bmod 18$  from which iterations of the Collatz function led to the number  $n$  on a non-

branching node;  $n$  returns  $n$  in case  $n \in S_{\geq j}$ ; uptoBranch is a version of colPath with the stopping function branchQ[ $n_{-}$ ] whether  $n \in S_{\geq 0}$ .

```
In[17]:= uptoBranch[n_] := If[Divisible[n, 3], Infinity,
  NestWhile[2 # &, n, branchQ[#] == False &]]
```

Example: how some Collatz branching nodes generated by downtoBranch and uptoBranch

```
In[18]:= Prepend[{#, downtoBranch[#], uptoBranch[#]} & /@ {16, 32, 64, 128, 256, 5, 10, 20, 40},
  {"n", "downtoBranch[n]", "uptoBranch[n]"}] // TableForm
```

Out[18]/TableForm=

| $n$ | downtoBranch[ $n$ ] | uptoBranch[ $n$ ] |
|-----|---------------------|-------------------|
| 16  | 16                  | 16                |
| 32  | 16                  | 256               |
| 64  | 16                  | 256               |
| 128 | 16                  | 256               |
| 256 | 256                 | 256               |
| 5   | 16                  | 40                |
| 10  | 16                  | 40                |
| 20  | 16                  | 40                |
| 40  | 40                  | 40                |

uptoBranchQ[ $n$ ] questions whether uptoBranch is upward (True) or rightward (False),

```
In[19]:= uptoBranchQ[n_] := Module[{n2}, n2 = n;
  If[n < 0, n2 = -n];
  If[branchQ[n2], If[upQ[n2], True, False], If[upQ[uptoBranch[n2]], True, False]]]
```

colEdges[ $n, nk$ ] gives the arrows in the Collatz tree for  $j$  levels, starting from node  $n$ . Level  $j+1$  is added to draw edges without an end node to denote that the Collatz tree is an infinite tree.

```

In[20]:= colEdges[n_, j_] := Module[{nodes, edges, newNodes, newEdges, k},
  newNodes = {If[OddQ[(# - 1) / 3], {(# - 1) / 3}, ## &[]], {2 #}} &;
  newEdges = {If[OddQ[(# - 1) / 3], {# → (# - 1) / 3}, ## &[]], {# → 2 #}} &;
  nodes = {n};
  edges = newEdges /@ nodes;
  For[k = 1, k ≤ j, k++, {
    nodes = DeleteCases[(newNodes /@ nodes) // Flatten, 1];
    edges = Append[edges, newEdges /@ nodes]
  }];
  edges = Append[Take[edges, j], Map[Rule[First[#], -Last[#]] &, Last[edges], {3}]] // Flatten]

```

negno, noneg, div3no, div23no are help functions to colTree. In the top row of a colTree invisible white styled numbers are plotted of which the edges towards them are plotted. In colEdges the numbers on this row are marked with a negative sign. negno turns a negative number into an invisible white styled number; noneg extracts the number from an invisible white styled number. div3no and div23no tests whehter a number a number is divisible by 3, respectively by 2 or 3, regardless whether it is negative or invisibly white styled.

```

In[21]:= negno[n_] := If[n < 0, Style[n, White], n];
noneg[n_] := If[NumberQ[n], n, First[n]];
div3no[n_] := If[Or[n < 0, And[n > 0, Divisible[n, 3]]], Style[n, White], n];
div23no[n_] := If[Or[n < 0, And[n > 0, Not[branchQ[n]]]], Style[n, White], n];

```





```

In[27]:= colTree3depart[n_, j_] := TreePlot[
  Rule[div3no[#[[1]]], div3no[#[[2]]]] & /@ colEdges[n, j],
  Bottom, n, PlotRangePadding → 0, VertexLabels → Placed[Automatic, Center],
  VertexShapeFunction → (Text[Framed[#2, FrameStyle → White, Background → Which[
    Not[branchQ[#2]], White,
    upQ[#2], LightBlue,
    True, LightRed]], #1] &),
  EdgeShapeFunction → ({Which[
    Divisible[noneg[Last[#2]], 3],
    Directive[Thick, Dashed, White],
    uptoBranchQ[noneg[Last[#2]]],
    Directive[Thick, Blue],
    True,
    Directive[Thick, Lighter[Red]]], Arrowheads[Medium], Arrow[#1, 0.18] &)}];
colTree3depart[1, 15]

```

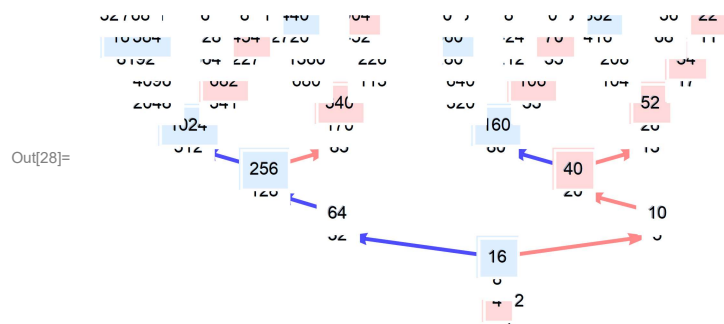

In[29]=

colTreeBranch leaves out non-branching nodes from the plot of the Collatz tree; if paths of consecutive edges with blank positions are connected the binTree is obtained

```

In[30]:= colTreeBranch[n_, j_] := TreePlot[
  Rule[div23no[#[[1]]], div23no[#[[2]]]] & /@
    colEdges[n, j], Bottom, Style[1, White], PlotRangePadding → 0, VertexLabels → Placed[Automatic, Center],
  VertexShapeFunction → (Text[Framed[ #2, FrameStyle → White, Background → Which[
    Not[branchQ[#2]], White,
    upQ[#2], Lighter[Lighter[Blue]],
    True, LightRed]], #1] &),
  EdgeShapeFunction → ({Which[
    Divisible[noneg[Last[#2]], 3],
    Directive[Thick, Dashed, White],
    uptoBranchQ[noneg[Last[#2]]],
    Directive[Thick, Blue],
    True,
    Directive[Thick, Lighter[Red]]], Arrowheads[Medium], Arrow[#1, 0.18] &)}];
colTreeBranch[1, 15]

```

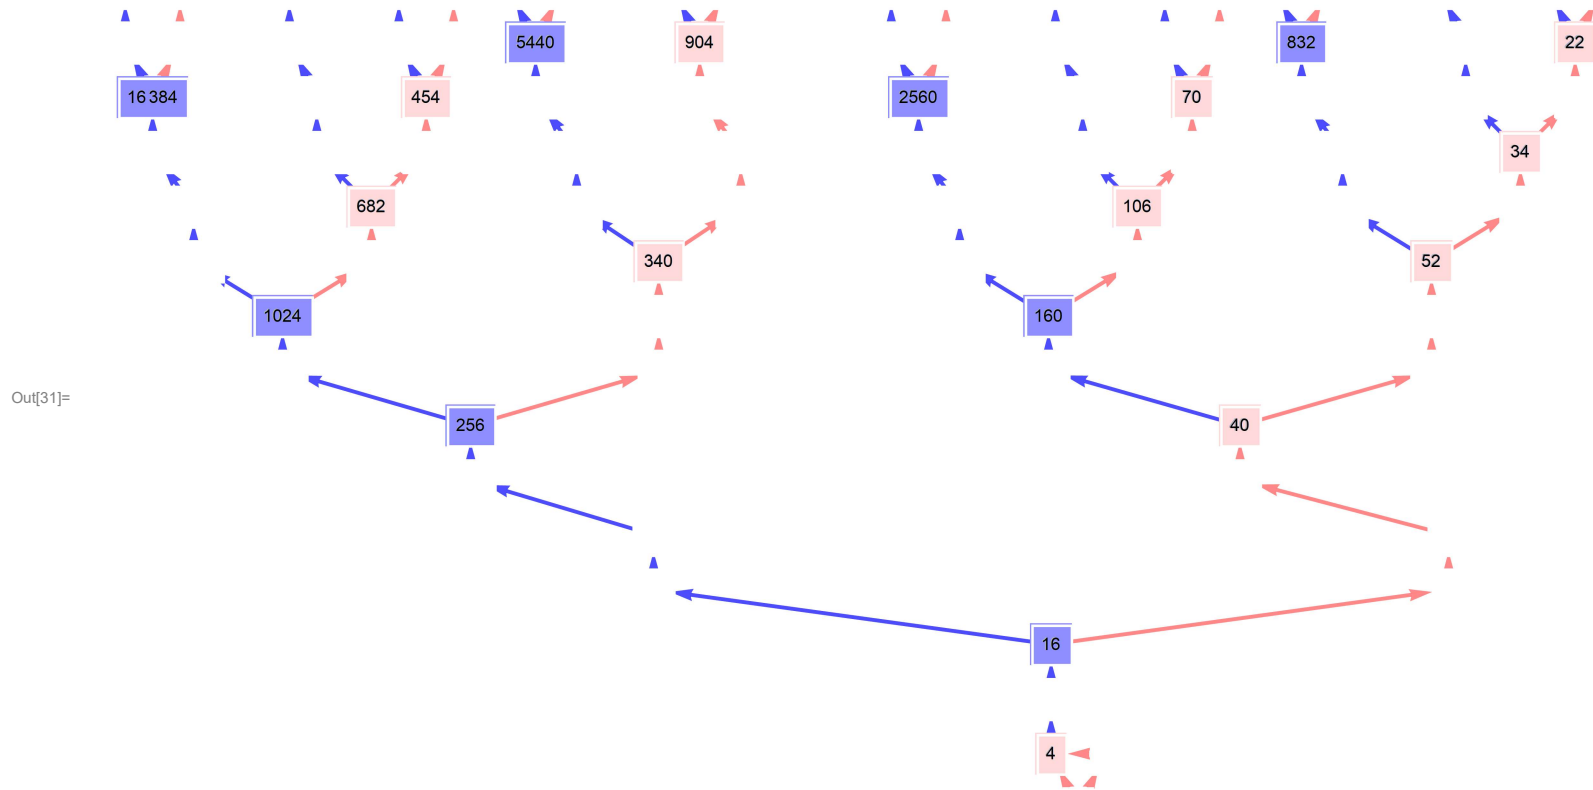

### 3. The binary Collatz tree $T_{\geq 0}$

#### Upward & rightward function, downward & leftward inverses

$u[n]$  is the upward function  $u$  for admissible numbers  $n \in S_{\geq 0}$  returning  $u[n] \in S_{\geq 1}$

```
In[32]:= u[n_] := If[m18[n] == 4, 4 n, 16 n]
```

$r[n]$  is the rightward function  $r$  for admissible numbers  $n \in S_{\geq 0}$  (which satisfy branchQ)

```
In[33]:= r[n_] := Switch[m54[n],
  4, 22 (n - 1) / 3,
  16, 23 (n - 1) / 3,
  22, 24 (n - 1) / 3,
  34, 2 (n - 1) / 3,
  40, 22 (n - 1) / 3,
  52, 2 (n - 1) / 3]
```

$d[n]$  defines the downward function as the inverse of the upward function;  $l[n]$  defines the leftward function as the inverse of the rightward function. l

```
In[34]:= d[n_] := Which[Mod[n, 18] == 4, n / 16, Mod[n, 18] == 16, n / 4]
```

```
In[35]:= l[n_] := Which[MemberQ[{16, 88, 160, 232, 256}, Mod[n, 288]], Null,
  MemberQ[{22, 34, 58, 70, 94, 106, 130, 142, 166, 178, 202, 214, 238, 250, 274, 286}, Mod[n, 288]],
  3 n / 2 + 1, MemberQ[{4, 52, 76, 124, 148, 196, 220, 268}, Mod[n, 288]], 3 n / 4 + 1,
  MemberQ[{40, 184}, Mod[n, 288]], 3 n / 8 + 1, MemberQ[{112}, Mod[n, 288]], 3 n / 16 + 1] // Expand
```

$pa[n]$  gives the parent of  $n$ , regardless whether  $n$  is an upward or rightward child

```
In[36]:= pa[n_] := If[upQ[n], d[n], l[n]]
```

contraction and expansion test whether  $n$  is either smaller or larger than  $pa[n]$ ;  $n$  is a contraction iff  $\{11, 18\} \equiv pa[n] \pmod{18}$

```
In[37]:= contraction[n_] := n < pa[n]; expansion[n_] := n > pa[n]
```

$g[n]$  is the binary tree function that forks for each  $n$  in  $r[n]$  and  $u[n]$

```
In[38]:= g[n_] := List[r[n], u[n]]
```

## upward, rightward, downward and leftward iteration functions

$uu[n, nk]$ ,  $rr[n, nk]$ ,  $dd[n, nk]$  and  $ll[n, nk]$  give paths of length  $j+1$  upward links, respectively  $k+1$  o,  $nk$  rightward links,  $j+1$  downward links and  $k+1$  leftward links, preceded by the argument  $n$ ;

$uj$  and  $rk$  give just the  $j$ 'th, respectively  $k$ 'th iteration

```
In[39]:= uj[n_, j_] := Nest[u, n, j]
```

```
In[40]:= uu[n_, j_] := NestList[u, n, j]
```

```
In[41]:= rk[n_, k_] := Nest[r, n, k]
```

```
In[42]:= rr[n_, k_] := NestList[r, n, k]
```

```
In[43]:= dj[n_, nj_] := Nest[d, n, nj]
```

```
In[44]:= lk[n_, nk_] := Nest[l, n, nk]
```

```
In[45]:= dd[n_, nj_] := NestList[d, n, nj]
```

```
In[46]:= ll[n_, nk_] := NestList[l, n, nk]
```

$ans[n, k]$  gives the ancestry of  $n$  to the  $k$ 'th degree

```
In[47]:= ans[n_, k_] := NestList[pa, n, k]
```

$uj[n, nk]$ ,  $rk[n, nk]$ ,  $dj[n, nk]$  and  $lk[n, nk]$  gives the  $nk$ 'th iteration of respectively the upward function, the rightward function, the downward function and the leftward function.

$ddd$  gives downward links until (including) the rightward number from which the upward orbit starts.

```
In[48]:= ddd[n_] := NestWhileList[d[#] &, n, upQ[#] == True &]
```

$lll$  gives leftward links until (including) the upward number  $m \in S_{\geq j}$  from which the rightward orbit starts

```
In[49]:= lll[n_] := NestWhileList[l[#] &, n, upQ[#] == False &]
```

$upa$  gives the upward parent  $m \in S_{\geq j}$  of a rightward number  $n = R^k(m) \in S_0$  on a rightward orbit

```
In[50]:= upa[n_] := lll[n] // Last
```

$rpa$  gives the rightward parent  $m \in S_0$  of an upward number  $n = U^j(m) \in S_0$  on an upward orbit

```
In[51]:= rpa[n_] := ddd[n] // Last
```

$sJ[n]$  gives the upwards generation  $j$  of an upward descendant  $n = U^j(m)$  of a rightward ancestor  $m \in S_0$

```
In[52]:= sJ[n_] := Length[ddd[n]] - 1
```

$s0K[n]$  gives the rightward generation  $k$  of an rightward descendant  $n = R_0^k(m)$  of an upward ancestor  $m \in S_{\geq j}$

```
In[53]:= s0K[n_] := If[r[n] ≠ n, Length[l1l[n]] - 1, 0]
```

Auxiliary function  $rexp[n]$  and  $lexp[n]$  gives the power of 2 to which  $n$  is raised in  $r[n]$ , respectively  $l[n]$

$upjQ$  questions whehter one's ancestor is upward of the  $>j$ 'th degree ( $ddd$  includes the rightward parent, reduces to more than  $j$  upward ancestors) (+1 in the function ensures that the last number in  $ddd[n]$  is the rightward ancestor of  $n$ )

```
In[54]:= upjQ[n_, j_] := Length[ddd[n]] > j + 1
```

$rkQ$  questions whehter one's ancestor is rightward of the  $>k$ 'th degree ( $lll$  includes the upward parent, reduces to more than  $k$  leftward ancestors) (+1 in the function ensures that the last number in  $lll[n]$  is the upward ancestor of  $n$ )

```
In[55]:= rkQ[n_, k_] := If[r[n] ≠ n, Length[l1l[n]] > k + 1, False]
```

```
In[56]:=
```

$upjQ$ , first leftwards ( $upjQ$  for trees  $T_j$ )

```
In[57]:= lupjQ[n_, j_] := Length[ddd[l[n]]] > j + 1
```

```
In[58]:= ltjQ[n_, j_] := Length[sJ[n]] < j
```

```
In[59]:= rexp[n_] := Switch[Mod[n, 54],
```

```
4, 2,
16, 3,
22, 4,
34, 1,
40, 2,
52, 1,
_, 0];
```

```
In[60]:= lexp[n_] := Which[MemberQ[{16, 88, 160, 232, 256}, Mod[n, 288]], {},
MemberQ[{22, 34, 58, 70, 94, 106, 130, 142, 166, 178, 202, 214, 238, 250, 274, 286}, Mod[n, 288]], 1, MemberQ[
{4, 52, 76, 124, 148, 196, 220, 268}, Mod[n, 288]], 2, MemberQ[{40, 184}, Mod[n, 288]], 3, MemberQ[{112}, Mod[n, 288]], 4] // Expand
```

$rrexp[n, k]$ , respectively  $llexp$ , give the characteristic series of powers of 2 to which  $n$  is raised in the  $k$ 'th rightward, respectively the  $j$ 'th upward iteration.

```
In[61]:= rrexp[n_, k_] := Cases[Drop[rexp[#] & /@ rr[n, k], -1], _Integer]
```

```
In[62]:= llexp[n_, j_] := Cases[Drop[lexp[#] & /@ ll[n, j], -1], _Integer]
```

rrem[n, k] and llem[n, k] give the characteristic series of remainder mod 54, resp mod 288, in the  $k'$  th rightward, respectively the  $k'$ th leftward iteration.

```
In[63]:= rrem[n_, k_] := Cases[Drop[Mod[rr[n, k], 54], -1], _Integer]
```

```
In[64]:= llem[n_, k_] := Cases[Drop[Mod[ll[n, k], 288], -1], _Integer]
```

## Examples of iterated binary tree functions

uu[7,5], rr[7,5] and ll[7,5] give the argument 7 and additionally 5 iterations of upward, rightward and leftward iterations of 7.

```
In[65]:= List[uu[22, 5], rr[22, 5], ll[22, 5]]
```

```
Out[65]= {{22, 88, 1408, 5632, 90112, 360448}, {22, 112, 148, 196, 130, 688}, {22, 34, 52, 40, 16, Null}}
```

```
In[66]:= uu[4, 2]
```

```
Out[66]= {4, 16, 256}
```

The leftward iterative function ll produces Null if further leftward iterates do not exist. The leftward iterative function lll stops iterating after arriving at an upward number; In lll-output with omitted Nulls the last number in row is an upwards number

```
In[67]:= lll[22]
```

```
Out[67]= {22, 34, 52, 40, 16}
```

The downward iterative function ddd stops iterating after arriving at a rightwardnumber; In ddd - output with omitted Nulls the last number in row is a rightward number

```
In[68]:= ddd[16384]
```

```
Out[68]= {16384, 1024, 256, 16, 4}
```

upa gives the upward parent in  $S_j$  of a rightward number  $n \in S_0 \subset \mathbb{N}^R$  on a rightward orbit, and n in case  $n \in \mathbb{N}^U$

```
In[69]:= {upa[22], upa[downtoBranch[3413]]} // TableForm
```

```
Out[69]/TableForm=
```

```
16
```

```
10240
```

rpa gives the rightward parent in  $S_0$  of an upward number  $n \in S_j \subset \mathbb{N}^U$  in the  $j$ 'th generation of upward descendants, and n in case  $n \in \mathbb{N}^R$

```
In[70]:= {rpa[downtoBranch[3413]], rpa[downtoBranch[7]]} // TableForm
```

```
Out[70]/TableForm=
```

```
40
```

```
22
```

$sJ[n]$  gives the upward generation number  $j$  of upward descendants of rightward ancestors in  $S_0$ , which is  $(ddd[n] // \text{Length}) - 1$ .  $sJ$  is important in the context of the reconnection function and its arguments

```
In[71]:= sJ[downtoBranch[5461]]
```

```
Out[71]= 4
```

$rK[n]$  gives the rightward generation number  $k$  of rightward descendants of upward ancestors in  $S_{>0}$ , which is  $(lll[n] // \text{Length}) - 1$ .  $rK$  is important to see the leftward speed at which the reconnection function reconnects upward descendants of  $n$  to a leftwards ancestor  $S_{>j}$ , and ultimately to the upward trunc that holds the binary tree.

```
In[72]:= lll[downtoBranch[27]]
```

```
Out[72]= {124, 94, 142, 214, 322, 484, 364, 274, 412, 310, 466, 700, 526,
          790, 1186, 1780, 1336, 502, 754, 1132, 850, 1276, 958, 1438, 2158, 3238, 4858, 7288}
```

```
In[73]:= s0K[downtoBranch[27]]
```

```
Out[73]= 27
```

$rrem[22]$  and  $llem[22]$  give the rightward, respectively leftward series of powers of 2 that determine rightward iterates, respectively leftward iterates

```
In[74]:= List[rrem[22, 4], llem[22, 4], rr[22, 4], ll[22, 4]] // TableForm
```

```
Out[74]/TableForm=
```

|    |     |     |     |     |
|----|-----|-----|-----|-----|
| 22 | 4   | 40  | 34  |     |
| 22 | 34  | 52  | 40  |     |
| 22 | 112 | 148 | 196 | 130 |
| 22 | 34  | 52  | 40  | 16  |

$rrexp[22]$  and  $llexp[22]$  give the rightward, respectively leftward characteristic powers of 5 iterations of 22;  $rrem[22]$  and  $llem[22]$  give the underlying argument remainders modulo 54



```
In[75]:= List[rrexpr[22, 4], llexpr[22, 4], rrem[22, 4], llem[22, 4]] // TableForm
```

```
Out[75]/TableForm=
```

|    |    |    |    |
|----|----|----|----|
| 4  | 2  | 2  | 1  |
| 1  | 1  | 2  | 3  |
| 22 | 4  | 40 | 34 |
| 22 | 34 | 52 | 40 |

## Orbits and root paths

binPath gives the inverse Collatz path for a positive integer  $n$ , restricted to numbers on branching nodes from the congruence classes  $\{4, 16\} \equiv n \pmod{18}$

binPath returns a list of coloured integers - upward Blue, rightward red, non branching number gray - that can be converted back to integers with the auxiliary basic function c2n[n]

```
In[76]:= binPath[n_] := Module[{lst1 = colPath[n], lst2, lst3},
  lst2 = Select[lst1, branchQ[#] &] // Reverse;
  lst3 = MapAt[Style[#, Bold, Darker[Blue]] &, (Style[#, Red] & /@ lst2), Position[(Style[#, Red] & /@ lst2), _?upQ]];
  If[branchQ[n], lst3, Append[lst3, Style[n, Gray]]]
]
```

```
In[77]:= {binPath[27], c2n /@ binPath[27]}
```

```
Out[77]:= {{4, 16, 40, 160, 106, 70, 184, 976, 1300, 1732, 2308, 9232, 6154, 4102, 2734, 1822, 7288, 4858, 3238, 2158, 1438,
  958, 1276, 850, 1132, 754, 502, 1336, 1780, 1186, 790, 526, 700, 466, 310, 412, 274, 364, 484, 322, 214, 142, 94, 124, 27},
  {4, 16, 40, 160, 106, 70, 184, 976, 1300, 1732, 2308, 9232, 6154, 4102, 2734, 1822, 7288, 4858, 3238, 2158, 1438, 958,
  1276, 850, 1132, 754, 502, 1336, 1780, 1186, 790, 526, 700, 466, 310, 412, 274, 364, 484, 322, 214, 142, 94, 124, 27}}
```

bbinPath[n] gives the binary root path of a number, starting with an upward iteration

```
In[78]:= bbinPath[n_] := If[upQ[#], 1, 0] & /@ c2n /@ binPath[downtoBranch[n]] // Rest
```

```
In[79]:= bbinPath[27]
```

```
Out[79]:= {1, 0, 1, 0, 0, 0, 0, 0, 0, 0, 1, 0, 0, 0, 0, 1, 0, 0, 0, 0, 0, 0, 0, 0, 0, 0, 0, 0, 0, 0, 0, 0, 0, 0, 0, 0, 0, 0, 0, 0, 0}
```

rootP[n] gives number of alternating upward and rightward iterations, starting with upward iterations

```
In[80]:= rootP[n_] := Partition[Length /@ Split[bbinPath[downtoBranch[n]]], UpTo[2]]
```

```
In[81]:= rootP[27]
```

```
Out[81]:= {{1, 1}, {1, 7}, {1, 4}, {1, 27}}
```

The number of different numbers that can be reached in the number of binary splits required to reach 27 is about  $1.76 \times 10^{13}$

```
In[82]:= 2^Length[binPath[downtoBranch[27]]] // N
```

```
Out[82]:= 1.75922 × 1013
```

The length of root paths in different trees (Collatz original, Syracuse, Collatz binary, upward & rightward orbits Collatz binary) of 27

```
In[83]:= Length /@ {colPath[27], syrPath[27], binPath[27], rootP[27] // Flatten}
```

```
Out[83]:= {112, 1, 45, 8}
```

## Finding least common multiple output congruence classes

TableU derives the argument periodicity (=6) and output periodicity (=96) of the **Upward** function  $u[n]$ , using FindInstance as minimization function:

$a \in aVec$ : {1,5} two admissible residue classes modulo 6 in  $S_{\geq 0}$

$p(a) \in puVec$ : {2,4} derived as the minimum power of  $p$  for which  $(3a + 1) 2^p - 1 \equiv rn$ ,

starting from  $a$ 's already pruned even parent  $3a+1$ ,

with as constraints that  $a$  and  $rn$  are admissible numbers

$u[n]|a \in fu$ : {4n+1,16n+5} the upward function  $u[n]$  given  $a$  (**definition 1**)

$\mathbb{N}^U \in nU$ : {{5,29,53,77},{85}} the upward output modulo 96 given  $a=\{1,5\}$  (**lemma 1**)

Cardinality per period of 96 gives density  $\rho(\mathbb{N}^U)=5/96$  (**lemma 3a**)

(Notes on TableU-code:

- instead of the Mathematica function ArgMin[], FindInstance[] is used to specify minimization constraints;

- instead of the derived function  $u[n]|a \in fu$ ,  $u[n_+]$  above based on it, is used to derive rightward output periodicity)

uargmin and argmin can be used to give a table with output values of the upward function applied to  $n=6i+a$ , respectively of the rightward function applied to  $n=18i+a$  for residue classes  $a$  (not divisible by 2 or 3) in its rows, and values of  $p$  up to 4 in its columns. The last term involving  $i$  shows the periodicity, the first term indicates whether  $p$  is the minimum argument: not a fraction and not divisible by 2 and/or 3.

```
In[84]:= uargp[n_] := Table[2^p n, {p, 1, 4}] // Expand;
```

```
Prepend[Table[{a, uargp[18 i + a]} // Flatten, {a, {4, 16}}], {"n=18i+a", "p=1", "p=2", "p=3", "p=4"}] // TableForm
```

```
Out[85]//TableForm=
```

| $n=18i+a$ | $p=1$       | $p=2$       | $p=3$         | $p=4$         |
|-----------|-------------|-------------|---------------|---------------|
| 4         | $8 + 36 i$  | $16 + 72 i$ | $32 + 144 i$  | $64 + 288 i$  |
| 16        | $32 + 36 i$ | $64 + 72 i$ | $128 + 144 i$ | $256 + 288 i$ |

```
In[86]:= rargp[n_] := Table[2^p (n - 1) / 3, {p, 1, 4}] // Expand;
Prepend[Table[{a, rargp[54 i + a]} // Flatten, {a, {4, 16, 22, 34, 40, 52}}], {"n=54i+a", "p=1", "p=2", "p=3", "p=4"}] // TableForm
```

Out[86]/TableForm=

| $n=54i+a$ | $p=1$       | $p=2$       | $p=3$         | $p=4$         |
|-----------|-------------|-------------|---------------|---------------|
| 4         | $2 + 36 i$  | $4 + 72 i$  | $8 + 144 i$   | $16 + 288 i$  |
| 16        | $10 + 36 i$ | $20 + 72 i$ | $40 + 144 i$  | $80 + 288 i$  |
| 22        | $14 + 36 i$ | $28 + 72 i$ | $56 + 144 i$  | $112 + 288 i$ |
| 34        | $22 + 36 i$ | $44 + 72 i$ | $88 + 144 i$  | $176 + 288 i$ |
| 40        | $26 + 36 i$ | $52 + 72 i$ | $104 + 144 i$ | $208 + 288 i$ |
| 52        | $34 + 36 i$ | $68 + 72 i$ | $136 + 144 i$ | $272 + 288 i$ |

```
In[87]:= TableU4 = Module[{aVec, puVec, argumentsU, a, p, rn, fu, nUp},
  aVec = {1, 5};
  argumentsU = (Table[18 i + (3 # + 1), {i, 0, 4}] & /@ aVec);
  puVec = Last /@ First /@ First /@ Table[
    FindInstance[
      ((3 a + 1) 2^p - 1) / 3 == rn &&
      p ∈ Integers && p > 0 && p < 5 &&
      rn ∈ Integers && Not[rn / 3 ∈ Integers],
      {p, rn}],
    {a, aVec}];
  fu = Simplify[((3 n + 1) 2^n - 1) / 3 & /@ puVec];
  nUp = Union[#] & /@ (Table[u[18 i + j] // m288, {i, 0, 3}, {j, {4, 16}}] // Transpose);
  alignU = Length /@ nUp;
  Prepend[{3 aVec + 1, argumentsU, puVec, Last /@ fu, alignU, nUp} // Transpose,
    {"a", "S_{≥0} argumentsU mod 18", "p(a)", "u[n]", "h_u", "S_{≥1} outputU mod 288"}] // MatrixForm
```

Out[87]/MatrixForm=

$$\begin{pmatrix} a & S_{\geq 0} \text{ argumentsU mod 18} & p(a) & u[n] & h_u & S_{\geq 1} \text{ outputU mod 288} \\ 4 & \{4, 22, 40, 58, 76\} & 2 & 4n & 4 & \{16, 88, 160, 232\} \\ 16 & \{16, 34, 52, 70, 88\} & 4 & 16n & 1 & \{256\} \end{pmatrix}$$

TableR derives the argument periodicity (=18) and output periodicity (=96) of the **Rightward** function  $r[n]$ , using FindInstance as minimization function:

$a \in aVec$ : {1,5,7,11,13,17} six admissible residue classes modulo 18 in  $S_{\geq 0}$

$p(a) \in prVec$ : {2,3,4,1,2,1} derived as the minimum power of  $p$  for which  $((3a + 1) 2^p - 1) / 3 = rn$ ,  
starting from  $a$  itself

(rather than from  $a$ 's pruned even parent  $3a+1$  as in the upward function),  
with as constraints that  $a$  and  $m$  are admissible numbers

$r[n]|a \in \text{fr}$ :  $\{-\frac{1}{3} + \frac{4n}{3}, \dots, -\frac{1}{3} + \frac{2n}{3}\}$  the upward function  $u[n]$  given  $a$  (**definition 2**)

$m(a)$   $\{24, \dots, 12\}$  six intrinsic moduli of the rightward function for  $a \in \text{aVec}$

$h(a)$   $\{4, 2, 1, 8, 4, 8\}$  heap vector, gives rightward output cardinality per output period 96  
sum heap vector equals density  $\rho(\mathbb{N}^R) = 27/96$

$\mathbb{N}^R \in nR$ :  $\{\{1, 25, \dots\}, \dots, \{\dots, 83, 9\}\}$  the rightward output modulo 96 given  $a = \{1, 5, \dots, 17\}$  (**lemma 2**)

Cardinality per period of 96 gives density  $\rho(\mathbb{N}^R) = 27/96$  (**lemma 3b**)

For  $j = \{0, 1, 2\}$ :  $R[54i + 18j + a] \bmod 18 : 3$  congruences classes modulo 18 rightward iteration  $k$   
given congruence classes  $a \in \text{aVec}$  at iteration  $k-1$

$T$  transformation matrix, indicator matrix whether specific congruence class is output

(Notes on TableR-code:

- instead of the Mathematica function `ArgMin[]`, `FindInstance[]` is used to specify minimization constraints;
- instead of the derived function  $r[n|a] \in \text{fr}$ ,  $r[n\_]$  above based on it, is used to derive rightward output periodicity)

```

In[88]:= TableR = Module[
  {aVec = {4, 16, 22, 34, 40, 52},
   argumentsR, prVec, a, p, rn, fr, maVec, heapVec, nR, nr18, transf},
  argumentsR = 54 # + aVec & /@ {0, 1, 2, 3, 4, 5} // Transpose;
  prVec = Last /@ First /@ First /@ Table[
    FindInstance[
      2^p (a - 1) / 3 == rn &&
      p ∈ Integers && p > 0 && p < 5 &&
      rn ∈ Integers && (rn - 1) / 3 ∈ Integers && Not[(rn - 1) / 9 ∈ Integers],
      {p, rn}],
    {a, {4, 16, 22, 34, 40, 52}}];
  fr = Distribute[2^# ((n - 1) / 3) & /@ prVec] ;
  maVec = 18 × 2^prVec / 3; heapVec = LCM[Sequence @@ maVec] / maVec;
  nR = Table[Table[r[54 (j - 1) + aVec[[i]]], {j, 1, LCM[Sequence @@ maVec] / maVec[[i]]}], {i, 1, 6}];
  nr18 = Table[Table[r[54 j + aVec[[i]]] // m54, {j, 0, 2}], {i, 1, 6}];
  transf = If[Sort[#] == {4, 22, 40}, {1, 0, 1, 0, 1, 0}, {0, 1, 0, 1, 0, 1}] & /@ nr18;
  Prepend[{aVec, argumentsR, prVec, fr, maVec, heapVec, nR, nr18, transf} // Transpose,
    {"a", "S≥0 argumentsR mod 54", "p(a)", "R[n] | a",
     "m(a)", "h(a)", "S0 outputR mod 288", "For j={0,1,2}: R[54i+18j+a] mod 18", "T"}] // MatrixForm]

```

Out[88]//MatrixForm=

| $a$ | $S_{\geq 0} \text{ argumentsR mod } 54$ | $p(a)$ | $R[n]   a$           | $m(a)$ | $h(a)$ | $S_0 \text{ outputR mod } 288$         | For $j=\{0,1,2\}: R[54i+18j+a] \text{ mod } 18$ |
|-----|-----------------------------------------|--------|----------------------|--------|--------|----------------------------------------|-------------------------------------------------|
| 4   | {4, 58, 112, 166, 220, 274}             | 2      | $\frac{4}{3}(-1+n)$  | 24     | 4      | {4, 76, 148, 220}                      | {4, 22, 40} {1, 0}                              |
| 16  | {16, 70, 124, 178, 232, 286}            | 3      | $\frac{8}{3}(-1+n)$  | 48     | 2      | {40, 184}                              | {40, 22, 4} {1, 0}                              |
| 22  | {22, 76, 130, 184, 238, 292}            | 4      | $\frac{16}{3}(-1+n)$ | 96     | 1      | {112}                                  | {4, 22, 40} {1, 0}                              |
| 34  | {34, 88, 142, 196, 250, 304}            | 1      | $\frac{2}{3}(-1+n)$  | 12     | 8      | {22, 58, 94, 130, 166, 202, 238, 274}  | {22, 4, 40} {1, 0}                              |
| 40  | {40, 94, 148, 202, 256, 310}            | 2      | $\frac{4}{3}(-1+n)$  | 24     | 4      | {52, 124, 196, 268}                    | {52, 16, 34} {0, 1}                             |
| 52  | {52, 106, 160, 214, 268, 322}           | 1      | $\frac{2}{3}(-1+n)$  | 12     | 8      | {34, 70, 106, 142, 178, 214, 250, 286} | {34, 16, 52} {0, 1}                             |

Figure S3.1 (supplementary materials) shows how upward numbers and rightward numbers cover all branching numbers, due to the alignment vector [4,2,1,8,4,8] for [■, ■, ■, ■, ■, ■].

```

In[89]:= DomainCodomainPlot = Module[{ares, heap, upw96,
  xy1896, yx9618, txy1896, tyx9618,
  tup96a, tup96b, tup96c, tup96d, tup96e,
  tri96a, tri96b},
ares = {4, 16, 22, 34, 40, 52};
heap = {4, 2, 1, 8, 4, 8};
upw96 = {16, 88, 160, 232, 256};
xy1896 = Map[#, r[#]] &, Table[Table[54 i + ares[[a]], {i, 0, heap[[a]] - 1}], {a, 1, 6}], {2}];
yx9618 = Map[{{0, Last[#]}, #] &, xy1896, {2}];
txy1896 = ListPlot[xy1896, Filling -> Axis, FillingStyle -> Directive[Thickness[0.0072]], PlotLegends -> ares,
  Ticks -> {Table[54 i, {i, 0, 11}], Table[18 i, {i, 0, 16}]}, PlotRange -> {{-1, 3 × 144 + 5}, {-35, 3 × 96 + 14}}, AxesLabel -> {"n", "S0"}];
tyx9618 = Table[
  Graphics[{ColorData[97, i], Thickness -> 0.0072, Line[yx9618[[i]]}],
  {i, 1, 6}];
tup96a = Graphics[{PointSize[Large], Blue, Point[Table[{3 × 144 + 4, i}, {i, upw96}]]}];
tup96b = Graphics[{PointSize[Large], Blue, DotDashed, Line[Table[{0, i}, {3 × 144 + 2, i}], {i, upw96}]]];
tup96c = Graphics[{PointSize[Large], Blue, DotDashed, Line[Table[{135, i}, {148, i}], {i, upw96}]]];
tup96d = Graphics[Table[Text[i, {3 × 144 - 36, i}], {i, upw96}]];
tup96e = Graphics[Text["S±1", {3 × 144 - 36, 3 × 96 + 8}]];
tri96a = Graphics[Table[Text[i, {54 i, -27}], {i, {1, 2, 4, 8}}]];
tri96b = Graphics[Text["h=", {6, -27}]];
Show[txy1896, tyx9618, tup96a, tup96b, tup96c, tup96d, tup96e, tri96a, tri96b]]

```

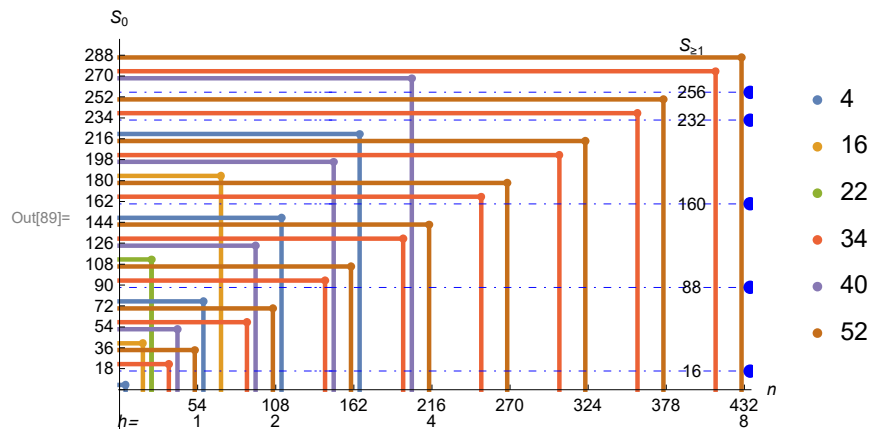

DomainCodomainPlot shows at its y-axis periodic output of the rightward and upward function to one output period 1..96.

The Blue horizontal lines show upward function output to upward numbers  $\{16, 88, 160, 232, 256\} \rightarrow \{\square\}$

The right-angled lines from the x-axis show maps from rightward congruence classes  $\{4,16,22,34,40,52\} \rightarrow \{\text{blue}, \text{orange}, \text{green}, \text{red}, \text{purple}, \text{brown}\}$ .

- $p(a)=1$ , contracting congruence classes  $\{40,52\} \rightarrow \{\text{red}, \text{brown}\}$  with  $h(a)=8$  argument periods of 54 per Least Common Multiple Argument period 3 144=432
- $p(a)=2$ , slowly expanding congruence classes  $\{4,40\} \rightarrow \{\text{blue}, \text{purple}\}$  with  $h(a)=4$  argument periods of 108 per Least Common Multiple Argument period 3 144=432
- $p(a)=3$ , expanding congruence class  $\{16\} \rightarrow \{\text{orange}\}$  with  $h(a)=2$  argument periods covering 216 per Least Common Multiple Argument period 3 144=432
- $p(a)=4$ , fastly expanding congruence class  $\{\}$   $\rightarrow \{\text{green}\}$  with  $h(a)=1$  argument periods covering per Least Common Multiple Argument period 3 144=432

```
In[90]:= TableT = Module[
  {a54 = {4, 16, 22, 34, 40, 52},
    na6, rna6, nr18, transf},
  na6 = 54 # + a54 & /@ {0, 1, 2, 3, 4, 5} // Transpose;
  rna6 = Map[r, na6, {2}];
  nr18 = Table[Table[r[54 j + a54[[i]]] // m54, {j, 0, 2}], {i, 1, 6}];
  transf = If[Sort[#] == {4, 22, 40}, {1, 0, 1, 0, 1, 0}, {0, 1, 0, 1, 0, 1}] & /@ nr18;
  Prepend[{a54, na6, rna6, nr18, transf} // Transpose,
    {"a", "For i={0,1}:For j={0,1,2}: \nn=162i+54j+a",
      "For i={0,1}:For j={0,1,2}: \nR0[162i+54j+a]", "For j={0,1,2}: \nR0[162i+54j+a] mod 54", "T"}]
  //
  MatrixForm]
```

Out[90]//MatrixForm=

|    | For i={0,1}:For j={0,1,2}:<br>$n=162i+54j+a$ | For i={0,1}:For j={0,1,2}:<br>$R_0[162i+54j+a]$ | For j={0,1,2}:<br>$R_0[162i+54j+a] \bmod 54$ | T                  |
|----|----------------------------------------------|-------------------------------------------------|----------------------------------------------|--------------------|
| 4  | {4, 58, 112, 166, 220, 274}                  | {4, 76, 148, 220, 292, 364}                     | {4, 22, 40}                                  | {1, 0, 1, 0, 1, 0} |
| 16 | {16, 70, 124, 178, 232, 286}                 | {40, 184, 328, 472, 616, 760}                   | {40, 22, 4}                                  | {1, 0, 1, 0, 1, 0} |
| 22 | {22, 76, 130, 184, 238, 292}                 | {112, 400, 688, 976, 1264, 1552}                | {4, 22, 40}                                  | {1, 0, 1, 0, 1, 0} |
| 34 | {34, 88, 142, 196, 250, 304}                 | {22, 58, 94, 130, 166, 202}                     | {22, 4, 40}                                  | {1, 0, 1, 0, 1, 0} |
| 40 | {40, 94, 148, 202, 256, 310}                 | {52, 124, 196, 268, 340, 412}                   | {52, 16, 34}                                 | {0, 1, 0, 1, 0, 1} |
| 52 | {52, 106, 160, 214, 268, 322}                | {34, 70, 106, 142, 178, 214}                    | {34, 16, 52}                                 | {0, 1, 0, 1, 0, 1} |

## 4.The Collatz clock

Congruence classes  $C5$  and  $c27$  and alignment vectors tree  $T_{\geq 0}$

The functions below generate the congruence classes that are used in Figure 6 of the main text (commutative diagram Collatz clock).

Some of them are listed in Section S2 of the Supplementary Materials. The notation of sets of congruence classes is explained in the main text.

$\text{perUo}[i]$ ,  $\text{perUe}[j]$ , and  $\text{PerR}[k]$  are the periodicities of the  $i$ 'th,  $j$ 'th, resp.  $k$ 'th iteration of the upward function for odd iterations, the upward function for even iterations, and the rightward function (regardless whether the iteration is odd or even).

```
In[91]:= perUj[j_] := 288 × 2^(3 j);
perUi[i_] := 4608 × 2^(3 (i - 1));
perR[k_] := 4608 × 2^(4 (k - 1));
perR2[k_] := 13824 × 2^(4 (k - 1));
```

$\text{brLst}[\text{maxLst}]$  gives branching nodes until a  $\text{maxLst}$ -periodicity

```
In[92]:= brLst[period_] := Module[{nk = period / 18}, Table[{18 i + 4, 18 i + 16}, {i, 0, nk - 1}] // Flatten // Sort]
```

$\text{splitMod}[\text{period}, \text{mod}]$  splits a period into subperiods modulo  $\text{mod}$

```
In[93]:= splitMod[period_, mod_] := Map[Last[#] &,
SortBy[
  (GatherBy[{Mod[#, mod], #} & /@ period, First]),
  {First, Last}], {2}]
```

$\text{uh}[n, \text{period}]$  and  $\text{rh}[n, \text{period}]$  apply the upward, resp. rightward, function to assign  $n$  to ascending congruence classes modulo  $\text{period}$ ;

$\text{C5mod18}$  and  $\text{c27mod54}$  are 5 upward, resp 27 rightward, congruence classes modulo 288 of the basic tree  $T_{\geq 0} = t_{\geq 0}$  split up by ascending congruence classes modulo 18, respectively 54

```
In[94]:= uh[n_, period_] := Module[{m = m18[n]}, Switch[m,
  4, u /@ Table[i period + n, {i, 0, 3}],
  16, u /@ Table[i period + n, {i, 0, 0}]]];
C5mod18 = uh[#, 18] & /@ {4, 16};
Grid[C5mod18, Alignment → Left]
```

```
16  88 160 232
Out[96]= 256
```



```

In[97]:= rh[n_, period_] := Module[{m = m54[n]}, Switch[m,
  4, r /@ Table[i period + n, {i, 0, 3}],
  16, r /@ Table[i period + n, {i, 0, 1}],
  22, r /@ Table[i period + n, {i, 0, 0}],
  34, r /@ Table[i period + n, {i, 0, 7}],
  40, r /@ Table[i period + n, {i, 0, 3}],
  52, r /@ Table[i period + n, {i, 0, 7}]]];
c27mod54 = rh[#, 54] & /@ {4, 16, 22, 34, 40, 52};
Grid[c27mod54, Alignment → Left]

```

```

4   76  148  220
40  184
112
Out[99]= 22  58  94  130  166  202  238  274
52  124  196  268
34   70  106  142  178  214  250  286

```

C5 and c27 are 5 upward, resp 27 rightward, congruence classes modulo 288 of the basic tree  $T_{\geq 0} = t_{\geq 0}$   
(definitons 1 and 2 main text)

```

In[100]:= C5 = C5mod18 // Flatten // Sort;
c27 = c27mod54 // Flatten // Sort;
Grid[{C5, c27}, Alignment → Left]

```

```

16  88  160  232  256
Out[102]= 4   22  34   40   52   58  70  76  94  106  112  124  130  142  148  166  178  184  196  202  214  220  238  250  268  274  286

```

alignU and alignR represent the upward and rightward alignment vectors (assuming their least possible congruence classes modulo 18, respectively 54)

```

In[103]:= alignU = Length /@ C5mod18 ;
alignR = Length /@ c27mod54;
Grid[{alignU, alignR}]

```

```

4   1
Out[105]= 4   2   1   8   4   8

```

c15 is labeled 3c5 in the main test, represents 15 upward congruence classes modulo in a three times larger period  $3 \cdot 288 = 864$ , split up by rightward argument classes m54. They are the arguments to generate the disjoint rightward trees  $t_k$ .

```

In[106]:= C15 = splitMod[
  Select[
    brLst[3 × 288],
    upQ[#] &],
  54]

Out[106]= {{544}, {16, 232, 448, 664}, {832}, {88, 304, 520, 736}, {256}, {160, 376, 592, 808}}

In[107]:= C15 = {16, 88, 160, 232, 256, 304, 376, 448, 520, 544, 592, 664, 736, 808, 832}
Out[107]= {16, 88, 160, 232, 256, 304, 376, 448, 520, 544, 592, 664, 736, 808, 832}

In[108]:= splitMod[C8, 18]
Out[108]= GatherBy[C8, First]

```

## Congruence classes and periodicities of, nested and disjoint, upward subtrees

$C5j[j]$  gives the  $5^{3j}$  congruence classes of the even nested tree  $T_{\geq j}$ ,

$m5j[j]$  gives their modular periodicity

```

In[109]:= C5j[j_] := 23j # & /@ C5;
m5j[j_] := 23j × 288;
Grid[
  Prepend[
    ReplacePart[
      Table[{j, C5j[j], m5j[j], m5j[j] // factorInteger}, {j, 0, 10, 2}],
      {1, 1} → "0: upward C5",
      {"T≥j upward nested", "5 congruence classes", "modular periodicity"}],
    Dividers → {False, {True, True}}, Alignment → Left]

```

|           | $T_{\geq j}$ upward nested | 5 congruence classes                                                 | modular periodicity |              |
|-----------|----------------------------|----------------------------------------------------------------------|---------------------|--------------|
|           | 0: upward C5               | {16, 88, 160, 232, 256}                                              | 288                 | $2^5 3^2$    |
|           | 2                          | {1024, 5632, 10240, 14848, 16384}                                    | 18432               | $2^{11} 3^2$ |
| Out[111]= | 4                          | {65536, 360448, 655360, 950272, 1048576}                             | 1179648             | $2^{17} 3^2$ |
|           | 6                          | {4194304, 23068672, 41943040, 60817408, 67108864}                    | 75497472            | $2^{23} 3^2$ |
|           | 8                          | {268435456, 1476395008, 2684354560, 3892314112, 4294967296}          | 4831838208          | $2^{29} 3^2$ |
|           | 10                         | {17179869184, 94489280512, 171798691840, 249108103168, 274877906944} | 309237645312        | $2^{35} 3^2$ |

```

In[112]:= C27j[j_] := 23j # & /@ c27;
Grid[
  Prepend[
    ReplacePart[
      Table[{j, C27j[j], m5j[j], m5j[j] // factorInteger}, {j, 0, 10, 2}],
      {1, 1} → "0: rightward c27",
      {"Tj upward disjoint", "27 congruence classes", "modular periodicity"}],
    Dividers → {False, {True, True}}, Alignment → Left]

```

|  | $T_j$ upward disjoint | 27 congruence classes                                                                                                                                                                                                                                                                                                                                                             | modular periodicity |              |
|--|-----------------------|-----------------------------------------------------------------------------------------------------------------------------------------------------------------------------------------------------------------------------------------------------------------------------------------------------------------------------------------------------------------------------------|---------------------|--------------|
|  | 0: rightward c27      | {4, 22, 34, 40, 52, 58, 70, 76, 94, 106, 112, 124, 130, 142, 148, 166, 178, 184, 196, 202, 214, 220, 238, 250, 268, 274, 286}                                                                                                                                                                                                                                                     | 288                 | $2^5 3^2$    |
|  | 2                     | {256, 1408, 2176, 2560, 3328, 3712, 4480, 4864, 6016, 6784, 7168, 7936, 8320, 9088, 9472, 10624, 11392, 11776, 12544, 12928, 13696, 14080, 15232, 16000, 17152, 17536, 18304}                                                                                                                                                                                                     | 18 432              | $2^{11} 3^2$ |
|  | 4                     | {16384, 90112, 139264, 163840, 212992, 237568, 286720, 311296, 385024, 434176, 458752, 507904, 532480, 581632, 606208, 679936, 729088, 753664, 802816, 827392, 876544, 901120, 974848, 1024000, 1097728, 1122304, 1171456}                                                                                                                                                        | 1 179 648           | $2^{17} 3^2$ |
|  | 6                     | {1048576, 5767168, 8912896, 10485760, 13631488, 15204352, 18350080, 19922944, 24641536, 27787264, 29360128, 32505856, 34078720, 37224448, 38797312, 43515904, 46661632, 48234496, 51380224, 52953088, 56098816, 57671680, 62390272, 65536000, 70254592, 71827456, 74973184}                                                                                                       | 75 497 472          | $2^{23} 3^2$ |
|  | 8                     | {67108864, 369098752, 570425344, 671088640, 872415232, 973078528, 1174405120, 1275068416, 1577058304, 1778384896, 1879048192, 2080374784, 2181038080, 2382364672, 2483027968, 2785017856, 2986344448, 3087007744, 3288334336, 3388997632, 3590324224, 3690987520, 3992977408, 4194304000, 4496293888, 4596957184, 4798283776}                                                     | 4 831 838 208       | $2^{29} 3^2$ |
|  | 10                    | {4294967296, 23622320128, 36507222016, 42949672960, 55834574848, 62277025792, 75161927680, 81604378624, 100931731456, 113816633344, 120259084288, 133143986176, 139586437120, 152471339008, 158913789952, 178241142784, 191126044672, 197568495616, 210453397504, 216895848448, 229780750336, 236223201280, 255550554112, 268435456000, 287762808832, 294205259776, 307090161664} | 309 237 645 312     | $2^{35} 3^2$ |

C8 eight upward congruence classes modulo 4608 of the basic odd nested tree  $T_{\geq 1} = t_0$

```

In[114]:= C8 = uh[#, 288] & /@ C5 // Flatten // Sort
Out[114]= {256, 1024, 1408, 2176, 2560, 3328, 3712, 4480}

```

$C8[i]$  gives the  $5^{3(i-1)}$  congruence classes of the even nested tree  $T_{\geq j}$

```
In[115]:= C8i[i_] := 23(i-1) # & /@ C8;
m8i[i_] := 23(i-1) × 4608;
Grid[
  Prepend[
    ReplacePart[
      Table[{i, splitMod[C8i[i], 18], m8i[i], m8i[i] // factorInteger}, {i, 1, 9, 2}],
      {1, 1} → "1: upward C8",
      {"T≥i upward nested", "8 congruence classes", "modular periodicity"}],
    Dividers → {False, {True, True}}, Alignment → Left]
```

|              | $T_{\geq i}$ upward nested 8 congruence classes                                                                         | modular periodicity |              |
|--------------|-------------------------------------------------------------------------------------------------------------------------|---------------------|--------------|
| 1: upward C8 | $\{\{256, 1408, 2560, 3712\}, \{1024, 2176, 3328, 4480\}\}$                                                             | 4608                | $2^9 3^2$    |
| 3            | $\{\{16384, 90112, 163840, 237568\}, \{65536, 139264, 212992, 286720\}\}$                                               | 294912              | $2^{15} 3^2$ |
| 5            | $\{\{1048576, 5767168, 10485760, 15204352\}, \{4194304, 8912896, 13631488, 18350080\}\}$                                | 18874368            | $2^{21} 3^2$ |
| 7            | $\{\{67108864, 369098752, 671088640, 973078528\},$<br>$\{268435456, 570425344, 872415232, 1174405120\}\}$               | 1207959552          | $2^{27} 3^2$ |
| 9            | $\{\{4294967296, 23622320128, 42949672960, 62277025792\},$<br>$\{17179869184, 3650722016, 55834574848, 75161927680\}\}$ | 77309411328         | $2^{33} 3^2$ |

$C72$  72 upward congruence classes modulo 288 in the disjoint upward tree  $T_1$

```
In[118]:= C72 = uh[#, 288] & /@ c27 // Flatten // Sort
Out[118]:= {16, 88, 160, 232, 304, 376, 448, 520, 544, 592, 664, 736, 808, 832, 880, 952, 1096, 1120, 1168, 1240, 1312, 1384, 1456, 1528, 1600, 1672, 1696,
1744, 1816, 1888, 1960, 1984, 2032, 2104, 2248, 2272, 2320, 2392, 2464, 2536, 2608, 2680, 2752, 2824, 2848, 2896, 2968, 3040, 3112, 3136,
3184, 3256, 3400, 3424, 3472, 3544, 3616, 3688, 3760, 3832, 3904, 3976, 4000, 4048, 4120, 4192, 4264, 4288, 4336, 4408, 4552, 4576}
```

```
In[119]:=
```

```
In[120]:= C72i[i_] := 23 (i-1) # & /@ C72;
```

```
Grid[
```

```
  Prepend[
```

```
    ReplacePart[
```

```
      Table[{i, splitMod[C72i[i], 18], m8i[i], m8i[i] // factorInteger}, {i, 1, 9, 2}],
```

```
      {1, 1} → "1: upward C72"],
```

```
      {"Ti upward disjoint", "72 congruence classes", "modular periodicity"}],
```

```
    Dividers → {False, {True, True}}, Alignment → Left]
```

| $T_i$ upward disjoint 72 congruence classes |                                                                                                                                                                                                                                                                                                                                                                                                                                                                                                                                                                                                                                                                                                                                  | modular periodicity |              |
|---------------------------------------------|----------------------------------------------------------------------------------------------------------------------------------------------------------------------------------------------------------------------------------------------------------------------------------------------------------------------------------------------------------------------------------------------------------------------------------------------------------------------------------------------------------------------------------------------------------------------------------------------------------------------------------------------------------------------------------------------------------------------------------|---------------------|--------------|
| 1: upward C72                               | {544, 832, 1120, 1696, 1984, 2272, 2848, 3136, 3424, 4000, 4288, 4576},<br>{16, 88, 160, 232, 304, 376, 448, 520, 592, 664, 736, 808, 880, 952, 1096, 1168, 1240, 1312,<br>1384, 1456, 1528, 1600, 1672, 1744, 1816, 1888, 1960, 2032, 2104, 2248, 2320, 2392,<br>2464, 2536, 2608, 2680, 2752, 2824, 2896, 2968, 3040, 3112, 3184, 3256, 3400, 3472,<br>3544, 3616, 3688, 3760, 3832, 3904, 3976, 4048, 4120, 4192, 4264, 4336, 4408, 4552}}                                                                                                                                                                                                                                                                                    | 4608                | $2^9 3^2$    |
| 3                                           | {34816, 53248, 71680, 108544, 126976,<br>145408, 182272, 200704, 219136, 256000, 274432, 292864},<br>{1024, 5632, 10240, 14848, 19456, 24064, 28672, 33280, 37888, 42496, 47104, 51712, 56320,<br>60928, 70144, 74752, 79360, 83968, 88576, 93184, 97792, 102400, 107008, 111616,<br>116224, 120832, 125440, 130048, 134656, 143872, 148480, 153088, 157696,<br>162304, 166912, 171520, 176128, 180736, 185344, 189952, 194560, 199168,<br>203776, 208384, 217600, 222208, 226816, 231424, 236032, 240640, 245248,<br>249856, 254464, 259072, 263680, 268288, 272896, 277504, 282112, 291328}}                                                                                                                                   | 294912              | $2^{15} 3^2$ |
| 5                                           | {2228224, 3407872, 4587520, 6946816, 8126464, 9306112,<br>11665408, 12845056, 14024704, 16384000, 17563648, 18743296},<br>{65536, 360448, 655360, 950272, 1245184, 1540096, 1835008, 2129920, 2424832,<br>2719744, 3014656, 3309568, 3604480, 3899392, 4489216, 4784128, 5079040, 5373952,<br>5668864, 5963776, 6258688, 6553600, 6848512, 7143424, 7438336, 7733248, 8028160,<br>8323072, 8617984, 9207808, 9502720, 9797632, 10092544, 10387456, 10682368, 10977280,<br>11272192, 11567104, 11862016, 12156928, 12451840, 12746752, 13041664, 13336576,<br>13926400, 14221312, 14516224, 14811136, 15106048, 15400960, 15695872, 15990784,<br>16285696, 16580608, 16875520, 17170432, 17465344, 17760256, 18055168, 18644992}} | 18874368            | $2^{21} 3^2$ |

```
Out[121]=
```

|   |                                                                                                                                                                                                                                                                                                                                                                                                                                                                                                                                                                                                                                                                                                                                                                                                                                                                                                                                                                                                      |                |              |
|---|------------------------------------------------------------------------------------------------------------------------------------------------------------------------------------------------------------------------------------------------------------------------------------------------------------------------------------------------------------------------------------------------------------------------------------------------------------------------------------------------------------------------------------------------------------------------------------------------------------------------------------------------------------------------------------------------------------------------------------------------------------------------------------------------------------------------------------------------------------------------------------------------------------------------------------------------------------------------------------------------------|----------------|--------------|
| 7 | { {142606336, 218103808, 293601280, 444596224, 520093696, 595591168,<br>746586112, 822083584, 897581056, 1048576000, 1124073472, 1199570944},<br>{4194304, 23068672, 41943040, 60817408, 79691776, 98566144, 117440512, 136314880,<br>155189248, 174063616, 192937984, 211812352, 230686720, 249561088, 287309824, 306184192,<br>325058560, 343932928, 362807296, 381681664, 400556032, 419430400, 438304768, 457179136,<br>476053504, 494927872, 513802240, 532676608, 551550976, 589299712, 608174080, 627048448,<br>645922816, 664797184, 683671552, 702545920, 721420288, 740294656, 759169024,<br>778043392, 796917760, 815792128, 834666496, 853540864, 891289600, 910163968,<br>929038336, 947912704, 966787072, 985661440, 1004535808, 1023410176, 1042284544,<br>1061158912, 1080033280, 1098907648, 1117782016, 1136656384, 1155530752, 1193279488} }                                                                                                                                      | 1 207 959 552  | $2^{27} 3^2$ |
| 9 | { {9126805504, 13958643712, 18790481920, 28454158336, 33285996544, 38117834752,<br>47781511168, 52613349376, 57445187584, 67108864000, 71940702208, 76772540416},<br>{268435456, 1476395008, 2684354560, 3892314112, 5100273664, 6308233216,<br>7516192768, 8724152320, 9932111872, 11140071424, 12348030976, 13555990528,<br>14763950080, 15971909632, 18387828736, 19595788288, 20803747840, 22011707392,<br>23219666944, 24427626496, 25635586048, 26843545600, 28051505152, 29259464704,<br>30467424256, 31675383808, 32883343360, 34091302912, 35299262464, 37715181568,<br>38923141120, 40131100672, 41339060224, 42547019776, 43754979328, 44962938880,<br>46170898432, 47378857984, 48586817536, 49794777088, 51002736640, 52210696192,<br>53418655744, 54626615296, 57042534400, 58250493952, 59458453504, 60666413056,<br>61874372608, 63082332160, 64290291712, 65498251264, 66706210816, 67914170368,<br>69122129920, 70330089472, 71538049024, 72746008576, 73953968128, 76369887232} } | 77 309 411 328 | $2^{33} 3^2$ |

## Congruence classes and periodicities of, nested and disjoint, rightward, subtrees

lstMt[lst,mod,times] aligns a list based on periodicity 'mod' 'times' times, e.g. {1,2},3,2 with a list of length 2 would deliver this list with length 1,2,3+1,3+2 four.

```
In[122]:= lstMt[lst_, mod_, times_] := Table[i mod + #, {i, 0, times - 1}] & /@ lst // Flatten // Sort
```

alignright[k,lst] assumes the congruence classes for the k'th rightward iteration;

returns the congruence classes for the k+1 th iteration

```

In[123]:= alignRight[{k_, lst1_}] := Module[
  {per =  $288 \times 2^{4k}$ , lst2, lst3},
  lst2 = splitMod[lstMt[lst1, per, 3], 54];
  lst3 = r /@
    ({lstMt[lst2[[1]], 3 per, 4],
     lstMt[lst2[[2]], 3 per, 2],
     lst2[[3]],
     lstMt[lst2[[4]], 3 per, 8],
     lstMt[lst2[[5]], 3 per, 4],
     lstMt[lst2[[6]], 3 per, 8]} // Flatten) // Sort;
  {k + 1, Map[Last, GatherBy[{m54[#], #} & /@ lst3 // Sort, First], {2}]}]

```

$c432[k]$ ,  $c81[k]$  and  $c351[k]$  give congruence classes for the  $k$ 'th rightward iteration of respectively  
 nested trees  $t_{\geq k}$  with  $(432 = 81 + 351) 13^{k-1}$  congruence classes,  
 disjoint trees  $t_k$  with  $81 \times 13^{k-1}$  congruence classes  
 and rightward iterations on rightward numbers with  $351 \times 13^{k-1}$  congruence classes.

```

In[124]:= c432k[nk_] := NestList[alignRight, {0, {C5, c27} // Flatten}, nk];
c81k[nk_] := NestList[alignRight, {0, C5}, nk];
c351k[nk_] := NestList[alignRight, {0, c27}, nk];

```

In[127]:= **intermezzo check set sizes congruence classes rightward congruence classes**

Out[127]= check classes<sup>2</sup> congruence<sup>2</sup> intermezzo rightward set sizes

```

In[128]:= alignR

```

Out[128]= {4, 2, 1, 8, 4, 8}

```

In[129]:= transR = {{1, 0, 1, 0, 1, 0}, {1, 0, 1, 0, 1, 0}, {1, 0, 1, 0, 1, 0}, {1, 0, 1, 0, 1, 0}, {0, 1, 0, 1, 0, 1}, {0, 1, 0, 1, 0, 1}}

```

```

Out[129]= {{1, 0, 1, 0, 1, 0}, {1, 0, 1, 0, 1, 0}, {1, 0, 1, 0, 1, 0}, {1, 0, 1, 0, 1, 0}, {0, 1, 0, 1, 0, 1}, {0, 1, 0, 1, 0, 1}}

```

```

In[130]:= nright3[k_] := NestList[Dot[# alignR, transR] &, {1, 4, 1, 4, 1, 4}, k]

```

```

In[131]:= nright[knright3_] := Map[factorInteger, Rest[nright3[knright3]] / 3, {2}] // Grid

```



In[132]:= **nright[3]**

Out[132]= 
$$\begin{array}{cccccc} 3^1 5^1 & 2^2 3^1 & 3^1 5^1 & 2^2 3^1 & 3^1 5^1 & 2^2 3^1 \\ 3^1 5^1 13^1 & 2^2 3^1 13^1 & 3^1 5^1 13^1 & 2^2 3^1 13^1 & 3^1 5^1 13^1 & 2^2 3^1 13^1 \\ 3^1 5^1 13^2 & 2^2 3^1 13^2 & 3^1 5^1 13^2 & 2^2 3^1 13^2 & 3^1 5^1 13^2 & 2^2 3^1 13^2 \end{array}$$

## end check

cNk[func\_,nk\_] can be applied to the three rightward functions above for k=1..nk iterations, with as output iterator k, congruence classes, factorInteger of cardinality, factorInteger of periodicity

In[133]:= **cNk[func\_, nk\_] :=**

**{First[#], Last[#], factorInteger[Length[Last[#] // Flatten]], 288 × 2<sup>4 First[#]</sup>, factorInteger[288 × 2<sup>4 First[#]</sup>]} & /@ func[nk]**

The grid for c81k is printed for k= 0 (upward congruence classes C5) only, the first iteration with c81 = 3<sup>4</sup> 13<sup>0</sup> congruence classes, and the second iteration with 81 13=27 13<sup>2</sup> iterations because it is just the combination of c81k and c351k.

In[134]:= **Grid[**

**Prepend[**  
**ReplacePart[cNk[c81k, 2], {{1, 1} → "0: upward C5", {2, 1} → "1: rightward c81"}],**  
**{"t<sub>k</sub> right disjoint", "81·13<sup>k-1</sup> congruence classes", "cardinality", "periodicity"}],**  
**Dividers → {False, {True, True}}, Alignment → Left]**

| $t_k$ right disjoint | $81 \cdot 13^{k-1}$ congruence classes                                                                                                                                                                                                                                                                                                                                                                                                                                                                          | cardinality                    | periodicity |                                |
|----------------------|-----------------------------------------------------------------------------------------------------------------------------------------------------------------------------------------------------------------------------------------------------------------------------------------------------------------------------------------------------------------------------------------------------------------------------------------------------------------------------------------------------------------|--------------------------------|-------------|--------------------------------|
| 0: upward C5         | {16, 88, 160, 232, 256}                                                                                                                                                                                                                                                                                                                                                                                                                                                                                         | 5 <sup>1</sup>                 | 288         | 2 <sup>5</sup> 3 <sup>2</sup>  |
| 1: rightward c81     | { {58, 490, 922, 1192, 1354, 1786, 2218, 2650, 2920, 3028, 3082, 3514, 3946, 4378, 4432},<br>{340, 394, 826, 1258, 1690, 2122, 2554, 2986, 3418, 3796, 3850, 4282},<br>{346, 616, 724, 778, 1210, 1642, 2074, 2344, 2506, 2938, 3370, 3802, 4072, 4180, 4234},<br>{250, 682, 1114, 1492, 1546, 1978, 2410, 2842, 3274, 3706, 4138, 4570},<br>{40, 202, 634, 1066, 1498, 1768, 1876, 1930, 2362, 2794, 3226, 3496, 3658, 4090, 4522},<br>{106, 538, 970, 1402, 1834, 2266, 2644, 2698, 3130, 3562, 3994, 4426} } | 3 <sup>4</sup>                 | 4608        | 2 <sup>9</sup> 3 <sup>2</sup>  |
| 2                    | { {166, 652, 1030, 1840, 1894, 2380, 2758, 3298, 3352, 3622, 3892, 4108, 4486, 5350, 5836, 6214, 6808, 7078, 7564, 7942, 8644, 8752, 8806, 9292, 9670, 10210, 10264, 10534, 10804, 11020, 11398, 12262, 12748, 13126, 13720, 13990, 14476, 14854, 15664, 15718, 16204, 16582, 17122, 17176, 17446, 17716, 17932, 18310, 19174, 19336, 19660, 20038, 20632, 20902, 21388, 21712, 21766, 22468, 22576, 22630, 23116, 23494, 24034, 24088, 24358, 24628, 24844, 25222, 26086, 26572, 26950, 27544, 27814,          | 3 <sup>4</sup> 13 <sup>1</sup> | 73 728      | 2 <sup>13</sup> 3 <sup>2</sup> |

```

28 300, 28 678, 29 488, 29 542, 30 028, 30 406, 30 946, 31 000, 31 270, 31 540, 31 756,
32 134, 32 998, 33 484, 33 862, 34 456, 34 726, 35 212, 35 590, 36 292, 36 400, 36 454,
36 940, 37 318, 37 858, 37 912, 38 182, 38 452, 38 668, 39 046, 39 910, 40 396, 40 720,
40 774, 41 368, 41 638, 42 124, 42 502, 42 772, 43 312, 43 366, 43 852, 44 230, 44 770,
44 824, 45 094, 45 364, 45 580, 45 958, 46 822, 46 984, 47 308, 47 686, 48 280, 48 550,
49 036, 49 360, 49 414, 50 116, 50 224, 50 278, 50 764, 51 142, 51 682, 51 736, 52 006,
52 276, 52 492, 52 870, 53 734, 54 220, 54 598, 55 192, 55 462, 55 948, 56 326, 57 136,
57 190, 57 676, 58 054, 58 594, 58 648, 58 918, 59 188, 59 404, 59 782, 60 646, 61 132,
61 510, 62 104, 62 374, 62 860, 63 238, 63 940, 64 048, 64 102, 64 588, 64 966, 65 506,
65 560, 65 830, 66 100, 66 316, 66 694, 67 558, 68 044, 68 422, 69 016, 69 286, 69 772,
70 150, 70 960, 71 014, 71 500, 71 878, 72 418, 72 472, 72 742, 73 012, 73 228, 73 606},
{70, 934, 1420, 1798, 2500, 2662, 3148, 3526, 4066, 4390, 4660, 4876, 5254, 6118,
6604, 6982, 7846, 8332, 8710, 9574, 10060, 10438, 10978, 11302, 11572, 11788, 12166,
13030, 13516, 13894, 14758, 15244, 15622, 16324, 16486, 16972, 17350, 17890, 18214,
18484, 18700, 19078, 19942, 20428, 20806, 21670, 22156, 22534, 23398, 23884, 24262,
24802, 25126, 25396, 25612, 25990, 26854, 27340, 27718, 28582, 29068, 29446, 30148,
30310, 30796, 31174, 31714, 32038, 32308, 32524, 32902, 33766, 34252, 34630, 35494,
35980, 36358, 36628, 37222, 37708, 38086, 38626, 38950, 39220, 39436, 39814, 40678,
41164, 41542, 42406, 42892, 43270, 43972, 44134, 44620, 44998, 45538, 45862, 46132,
46348, 46726, 47590, 48076, 48454, 49318, 49804, 50182, 51046, 51532, 51910, 52450,
52774, 53044, 53260, 53638, 54502, 54988, 55366, 56230, 56716, 57094, 57796, 57958,
58444, 58822, 59362, 59686, 59956, 60172, 60550, 61414, 61900, 62278, 63142,
63628, 64006, 64870, 65356, 65734, 66274, 66598, 66868, 67084, 67462, 68326,
68812, 69190, 70054, 70540, 70918, 71620, 71782, 72268, 72646, 73186, 73510},
{76, 454, 994, 1048, 1318, 1588, 1804, 2182, 3046, 3532, 3856, 3910, 4504, 4774, 5260,
5638, 5908, 6448, 6502, 6988, 7366, 7906, 7960, 8230, 8500, 8716, 9094, 9958, 10120,
10444, 10822, 11416, 11686, 12172, 12496, 12550, 13252, 13360, 13414, 13900, 14278,
14818, 14872, 15142, 15412, 15628, 16006, 16870, 17356, 17734, 18328, 18598, 19084,
19462, 20272, 20326, 20812, 21190, 21730, 21784, 22054, 22324, 22540, 22918, 23782,
24268, 24646, 25240, 25510, 25996, 26374, 27076, 27184, 27238, 27724, 28102,
28642, 28696, 28966, 29236, 29452, 29830, 30694, 31180, 31558, 32152, 32422,
32908, 33286, 34096, 34150, 34636, 35014, 35554, 35608, 35878, 36148, 36364,
36742, 37606, 37768, 38092, 38470, 39064, 39334, 39820, 40144, 40198, 40900,
41008, 41062, 41548, 41926, 42466, 42520, 42790, 43060, 43276, 43654, 44518,
45004, 45382, 45976, 46246, 46732, 47110, 47920, 47974, 48460, 48838, 49378,
49432, 49702, 49972, 50188, 50566, 51430, 51916, 52294, 52888, 53158, 53644,
54022, 54724, 54822, 54886, 55272, 55750, 56200, 56244, 56614, 56884, 57100

```

Out[134]=

34022, 34724, 34832, 34880, 35372, 35730, 36230, 36344, 36614, 36884, 37100,  
 57478, 58342, 58828, 59152, 59206, 59800, 60070, 60556, 60934, 61204, 61744,  
 61798, 62284, 62662, 63202, 63256, 63526, 63796, 64012, 64390, 65254, 65416,  
 65740, 66118, 66712, 66982, 67468, 67792, 67846, 68548, 68656, 68710, 69196,  
 69574, 70114, 70168, 70438, 70708, 70924, 71302, 72166, 72652, 73030, 73624},  
 {358, 844, 1222, 1762, 2086, 2356, 2572, 2950, 3814, 4300, 4678, 5542, 6028, 6406,  
 7108, 7270, 7756, 8134, 8674, 8998, 9268, 9484, 9862, 10726, 11212, 11590, 12454,  
 12940, 13318, 14182, 14668, 15046, 15586, 15910, 16180, 16396, 16774, 17638, 18124,  
 18502, 19366, 19852, 20230, 20932, 21094, 21580, 21958, 22498, 22822, 23092, 23308,  
 23686, 24550, 25036, 25414, 26278, 26764, 27142, 28006, 28492, 28870, 29410, 29734,  
 30004, 30220, 30598, 31462, 31948, 32326, 33190, 33676, 34054, 34756, 34918, 35404,  
 35782, 36322, 36646, 36916, 37132, 37510, 38374, 38860, 39238, 40102, 40588, 40966,  
 41830, 42316, 42694, 43234, 43558, 43828, 44044, 44422, 45286, 45772, 46150, 47014,  
 47500, 47878, 48580, 48742, 49228, 49606, 50146, 50470, 50740, 50956, 51334, 52198,  
 52684, 53062, 53926, 54412, 54790, 55060, 55654, 56140, 56518, 57058, 57382, 57652,  
 57868, 58246, 59110, 59596, 59974, 60838, 61324, 61702, 62404, 62566, 63052,  
 63430, 63970, 64294, 64564, 64780, 65158, 66022, 66508, 66886, 67750, 68236,  
 68614, 69478, 69964, 70342, 70882, 71206, 71476, 71692, 72070, 72934, 73420},  
 {742, 904, 1228, 1606, 2200, 2470, 2956, 3280, 3334, 4036, 4144, 4198, 4684, 5062,  
 5602, 5656, 5926, 6196, 6412, 6790, 7654, 8140, 8518, 9112, 9382, 9868, 10246, 11056,  
 11110, 11596, 11974, 12514, 12568, 12838, 13108, 13324, 13702, 14566, 15052, 15430,  
 16024, 16294, 16780, 17158, 17860, 17968, 18022, 18508, 18886, 19426, 19480,  
 19750, 20020, 20236, 20614, 21478, 21964, 22288, 22342, 22936, 23206, 23692,  
 24070, 24340, 24880, 24934, 25420, 25798, 26338, 26392, 26662, 26932, 27148,  
 27526, 28390, 28552, 28876, 29254, 29848, 30118, 30604, 30928, 30982, 31684,  
 31792, 31846, 32332, 32710, 33250, 33304, 33574, 33844, 34060, 34438, 35302,  
 35788, 36166, 36760, 37030, 37516, 37894, 38704, 38758, 39244, 39622, 40162,  
 40216, 40486, 40756, 40972, 41350, 42214, 42700, 43078, 43672, 43942, 44428,  
 44806, 45508, 45616, 45670, 46156, 46534, 47074, 47128, 47398, 47668, 47884,  
 48208, 48262, 49126, 49612, 49990, 50584, 50854, 51340, 51718, 52528, 52582,  
 53068, 53446, 53986, 54040, 54310, 54580, 54796, 55174, 56038, 56200, 56524,  
 56902, 57496, 57766, 58252, 58576, 58630, 59332, 59440, 59494, 59980, 60358,  
 60898, 60952, 61222, 61492, 61708, 62086, 62950, 63436, 63814, 64408, 64678,  
 65164, 65542, 66352, 66406, 66892, 67270, 67810, 67864, 68134, 68404, 68620,  
 68998, 69862, 70348, 70726, 71320, 71590, 72076, 72454, 73156, 73264, 73318},  
 {52, 268, 646, 1510, 1996, 2374, 3238, 3724, 4102, 4966, 5452, 5830, 6370, 6694, 6964,  
 7180, 7558, 8422, 8908, 9286, 10150, 10636, 11014, 11716, 11878, 12364, 12742,

```

13 282, 13 606, 13 876, 14 092, 14 470, 15 334, 15 820, 16 198, 17 062, 17 548, 17 926, 18 196,
18 790, 19 276, 19 654, 20 194, 20 518, 20 788, 21 004, 21 382, 22 246, 22 732, 23 110, 23 974,
24 460, 24 838, 25 540, 25 702, 26 188, 26 566, 27 106, 27 430, 27 700, 27 916, 28 294, 29 158,
29 644, 30 022, 30 886, 31 372, 31 750, 32 614, 33 100, 33 478, 34 018, 34 342, 34 612, 34 828,
35 206, 36 070, 36 556, 36 934, 37 798, 38 284, 38 662, 39 364, 39 526, 40 012, 40 390, 40 930,
41 254, 41 524, 41 740, 42 118, 42 982, 43 468, 43 846, 44 710, 45 196, 45 574, 46 438, 46 924,
47 302, 47 842, 48 166, 48 436, 48 652, 49 030, 49 894, 50 380, 50 758, 51 622, 52 108, 52 486,
53 188, 53 350, 53 836, 54 214, 54 754, 55 078, 55 348, 55 564, 55 942, 56 806, 57 292, 57 670,
58 534, 59 020, 59 398, 60 262, 60 748, 61 126, 61 666, 61 990, 62 260, 62 476, 62 854,
63 718, 64 204, 64 582, 65 446, 65 932, 66 310, 67 012, 67 174, 67 660, 68 038, 68 578,
68 902, 69 172, 69 388, 69 766, 70 630, 71 116, 71 494, 72 358, 72 844, 73 222, 73 492}}

```

The grid for c351k is printed for  $k=0$  (rightward congruence classes c27) only, the first iteration with  $c351=27 \cdot 13$  congruence classes, and the second iteration with  $351 \cdot 13=27 \cdot 13^2$  iterations because it is just the combination of c81k and c351k.

```

In[135]:= Grid[
  Prepend[
    ReplacePart[cNk[c351k, 2], {{1, 1} → "0: rightward c27", {2, 1} → "1: rightward c351"}],
    {"t≥k right nested", "351·13k-1 congruence classes", "cardinality", "periodicity"}],
  Dividers → {False, {True, True}}, Alignment → Left]

```

| $t_{\geq k}$ right nested | $351 \cdot 13^{k-1}$ congruence classes                                                                                                                                                                                                                                                                                                                                                                                                                                                                                                                                                                                                                                                                                                                                                                                                                                                                                                                                                                                   | cardinality      | periodicity                |
|---------------------------|---------------------------------------------------------------------------------------------------------------------------------------------------------------------------------------------------------------------------------------------------------------------------------------------------------------------------------------------------------------------------------------------------------------------------------------------------------------------------------------------------------------------------------------------------------------------------------------------------------------------------------------------------------------------------------------------------------------------------------------------------------------------------------------------------------------------------------------------------------------------------------------------------------------------------------------------------------------------------------------------------------------------------|------------------|----------------------------|
| 0: rightward c27          | {4, 22, 34, 40, 52, 58, 70, 76, 94, 106, 112, 124, 130, 142, 148, 166, 178, 184, 196, 202, 214, 220, 238, 250, 268, 274, 286}                                                                                                                                                                                                                                                                                                                                                                                                                                                                                                                                                                                                                                                                                                                                                                                                                                                                                             | $3^3$            | $288 \cdot 2^5 \cdot 3^2$  |
| 1: rightward c351         | {4, 112, 166, 220, 274, 328, 382, 436, 598, 652, 706, 760, 814, 868, 976, 1030, 1084, 1138, 1246, 1300, 1462, 1516, 1570, 1624, 1678, 1732, 1840, 1894, 1948, 2002, 2056, 2110, 2164, 2326, 2380, 2434, 2488, 2542, 2596, 2704, 2758, 2812, 2866, 2974, 3190, 3244, 3298, 3352, 3406, 3460, 3568, 3622, 3676, 3730, 3784, 3838, 3892, 4054, 4108, 4162, 4216, 4270, 4324, 4486, 4540, 4594}, {70, 124, 178, 286, 502, 556, 610, 718, 772, 934, 988, 1042, 1150, 1204, 1366, 1420, 1474, 1582, 1636, 1798, 1852, 1906, 2014, 2068, 2230, 2284, 2338, 2446, 2500, 2662, 2716, 2770, 2878, 2932, 3094, 3148, 3202, 3310, 3364, 3526, 3580, 3634, 3742, 3958, 4012, 4066, 4174, 4228, 4390, 4444, 4498, 4606}, {22, 76, 130, 184, 238, 292, 400, 454, 508, 562, 670, 886, 940, 994, 1048, 1102, 1156, 1264, 1318, 1372, 1426, 1480, 1534, 1588, 1750, 1804, 1858, 1912, 1966, 2020, 2128, 2182, 2236, 2290, 2398, 2452, 2614, 2668, 2722, 2776, 2830, 2884, 2992, 3046, 3100, 3154, 3208, 3262, 3316, 3478, 3532, 3586, 3640} | $3^3 \cdot 13^1$ | $4608 \cdot 2^9 \cdot 3^2$ |

2830, 2884, 2932, 3040, 3100, 3134, 3200, 3202, 3310, 3470, 3532, 3580, 3640,  
 3694, 3748, 3856, 3910, 3964, 4018, 4126, 4342, 4396, 4450, 4504, 4558},  
 {34, 142, 196, 358, 412, 466, 574, 628, 790, 844, 898, 1006, 1060, 1222, 1276,  
 1330, 1438, 1654, 1708, 1762, 1870, 1924, 2086, 2140, 2194, 2302, 2356,  
 2518, 2572, 2626, 2734, 2788, 2950, 3004, 3058, 3166, 3220, 3382, 3436, 3490,  
 3598, 3652, 3814, 3868, 3922, 4030, 4084, 4246, 4300, 4354, 4462, 4516},  
 {94, 148, 310, 364, 418, 472, 526, 580, 688, 742, 796, 850, 904, 958, 1012,  
 1174, 1228, 1282, 1336, 1390, 1444, 1552, 1606, 1660, 1714, 1822, 2038,  
 2092, 2146, 2200, 2254, 2308, 2416, 2470, 2524, 2578, 2632, 2686, 2740,  
 2902, 2956, 3010, 3064, 3118, 3172, 3280, 3334, 3388, 3442, 3550, 3604, 3766,  
 3820, 3874, 3928, 3982, 4036, 4144, 4198, 4252, 4306, 4360, 4414, 4468},  
 {52, 214, 268, 322, 430, 484, 646, 700, 754, 862, 916, 1078, 1132, 1186, 1294,  
 1348, 1510, 1564, 1618, 1726, 1780, 1942, 1996, 2050, 2158, 2212, 2374,  
 2428, 2482, 2590, 2806, 2860, 2914, 3022, 3076, 3238, 3292, 3346, 3454, 3508,  
 3670, 3724, 3778, 3886, 3940, 4102, 4156, 4210, 4318, 4372, 4534, 4588}}}

2

{ {4, 112, 220, 274, 328, 382, 436, 598, 706, 760, 814, 868, 976, 1084, 1138, 1246, 1300, 1462,  $3^3 13^2$  73 728  $2^{13} 3^2$   
 1516, 1570, 1624, 1678, 1732, 1948, 2002, 2056, 2110, 2164, 2326, 2434, 2488, 2542,  
 2596, 2704, 2812, 2866, 2974, 3190, 3244, 3406, 3460, 3568, 3676, 3730, 3784, 3838,  
 4054, 4162, 4216, 4270, 4324, 4540, 4594, 4702, 4756, 4918, 4972, 5026, 5080, 5134,  
 5188, 5296, 5404, 5458, 5512, 5566, 5620, 5782, 5890, 5944, 5998, 6052, 6160, 6268,  
 6322, 6430, 6646, 6700, 6754, 6862, 6916, 7024, 7132, 7186, 7240, 7294, 7348, 7510,  
 7618, 7672, 7726, 7780, 7888, 7996, 8050, 8158, 8212, 8374, 8428, 8482, 8536, 8590,  
 8860, 8914, 8968, 9022, 9076, 9238, 9346, 9400, 9454, 9508, 9616, 9724, 9778, 9886,  
 10102, 10156, 10318, 10372, 10480, 10588, 10642, 10696, 10750, 10966, 11074, 11128,  
 11182, 11236, 11344, 11452, 11506, 11614, 11668, 11830, 11884, 11938, 11992, 12046,  
 12100, 12208, 12316, 12370, 12424, 12478, 12532, 12694, 12802, 12856, 12910, 12964,  
 13072, 13180, 13234, 13342, 13558, 13612, 13666, 13774, 13828, 13936, 14044, 14098,  
 14152, 14206, 14260, 14422, 14530, 14584, 14638, 14692, 14800, 14908, 14962,  
 15070, 15124, 15286, 15340, 15394, 15448, 15502, 15556, 15772, 15826, 15880,  
 15934, 15988, 16150, 16258, 16312, 16366, 16420, 16528, 16636, 16690, 16798, 17014,  
 17068, 17230, 17284, 17392, 17500, 17554, 17608, 17662, 17878, 17986, 18040,  
 18094, 18148, 18364, 18418, 18526, 18580, 18742, 18796, 18850, 18904, 18958,  
 19012, 19120, 19228, 19282, 19390, 19444, 19606, 19714, 19768, 19822, 19876,  
 19984, 20092, 20146, 20254, 20470, 20524, 20578, 20686, 20740, 20848, 20956,  
 21010, 21064, 21118, 21172, 21334, 21442, 21496, 21550, 21604, 21820, 21874,  
 21982, 22036, 22198, 22252, 22306, 22360, 22414, 22684, 22738, 22792, 22846,  
 22900, 23062, 23170, 23224, 23278, 23332, 23440, 23548, 23602, 23710, 23926,

23 980, 24 142, 24 196, 24 304, 24 412, 24 466, 24 520, 24 574, 24 790, 24 898, 24 952,  
 25 006, 25 060, 25 168, 25 276, 25 330, 25 438, 25 492, 25 654, 25 708, 25 762, 25 816,  
 25 870, 25 924, 26 032, 26 140, 26 194, 26 248, 26 302, 26 356, 26 518, 26 626, 26 680,  
 26 734, 26 788, 26 896, 27 004, 27 058, 27 166, 27 382, 27 436, 27 490, 27 598, 27 652,  
 27 760, 27 868, 27 922, 27 976, 28 030, 28 084, 28 246, 28 354, 28 408, 28 462, 28 516,  
 28 624, 28 732, 28 786, 28 894, 28 948, 29 110, 29 164, 29 218, 29 272, 29 326, 29 380,  
 29 596, 29 650, 29 704, 29 758, 29 812, 29 974, 30 082, 30 136, 30 190, 30 244, 30 352,  
 30 460, 30 514, 30 622, 30 838, 30 892, 31 054, 31 108, 31 216, 31 324, 31 378, 31 432,  
 31 486, 31 702, 31 810, 31 864, 31 918, 31 972, 32 188, 32 242, 32 350, 32 404, 32 566,  
 32 620, 32 674, 32 728, 32 782, 32 836, 32 944, 33 052, 33 106, 33 160, 33 214, 33 268,  
 33 430, 33 538, 33 592, 33 646, 33 700, 33 808, 33 916, 33 970, 34 078, 34 294, 34 348,  
 34 402, 34 510, 34 564, 34 672, 34 780, 34 834, 34 888, 34 942, 34 996, 35 158, 35 266,  
 35 320, 35 374, 35 428, 35 536, 35 644, 35 698, 35 806, 35 860, 36 022, 36 076, 36 130,  
 36 184, 36 238, 36 508, 36 562, 36 616, 36 670, 36 724, 36 886, 36 994, 37 048, 37 102,  
 37 156, 37 264, 37 372, 37 426, 37 534, 37 750, 37 804, 37 966, 38 020, 38 128, 38 236,  
 38 290, 38 344, 38 398, 38 614, 38 722, 38 776, 38 830, 38 884, 38 992, 39 100, 39 154,  
 39 262, 39 316, 39 478, 39 532, 39 586, 39 640, 39 694, 39 748, 39 856, 39 964, 40 018,  
 40 072, 40 126, 40 180, 40 342, 40 450, 40 504, 40 558, 40 612, 40 828, 40 882, 40 990,  
 41 206, 41 260, 41 314, 41 422, 41 476, 41 584, 41 692, 41 746, 41 800, 41 854, 41 908,  
 42 070, 42 178, 42 232, 42 286, 42 340, 42 448, 42 556, 42 610, 42 718, 42 934, 42 988,  
 43 042, 43 096, 43 150, 43 204, 43 420, 43 474, 43 528, 43 582, 43 636, 43 798, 43 906,  
 43 960, 44 014, 44 068, 44 176, 44 284, 44 338, 44 446, 44 662, 44 716, 44 878, 44 932,  
 45 040, 45 148, 45 202, 45 256, 45 310, 45 526, 45 634, 45 688, 45 742, 45 796, 46 012,  
 46 066, 46 174, 46 228, 46 390, 46 444, 46 498, 46 552, 46 606, 46 660, 46 768, 46 876,  
 46 930, 47 038, 47 092, 47 254, 47 362, 47 416, 47 470, 47 524, 47 632, 47 740, 47 794,  
 47 902, 48 118, 48 172, 48 226, 48 334, 48 388, 48 496, 48 604, 48 658, 48 712, 48 766,  
 48 820, 48 982, 49 090, 49 144, 49 198, 49 252, 49 468, 49 522, 49 630, 49 684, 49 846,  
 49 900, 49 954, 50 008, 50 062, 50 332, 50 386, 50 440, 50 494, 50 548, 50 710, 50 818,  
 50 872, 50 926, 50 980, 51 088, 51 196, 51 250, 51 358, 51 574, 51 628, 51 790, 51 844,  
 51 952, 52 060, 52 114, 52 168, 52 222, 52 438, 52 546, 52 600, 52 654, 52 708, 52 816,  
 52 924, 52 978, 53 086, 53 140, 53 302, 53 356, 53 410, 53 464, 53 518, 53 572, 53 680,  
 53 788, 53 842, 53 896, 53 950, 54 004, 54 166, 54 274, 54 328, 54 382, 54 436, 54 544,  
 54 652, 54 706, 54 814, 55 030, 55 084, 55 138, 55 246, 55 300, 55 408, 55 516, 55 570,  
 55 624, 55 678, 55 732, 55 894, 56 002, 56 056, 56 110, 56 164, 56 272, 56 380, 56 434,  
 56 542, 56 596, 56 758, 56 812, 56 866, 56 920, 56 974, 57 028, 57 244, 57 298, 57 352,  
 57 406, 57 460, 57 622, 57 730, 57 784, 57 838, 57 892, 58 000, 58 108, 58 162, 58 270,

58486, 58540, 58702, 58756, 58864, 58972, 59026, 59080, 59134, 59350, 59458,  
 59512, 59566, 59620, 59836, 59890, 59998, 60052, 60214, 60268, 60322, 60376,  
 60430, 60484, 60592, 60700, 60754, 60808, 60862, 60916, 61078, 61186, 61240,  
 61294, 61348, 61456, 61564, 61618, 61726, 61942, 61996, 62050, 62158, 62212,  
 62320, 62428, 62482, 62536, 62590, 62644, 62806, 62914, 62968, 63022, 63076,  
 63184, 63292, 63346, 63454, 63508, 63670, 63724, 63778, 63832, 63886, 64156,  
 64210, 64264, 64318, 64372, 64534, 64642, 64696, 64750, 64804, 64912, 65020,  
 65074, 65182, 65398, 65452, 65614, 65668, 65776, 65884, 65938, 65992, 66046,  
 66262, 66370, 66424, 66478, 66532, 66640, 66748, 66802, 66910, 66964, 67126,  
 67180, 67234, 67288, 67342, 67396, 67504, 67612, 67666, 67720, 67774, 67828,  
 67990, 68098, 68152, 68206, 68260, 68368, 68476, 68530, 68638, 68854, 68908,  
 68962, 69070, 69124, 69232, 69340, 69394, 69448, 69502, 69556, 69718, 69826,  
 69880, 69934, 69988, 70096, 70204, 70258, 70366, 70420, 70582, 70636, 70690,  
 70744, 70798, 70852, 71068, 71122, 71176, 71230, 71284, 71446, 71554, 71608,  
 71662, 71716, 71824, 71932, 71986, 72094, 72310, 72364, 72526, 72580, 72688,  
 72796, 72850, 72904, 72958, 73174, 73282, 73336, 73390, 73444, 73660, 73714},  
 {124, 178, 286, 502, 556, 610, 718, 772, 988, 1042, 1150, 1204, 1366, 1474, 1582,  
 1636, 1852, 1906, 2014, 2068, 2230, 2284, 2338, 2446, 2716, 2770, 2878, 2932, 3094,  
 3202, 3310, 3364, 3580, 3634, 3742, 3958, 4012, 4174, 4228, 4444, 4498, 4606, 4822,  
 4930, 5038, 5092, 5308, 5362, 5470, 5524, 5686, 5740, 5794, 5902, 5956, 6172, 6226,  
 6334, 6388, 6550, 6658, 6766, 6820, 7036, 7090, 7198, 7414, 7468, 7522, 7630, 7684,  
 7900, 7954, 8062, 8116, 8278, 8386, 8494, 8548, 8764, 8818, 8926, 8980, 9142, 9196,  
 9250, 9358, 9412, 9628, 9682, 9790, 9844, 10006, 10114, 10222, 10276, 10492, 10546,  
 10654, 10870, 10924, 11086, 11140, 11356, 11410, 11518, 11734, 11842, 11950, 12004,  
 12220, 12274, 12382, 12436, 12598, 12652, 12706, 12814, 12868, 13084, 13138, 13246,  
 13300, 13462, 13570, 13678, 13732, 13948, 14002, 14110, 14326, 14380, 14434, 14542,  
 14596, 14812, 14866, 14974, 15028, 15190, 15298, 15406, 15460, 15676, 15730, 15838,  
 15892, 16054, 16108, 16162, 16270, 16540, 16594, 16702, 16756, 16918, 17026, 17134,  
 17188, 17404, 17458, 17566, 17782, 17836, 17998, 18052, 18268, 18322, 18430, 18646,  
 18754, 18862, 18916, 19132, 19186, 19294, 19348, 19510, 19564, 19618, 19726,  
 19780, 19996, 20050, 20158, 20212, 20374, 20482, 20590, 20644, 20860, 20914,  
 21022, 21238, 21292, 21346, 21454, 21508, 21724, 21778, 21886, 21940, 22102,  
 22210, 22318, 22372, 22588, 22642, 22750, 22804, 22966, 23020, 23074, 23182,  
 23236, 23452, 23506, 23614, 23668, 23830, 23938, 24046, 24100, 24316, 24370,  
 24478, 24694, 24748, 24910, 24964, 25180, 25234, 25342, 25558, 25666, 25774,  
 25828, 26044, 26098, 26206, 26260, 26422, 26476, 26530, 26638, 26692, 26908,  
 26962, 27070, 27124, 27286, 27340, 27502, 27556, 27772, 27826, 27934, 28150

20 502, 21 070, 21 124, 21 200, 21 334, 21 302, 21 330, 21 772, 21 020, 21 334, 20 130,  
 28 204, 28 258, 28 366, 28 420, 28 636, 28 690, 28 798, 28 852, 29 014, 29 122, 29 230,  
 29 284, 29 500, 29 554, 29 662, 29 716, 29 878, 29 932, 29 986, 30 094, 30 364, 30 418,  
 30 526, 30 580, 30 742, 30 850, 30 958, 31 012, 31 228, 31 282, 31 390, 31 606, 31 660,  
 31 822, 31 876, 32 092, 32 146, 32 254, 32 470, 32 578, 32 686, 32 740, 32 956, 33 010,  
 33 118, 33 172, 33 334, 33 388, 33 442, 33 550, 33 604, 33 820, 33 874, 33 982, 34 036,  
 34 198, 34 306, 34 414, 34 468, 34 684, 34 738, 34 846, 35 062, 35 116, 35 170, 35 278,  
 35 332, 35 548, 35 602, 35 710, 35 764, 35 926, 36 034, 36 142, 36 196, 36 412, 36 466,  
 36 574, 36 790, 36 844, 36 898, 37 006, 37 060, 37 276, 37 330, 37 438, 37 492, 37 654,  
 37 762, 37 870, 37 924, 38 140, 38 194, 38 302, 38 518, 38 572, 38 734, 38 788, 39 004,  
 39 058, 39 166, 39 382, 39 490, 39 598, 39 652, 39 868, 39 922, 40 030, 40 084, 40 246,  
 40 300, 40 354, 40 462, 40 516, 40 732, 40 786, 40 894, 40 948, 41 110, 41 218, 41 326,  
 41 380, 41 596, 41 650, 41 758, 41 974, 42 028, 42 082, 42 190, 42 244, 42 460, 42 514,  
 42 622, 42 676, 42 838, 42 946, 43 054, 43 108, 43 324, 43 378, 43 486, 43 540, 43 702,  
 43 756, 43 810, 43 918, 44 188, 44 242, 44 350, 44 404, 44 566, 44 674, 44 782, 44 836,  
 45 052, 45 106, 45 214, 45 430, 45 484, 45 646, 45 700, 45 916, 45 970, 46 078, 46 294,  
 46 402, 46 510, 46 564, 46 780, 46 834, 46 942, 46 996, 47 158, 47 212, 47 266, 47 374,  
 47 428, 47 644, 47 698, 47 806, 47 860, 48 022, 48 130, 48 238, 48 292, 48 508, 48 562,  
 48 670, 48 886, 48 940, 48 994, 49 102, 49 156, 49 372, 49 426, 49 534, 49 588, 49 750,  
 49 858, 49 966, 50 020, 50 236, 50 290, 50 398, 50 452, 50 614, 50 668, 50 722, 50 830,  
 50 884, 51 100, 51 154, 51 262, 51 316, 51 478, 51 586, 51 694, 51 748, 51 964, 52 018,  
 52 126, 52 342, 52 396, 52 558, 52 612, 52 828, 52 882, 52 990, 53 206, 53 314, 53 422,  
 53 476, 53 692, 53 746, 53 854, 53 908, 54 070, 54 124, 54 178, 54 286, 54 340, 54 556,  
 54 610, 54 718, 54 772, 54 934, 55 042, 55 150, 55 204, 55 420, 55 474, 55 582, 55 798,  
 55 852, 55 906, 56 014, 56 068, 56 284, 56 338, 56 446, 56 500, 56 662, 56 770, 56 878,  
 56 932, 57 148, 57 202, 57 310, 57 364, 57 526, 57 580, 57 634, 57 742, 58 012, 58 066,  
 58 174, 58 228, 58 390, 58 498, 58 606, 58 660, 58 876, 58 930, 59 038, 59 254, 59 308,  
 59 470, 59 524, 59 740, 59 794, 59 902, 60 118, 60 226, 60 334, 60 388, 60 604, 60 658,  
 60 766, 60 820, 60 982, 61 036, 61 090, 61 198, 61 252, 61 468, 61 522, 61 630, 61 684,  
 61 846, 61 954, 62 062, 62 116, 62 332, 62 386, 62 494, 62 710, 62 764, 62 818, 62 926,  
 62 980, 63 196, 63 250, 63 358, 63 412, 63 574, 63 682, 63 790, 63 844, 64 060, 64 114,  
 64 222, 64 276, 64 438, 64 492, 64 546, 64 654, 64 708, 64 924, 64 978, 65 086, 65 140,  
 65 302, 65 410, 65 518, 65 572, 65 788, 65 842, 65 950, 66 166, 66 220, 66 382, 66 436,  
 66 652, 66 706, 66 814, 67 030, 67 138, 67 246, 67 300, 67 516, 67 570, 67 678, 67 732,  
 67 894, 67 948, 68 002, 68 110, 68 164, 68 380, 68 434, 68 542, 68 596, 68 758, 68 866,  
 68 974, 69 028, 69 244, 69 298, 69 406, 69 622, 69 676, 69 730, 69 838, 69 892, 70 108,  
 70 162, 70 270, 70 324, 70 486, 70 594, 70 702, 70 756, 70 972, 71 026, 71 134, 71 188,



71350, 71404, 71458, 71566, 71836, 71890, 71998, 72052, 72214, 72322, 72430,  
 72484, 72700, 72754, 72862, 73078, 73132, 73294, 73348, 73564, 73618, 73726},  
 {22, 130, 184, 238, 292, 400, 508, 562, 670, 886, 940, 1102, 1156, 1264, 1372, 1426,  
 1480, 1534, 1750, 1858, 1912, 1966, 2020, 2128, 2236, 2290, 2398, 2452, 2614, 2668,  
 2722, 2776, 2830, 2884, 2992, 3100, 3154, 3208, 3262, 3316, 3478, 3586, 3640, 3694,  
 3748, 3964, 4018, 4126, 4342, 4396, 4450, 4558, 4612, 4720, 4828, 4882, 4936, 4990,  
 5044, 5206, 5314, 5368, 5422, 5476, 5584, 5692, 5746, 5854, 6070, 6124, 6178, 6232,  
 6286, 6340, 6556, 6610, 6664, 6718, 6772, 6934, 7042, 7096, 7150, 7204, 7312, 7420,  
 7474, 7582, 7798, 7852, 8014, 8068, 8176, 8284, 8338, 8392, 8446, 8662, 8770, 8824,  
 8878, 8932, 9148, 9202, 9310, 9364, 9526, 9580, 9634, 9688, 9742, 9796, 9904, 10012,  
 10066, 10174, 10228, 10390, 10498, 10552, 10606, 10660, 10768, 10876, 10930, 11038,  
 11254, 11308, 11362, 11470, 11524, 11632, 11740, 11794, 11848, 11902, 11956, 12118,  
 12226, 12280, 12334, 12388, 12604, 12658, 12766, 12820, 12982, 13036, 13090, 13144,  
 13198, 13468, 13522, 13576, 13630, 13684, 13846, 13954, 14008, 14062, 14116,  
 14224, 14332, 14386, 14494, 14710, 14764, 14926, 14980, 15088, 15196, 15250,  
 15304, 15358, 15574, 15682, 15736, 15790, 15844, 15952, 16060, 16114, 16222,  
 16276, 16438, 16492, 16546, 16600, 16654, 16708, 16816, 16924, 16978, 17032,  
 17086, 17140, 17302, 17410, 17464, 17518, 17572, 17680, 17788, 17842, 17950,  
 18166, 18220, 18274, 18382, 18436, 18544, 18652, 18706, 18760, 18814, 18868,  
 19030, 19138, 19192, 19246, 19300, 19408, 19516, 19570, 19678, 19732, 19894,  
 19948, 20002, 20056, 20110, 20164, 20380, 20434, 20488, 20542, 20596, 20758,  
 20866, 20920, 20974, 21028, 21136, 21244, 21298, 21406, 21622, 21676, 21838,  
 21892, 22000, 22108, 22162, 22216, 22270, 22486, 22594, 22648, 22702, 22756,  
 22972, 23026, 23134, 23188, 23350, 23404, 23458, 23512, 23566, 23620, 23728,  
 23836, 23890, 23944, 23998, 24052, 24214, 24322, 24376, 24430, 24484, 24592,  
 24700, 24754, 24862, 25078, 25132, 25186, 25294, 25348, 25456, 25564, 25618,  
 25672, 25726, 25780, 25942, 26050, 26104, 26158, 26212, 26320, 26428, 26482,  
 26590, 26644, 26806, 26860, 26914, 26968, 27022, 27292, 27346, 27400, 27454,  
 27508, 27670, 27778, 27832, 27886, 27940, 28048, 28156, 28210, 28318, 28534,  
 28588, 28750, 28804, 28912, 29020, 29074, 29128, 29182, 29398, 29506, 29560,  
 29614, 29668, 29776, 29884, 29938, 30046, 30100, 30262, 30316, 30370, 30424,  
 30478, 30532, 30640, 30748, 30802, 30856, 30910, 30964, 31126, 31234, 31288,  
 31342, 31396, 31504, 31612, 31666, 31774, 31990, 32044, 32098, 32206, 32260,  
 32368, 32476, 32530, 32584, 32638, 32692, 32854, 32962, 33016, 33070, 33124,  
 33232, 33340, 33394, 33502, 33556, 33718, 33772, 33826, 33880, 33934, 33988,  
 34204, 34258, 34312, 34366, 34420, 34582, 34690, 34744, 34798, 34852, 34960,

Out[135]=

35 068, 35 122, 35 230, 35 446, 35 500, 35 662, 35 716, 35 824, 35 932, 35 986, 36 040,  
 36 094, 36 310, 36 418, 36 472, 36 526, 36 580, 36 796, 36 850, 36 958, 37 012, 37 174,  
 37 228, 37 282, 37 336, 37 390, 37 444, 37 552, 37 660, 37 714, 37 822, 37 876, 38 038,  
 38 146, 38 200, 38 254, 38 308, 38 416, 38 524, 38 578, 38 686, 38 902, 38 956, 39 010,  
 39 118, 39 172, 39 280, 39 388, 39 442, 39 496, 39 550, 39 604, 39 766, 39 874, 39 928,  
 39 982, 40 036, 40 252, 40 306, 40 414, 40 468, 40 630, 40 684, 40 738, 40 792, 40 846,  
 41 116, 41 170, 41 224, 41 278, 41 332, 41 494, 41 602, 41 656, 41 710, 41 764, 41 872,  
 41 980, 42 034, 42 142, 42 358, 42 412, 42 574, 42 628, 42 736, 42 844, 42 898, 42 952,  
 43 006, 43 222, 43 330, 43 384, 43 438, 43 492, 43 600, 43 708, 43 762, 43 870, 43 924,  
 44 086, 44 140, 44 194, 44 248, 44 302, 44 356, 44 464, 44 572, 44 626, 44 680, 44 734,  
 44 788, 44 950, 45 058, 45 112, 45 166, 45 220, 45 328, 45 436, 45 490, 45 598, 45 814,  
 45 868, 45 922, 46 030, 46 084, 46 192, 46 300, 46 354, 46 408, 46 462, 46 516, 46 678,  
 46 786, 46 840, 46 894, 46 948, 47 056, 47 164, 47 218, 47 326, 47 380, 47 542, 47 596,  
 47 650, 47 704, 47 758, 47 812, 48 028, 48 082, 48 136, 48 190, 48 244, 48 406, 48 514,  
 48 568, 48 622, 48 676, 48 784, 48 892, 48 946, 49 054, 49 270, 49 324, 49 486, 49 540,  
 49 648, 49 756, 49 810, 49 864, 49 918, 50 134, 50 242, 50 296, 50 350, 50 404, 50 620,  
 50 674, 50 782, 50 836, 50 998, 51 052, 51 106, 51 160, 51 214, 51 268, 51 376, 51 484,  
 51 538, 51 592, 51 646, 51 700, 51 862, 51 970, 52 024, 52 078, 52 132, 52 240, 52 348,  
 52 402, 52 510, 52 726, 52 780, 52 834, 52 942, 52 996, 53 104, 53 212, 53 266, 53 320,  
 53 374, 53 428, 53 590, 53 698, 53 752, 53 806, 53 860, 53 968, 54 076, 54 130, 54 238,  
 54 292, 54 454, 54 508, 54 562, 54 616, 54 670, 54 940, 54 994, 55 048, 55 102, 55 156,  
 55 318, 55 426, 55 480, 55 534, 55 588, 55 696, 55 804, 55 858, 55 966, 56 182, 56 236,  
 56 398, 56 452, 56 560, 56 668, 56 722, 56 776, 56 830, 57 046, 57 154, 57 208, 57 262,  
 57 316, 57 424, 57 532, 57 586, 57 694, 57 748, 57 910, 57 964, 58 018, 58 072, 58 126,  
 58 180, 58 288, 58 396, 58 450, 58 504, 58 558, 58 612, 58 774, 58 882, 58 936, 58 990,  
 59 044, 59 260, 59 314, 59 422, 59 638, 59 692, 59 746, 59 854, 59 908, 60 016, 60 124,  
 60 178, 60 232, 60 286, 60 340, 60 502, 60 610, 60 664, 60 718, 60 772, 60 880, 60 988,  
 61 042, 61 150, 61 366, 61 420, 61 474, 61 528, 61 582, 61 636, 61 852, 61 906, 61 960,  
 62 014, 62 068, 62 230, 62 338, 62 392, 62 446, 62 500, 62 608, 62 716, 62 770, 62 878,  
 63 094, 63 148, 63 310, 63 364, 63 472, 63 580, 63 634, 63 688, 63 742, 63 958, 64 066,  
 64 120, 64 174, 64 228, 64 444, 64 498, 64 606, 64 660, 64 822, 64 876, 64 930, 64 984,  
 65 038, 65 092, 65 200, 65 308, 65 362, 65 470, 65 524, 65 686, 65 794, 65 848, 65 902,  
 65 956, 66 064, 66 172, 66 226, 66 334, 66 550, 66 604, 66 658, 66 766, 66 820, 66 928,  
 67 036, 67 090, 67 144, 67 198, 67 252, 67 414, 67 522, 67 576, 67 630, 67 684, 67 900,  
 67 954, 68 062, 68 116, 68 278, 68 332, 68 386, 68 440, 68 494, 68 764, 68 818, 68 872,  
 68 926, 68 980, 69 142, 69 250, 69 304, 69 358, 69 412, 69 520, 69 628, 69 682, 69 790,  
 70 006, 70 060, 70 222, 70 276, 70 384, 70 492, 70 546, 70 600, 70 654, 70 870, 70 978.

70000, 70000, 70222, 70270, 70304, 70432, 70570, 70600, 70634, 70670, 70700,  
 71032, 71086, 71140, 71248, 71356, 71410, 71518, 71572, 71734, 71788, 71842,  
 71896, 71950, 72004, 72112, 72220, 72274, 72328, 72382, 72436, 72598, 72706,  
 72760, 72814, 72868, 72976, 73084, 73138, 73246, 73462, 73516, 73570, 73678},  
 {34, 142, 196, 412, 466, 574, 628, 790, 898, 1006, 1060, 1276, 1330, 1438, 1654,  
 1708, 1870, 1924, 2140, 2194, 2302, 2518, 2626, 2734, 2788, 3004, 3058, 3166,  
 3220, 3382, 3436, 3490, 3598, 3652, 3868, 3922, 4030, 4084, 4246, 4354, 4462,  
 4516, 4732, 4786, 4894, 5110, 5164, 5218, 5326, 5380, 5596, 5650, 5758, 5812,  
 5974, 6082, 6190, 6244, 6460, 6514, 6622, 6676, 6838, 6892, 6946, 7054, 7324,  
 7378, 7486, 7540, 7702, 7810, 7918, 7972, 8188, 8242, 8350, 8566, 8620, 8782,  
 8836, 9052, 9106, 9214, 9430, 9538, 9646, 9700, 9916, 9970, 10078, 10132, 10294,  
 10348, 10402, 10510, 10564, 10780, 10834, 10942, 10996, 11158, 11266, 11374,  
 11428, 11644, 11698, 11806, 12022, 12076, 12130, 12238, 12292, 12508, 12562,  
 12670, 12724, 12886, 12994, 13102, 13156, 13372, 13426, 13534, 13588, 13750,  
 13804, 13858, 13966, 14020, 14236, 14290, 14398, 14452, 14614, 14722, 14830,  
 14884, 15100, 15154, 15262, 15478, 15532, 15694, 15748, 15964, 16018, 16126,  
 16342, 16450, 16558, 16612, 16828, 16882, 16990, 17044, 17206, 17260, 17314,  
 17422, 17476, 17692, 17746, 17854, 17908, 18070, 18178, 18286, 18340, 18556,  
 18610, 18718, 18934, 18988, 19042, 19150, 19204, 19420, 19474, 19582, 19636,  
 19798, 19906, 20014, 20068, 20284, 20338, 20446, 20500, 20662, 20716, 20770,  
 20878, 21148, 21202, 21310, 21364, 21526, 21634, 21742, 21796, 22012, 22066,  
 22174, 22390, 22444, 22606, 22660, 22876, 22930, 23038, 23254, 23362, 23470,  
 23524, 23740, 23794, 23902, 23956, 24118, 24172, 24226, 24334, 24388, 24604,  
 24658, 24766, 24820, 24982, 25090, 25198, 25252, 25468, 25522, 25630, 25846,  
 25900, 25954, 26062, 26116, 26332, 26386, 26494, 26548, 26710, 26818, 26926,  
 26980, 27196, 27250, 27358, 27412, 27574, 27628, 27682, 27790, 27844, 28060,  
 28114, 28222, 28276, 28438, 28546, 28654, 28708, 28924, 28978, 29086, 29302,  
 29356, 29518, 29572, 29788, 29842, 29950, 30166, 30274, 30382, 30436, 30652,  
 30706, 30814, 30868, 31030, 31084, 31138, 31246, 31300, 31516, 31570, 31678,  
 31732, 31894, 32002, 32110, 32164, 32380, 32434, 32542, 32758, 32812, 32866,  
 32974, 33028, 33244, 33298, 33406, 33460, 33622, 33730, 33838, 33892, 34108,  
 34162, 34270, 34324, 34486, 34540, 34594, 34702, 34972, 35026, 35134, 35188,  
 35350, 35458, 35566, 35620, 35836, 35890, 35998, 36214, 36268, 36430, 36484,  
 36700, 36754, 36862, 37078, 37186, 37294, 37348, 37564, 37618, 37726, 37780,  
 37942, 37996, 38050, 38158, 38212, 38428, 38482, 38590, 38644, 38806, 38914,  
 39022, 39076, 39292, 39346, 39454, 39670, 39724, 39778, 39886, 39940, 40156,  
 40210, 40318, 40372, 40534, 40642, 40750, 40804, 41020, 41074, 41182, 41236,

41 398, 41 452, 41 506, 41 614, 41 668, 41 884, 41 938, 42 046, 42 100, 42 262, 42 370,  
 42 478, 42 532, 42 748, 42 802, 42 910, 43 126, 43 180, 43 342, 43 396, 43 612, 43 666,  
 43 774, 43 990, 44 098, 44 206, 44 260, 44 476, 44 530, 44 638, 44 692, 44 854, 44 908,  
 44 962, 45 070, 45 124, 45 340, 45 394, 45 502, 45 556, 45 718, 45 826, 45 934, 45 988,  
 46 204, 46 258, 46 366, 46 582, 46 636, 46 690, 46 798, 46 852, 47 068, 47 122, 47 230,  
 47 284, 47 446, 47 554, 47 662, 47 716, 47 932, 47 986, 48 094, 48 148, 48 310, 48 364,  
 48 418, 48 526, 48 796, 48 850, 48 958, 49 012, 49 174, 49 282, 49 390, 49 444, 49 660,  
 49 714, 49 822, 50 038, 50 092, 50 254, 50 308, 50 524, 50 578, 50 686, 50 902, 51 010,  
 51 118, 51 172, 51 388, 51 442, 51 550, 51 604, 51 766, 51 820, 51 874, 51 982, 52 036,  
 52 252, 52 306, 52 414, 52 468, 52 630, 52 738, 52 846, 52 900, 53 116, 53 170, 53 278,  
 53 494, 53 548, 53 602, 53 710, 53 764, 53 980, 54 034, 54 142, 54 196, 54 358, 54 466,  
 54 574, 54 628, 54 844, 54 898, 55 006, 55 222, 55 276, 55 330, 55 438, 55 492, 55 708,  
 55 762, 55 870, 55 924, 56 086, 56 194, 56 302, 56 356, 56 572, 56 626, 56 734, 56 950,  
 57 004, 57 166, 57 220, 57 436, 57 490, 57 598, 57 814, 57 922, 58 030, 58 084, 58 300,  
 58 354, 58 462, 58 516, 58 678, 58 732, 58 786, 58 894, 58 948, 59 164, 59 218, 59 326,  
 59 380, 59 542, 59 650, 59 758, 59 812, 60 028, 60 082, 60 190, 60 406, 60 460, 60 514,  
 60 622, 60 676, 60 892, 60 946, 61 054, 61 108, 61 270, 61 378, 61 486, 61 540, 61 756,  
 61 810, 61 918, 61 972, 62 134, 62 188, 62 242, 62 350, 62 620, 62 674, 62 782, 62 836,  
 62 998, 63 106, 63 214, 63 268, 63 484, 63 538, 63 646, 63 862, 63 916, 64 078, 64 132,  
 64 348, 64 402, 64 510, 64 726, 64 834, 64 942, 64 996, 65 212, 65 266, 65 374, 65 428,  
 65 590, 65 644, 65 698, 65 806, 65 860, 66 076, 66 130, 66 238, 66 292, 66 454, 66 562,  
 66 670, 66 724, 66 940, 66 994, 67 102, 67 318, 67 372, 67 426, 67 534, 67 588, 67 804,  
 67 858, 67 966, 68 020, 68 182, 68 290, 68 398, 68 452, 68 668, 68 722, 68 830, 68 884,  
 69 046, 69 100, 69 154, 69 262, 69 316, 69 532, 69 586, 69 694, 69 748, 69 910, 70 018,  
 70 126, 70 180, 70 396, 70 450, 70 558, 70 774, 70 828, 70 990, 71 044, 71 260, 71 314,  
 71 422, 71 638, 71 746, 71 854, 71 908, 72 124, 72 178, 72 286, 72 340, 72 502, 72 556,  
 72 610, 72 718, 72 772, 72 988, 73 042, 73 150, 73 204, 73 366, 73 474, 73 582, 73 636},  
 {94, 148, 310, 364, 418, 472, 526, 580, 688, 796, 850, 958, 1012, 1174, 1282, 1336,  
 1390, 1444, 1552, 1660, 1714, 1822, 2038, 2092, 2146, 2254, 2308, 2416, 2524,  
 2578, 2632, 2686, 2740, 2902, 3010, 3064, 3118, 3172, 3388, 3442, 3550, 3604,  
 3766, 3820, 3874, 3928, 3982, 4252, 4306, 4360, 4414, 4468, 4630, 4738, 4792,  
 4846, 4900, 5008, 5116, 5170, 5278, 5494, 5548, 5710, 5764, 5872, 5980, 6034,  
 6088, 6142, 6358, 6466, 6520, 6574, 6628, 6736, 6844, 6898, 7006, 7060, 7222,  
 7276, 7330, 7384, 7438, 7492, 7600, 7708, 7762, 7816, 7870, 7924, 8086, 8194,  
 8248, 8302, 8356, 8464, 8572, 8626, 8734, 8950, 9004, 9058, 9166, 9220, 9328,  
 9436, 9490, 9544, 9598, 9652, 9814, 9922, 9976, 10 030, 10 084, 10 192, 10 300,  
 .....

10 354, 10 462, 10 516, 10 678, 10 732, 10 786, 10 840, 10 894, 10 948, 11 164, 11 218,  
 11 272, 11 326, 11 380, 11 542, 11 650, 11 704, 11 758, 11 812, 11 920, 12 028, 12 082,  
 12 190, 12 406, 12 460, 12 622, 12 676, 12 784, 12 892, 12 946, 13 000, 13 054, 13 270,  
 13 378, 13 432, 13 486, 13 540, 13 756, 13 810, 13 918, 13 972, 14 134, 14 188, 14 242,  
 14 296, 14 350, 14 404, 14 512, 14 620, 14 674, 14 728, 14 782, 14 836, 14 998, 15 106,  
 15 160, 15 214, 15 268, 15 376, 15 484, 15 538, 15 646, 15 862, 15 916, 15 970, 16 078,  
 16 132, 16 240, 16 348, 16 402, 16 456, 16 510, 16 564, 16 726, 16 834, 16 888, 16 942,  
 16 996, 17 104, 17 212, 17 266, 17 374, 17 428, 17 590, 17 644, 17 698, 17 752, 17 806,  
 18 076, 18 130, 18 184, 18 238, 18 292, 18 454, 18 562, 18 616, 18 670, 18 724, 18 832,  
 18 940, 18 994, 19 102, 19 318, 19 372, 19 534, 19 588, 19 696, 19 804, 19 858, 19 912,  
 19 966, 20 182, 20 290, 20 344, 20 398, 20 452, 20 560, 20 668, 20 722, 20 830, 20 884,  
 21 046, 21 100, 21 154, 21 208, 21 262, 21 316, 21 424, 21 532, 21 586, 21 640, 21 694,  
 21 748, 21 910, 22 018, 22 072, 22 126, 22 180, 22 396, 22 450, 22 558, 22 774, 22 828,  
 22 882, 22 990, 23 044, 23 152, 23 260, 23 314, 23 368, 23 422, 23 476, 23 638, 23 746,  
 23 800, 23 854, 23 908, 24 016, 24 124, 24 178, 24 286, 24 502, 24 556, 24 610, 24 664,  
 24 718, 24 772, 24 988, 25 042, 25 096, 25 150, 25 204, 25 366, 25 474, 25 528, 25 582,  
 25 636, 25 744, 25 852, 25 906, 26 014, 26 230, 26 284, 26 446, 26 500, 26 608, 26 716,  
 26 770, 26 824, 26 878, 27 094, 27 202, 27 256, 27 310, 27 364, 27 580, 27 634, 27 742,  
 27 796, 27 958, 28 012, 28 066, 28 120, 28 174, 28 228, 28 336, 28 444, 28 498, 28 606,  
 28 660, 28 822, 28 930, 28 984, 29 038, 29 092, 29 200, 29 308, 29 362, 29 470, 29 686,  
 29 740, 29 794, 29 902, 29 956, 30 064, 30 172, 30 226, 30 280, 30 334, 30 388, 30 550,  
 30 658, 30 712, 30 766, 30 820, 31 036, 31 090, 31 198, 31 252, 31 414, 31 468, 31 522,  
 31 576, 31 630, 31 900, 31 954, 32 008, 32 062, 32 116, 32 278, 32 386, 32 440, 32 494,  
 32 548, 32 656, 32 764, 32 818, 32 926, 33 142, 33 196, 33 358, 33 412, 33 520, 33 628,  
 33 682, 33 736, 33 790, 34 006, 34 114, 34 168, 34 222, 34 276, 34 384, 34 492, 34 546,  
 34 654, 34 708, 34 870, 34 924, 34 978, 35 032, 35 086, 35 140, 35 248, 35 356, 35 410,  
 35 464, 35 518, 35 572, 35 734, 35 842, 35 896, 35 950, 36 004, 36 112, 36 220, 36 274,  
 36 382, 36 598, 36 652, 36 706, 36 814, 36 868, 36 976, 37 084, 37 138, 37 192, 37 246,  
 37 300, 37 462, 37 570, 37 624, 37 678, 37 732, 37 840, 37 948, 38 002, 38 110, 38 164,  
 38 326, 38 380, 38 434, 38 488, 38 542, 38 596, 38 812, 38 866, 38 920, 38 974, 39 028,  
 39 190, 39 298, 39 352, 39 406, 39 460, 39 568, 39 676, 39 730, 39 838, 40 054, 40 108,  
 40 270, 40 324, 40 432, 40 540, 40 594, 40 648, 40 702, 40 918, 41 026, 41 080, 41 134,  
 41 188, 41 404, 41 458, 41 566, 41 620, 41 782, 41 836, 41 890, 41 944, 41 998, 42 052,  
 42 160, 42 268, 42 322, 42 376, 42 430, 42 484, 42 646, 42 754, 42 808, 42 862, 42 916,  
 43 024, 43 132, 43 186, 43 294, 43 510, 43 564, 43 618, 43 726, 43 780, 43 888, 43 996,  
 44 050, 44 104, 44 158, 44 212, 44 374, 44 482, 44 536, 44 590, 44 644, 44 752, 44 860,  
 44 914. 45 022. 45 076. 45 238. 45 292. 45 346. 45 400. 45 454. 45 724. 45 778. 45 832.

45 886, 45 940, 46 102, 46 210, 46 264, 46 318, 46 372, 46 480, 46 588, 46 642, 46 750,  
 46 966, 47 020, 47 182, 47 236, 47 344, 47 452, 47 506, 47 560, 47 614, 47 830, 47 938,  
 47 992, 48 046, 48 100, 48 316, 48 370, 48 478, 48 532, 48 694, 48 748, 48 802, 48 856,  
 48 910, 48 964, 49 072, 49 180, 49 234, 49 288, 49 342, 49 396, 49 558, 49 666, 49 720,  
 49 774, 49 828, 49 936, 50 044, 50 098, 50 206, 50 422, 50 476, 50 530, 50 638, 50 692,  
 50 800, 50 908, 50 962, 51 016, 51 070, 51 124, 51 286, 51 394, 51 448, 51 502, 51 556,  
 51 664, 51 772, 51 826, 51 934, 51 988, 52 150, 52 204, 52 258, 52 312, 52 366, 52 420,  
 52 636, 52 690, 52 744, 52 798, 52 852, 53 014, 53 122, 53 176, 53 230, 53 284, 53 392,  
 53 500, 53 554, 53 662, 53 878, 53 932, 54 094, 54 148, 54 256, 54 364, 54 418, 54 472,  
 54 526, 54 742, 54 850, 54 904, 54 958, 55 012, 55 228, 55 282, 55 390, 55 444, 55 606,  
 55 660, 55 714, 55 768, 55 822, 55 876, 55 984, 56 092, 56 146, 56 254, 56 308, 56 470,  
 56 578, 56 632, 56 686, 56 740, 56 848, 56 956, 57 010, 57 118, 57 334, 57 388, 57 442,  
 57 550, 57 604, 57 712, 57 820, 57 874, 57 928, 57 982, 58 036, 58 198, 58 306, 58 360,  
 58 414, 58 468, 58 684, 58 738, 58 846, 58 900, 59 062, 59 116, 59 170, 59 224, 59 278,  
 59 548, 59 602, 59 656, 59 710, 59 764, 59 926, 60 034, 60 088, 60 142, 60 196, 60 304,  
 60 412, 60 466, 60 574, 60 790, 60 844, 61 006, 61 060, 61 168, 61 276, 61 330, 61 384,  
 61 438, 61 654, 61 762, 61 816, 61 870, 61 924, 62 032, 62 140, 62 194, 62 302, 62 356,  
 62 518, 62 572, 62 626, 62 680, 62 734, 62 788, 62 896, 63 004, 63 058, 63 112, 63 166,  
 63 220, 63 382, 63 490, 63 544, 63 598, 63 652, 63 760, 63 868, 63 922, 64 030, 64 246,  
 64 300, 64 354, 64 462, 64 516, 64 624, 64 732, 64 786, 64 840, 64 894, 64 948, 65 110,  
 65 218, 65 272, 65 326, 65 380, 65 488, 65 596, 65 650, 65 758, 65 812, 65 974, 66 028,  
 66 082, 66 136, 66 190, 66 244, 66 460, 66 514, 66 568, 66 622, 66 676, 66 838, 66 946,  
 67 000, 67 054, 67 108, 67 216, 67 324, 67 378, 67 486, 67 702, 67 756, 67 918, 67 972,  
 68 080, 68 188, 68 242, 68 296, 68 350, 68 566, 68 674, 68 728, 68 782, 68 836, 69 052,  
 69 106, 69 214, 69 268, 69 430, 69 484, 69 538, 69 592, 69 646, 69 700, 69 808, 69 916,  
 69 970, 70 024, 70 078, 70 132, 70 294, 70 402, 70 456, 70 510, 70 564, 70 672, 70 780,  
 70 834, 70 942, 71 158, 71 212, 71 266, 71 374, 71 428, 71 536, 71 644, 71 698, 71 752,  
 71 806, 71 860, 72 022, 72 130, 72 184, 72 238, 72 292, 72 400, 72 508, 72 562, 72 670,  
 72 724, 72 886, 72 940, 72 994, 73 048, 73 102, 73 372, 73 426, 73 480, 73 534, 73 588},  
 {214, 322, 430, 484, 700, 754, 862, 916, 1078, 1132, 1186, 1294, 1348, 1564, 1618,  
 1726, 1780, 1942, 2050, 2158, 2212, 2428, 2482, 2590, 2806, 2860, 2914, 3022,  
 3076, 3292, 3346, 3454, 3508, 3670, 3778, 3886, 3940, 4156, 4210, 4318, 4372,  
 4534, 4588, 4642, 4750, 4804, 5020, 5074, 5182, 5236, 5398, 5506, 5614, 5668,  
 5884, 5938, 6046, 6262, 6316, 6478, 6532, 6748, 6802, 6910, 7126, 7234, 7342,  
 7396, 7612, 7666, 7774, 7828, 7990, 8044, 8098, 8206, 8260, 8476, 8530, 8638,  
 8692, 8854, 8962, 9070, 9124, 9340, 9394, 9502, 9718, 9772, 9826, 9934, 9988,

10 204, 10 258, 10 366, 10 420, 10 582, 10 690, 10 798, 10 852, 11 068, 11 122, 11 230,  
 11 284, 11 446, 11 500, 11 554, 11 662, 11 932, 11 986, 12 094, 12 148, 12 310, 12 418,  
 12 526, 12 580, 12 796, 12 850, 12 958, 13 174, 13 228, 13 390, 13 444, 13 660, 13 714,  
 13 822, 14 038, 14 146, 14 254, 14 308, 14 524, 14 578, 14 686, 14 740, 14 902, 14 956,  
 15 010, 15 118, 15 172, 15 388, 15 442, 15 550, 15 604, 15 766, 15 874, 15 982, 16 036,  
 16 252, 16 306, 16 414, 16 630, 16 684, 16 738, 16 846, 16 900, 17 116, 17 170, 17 278,  
 17 332, 17 494, 17 602, 17 710, 17 764, 17 980, 18 034, 18 142, 18 358, 18 412, 18 466,  
 18 574, 18 628, 18 844, 18 898, 19 006, 19 060, 19 222, 19 330, 19 438, 19 492, 19 708,  
 19 762, 19 870, 20 086, 20 140, 20 302, 20 356, 20 572, 20 626, 20 734, 20 950, 21 058,  
 21 166, 21 220, 21 436, 21 490, 21 598, 21 652, 21 814, 21 868, 21 922, 22 030, 22 084,  
 22 300, 22 354, 22 462, 22 516, 22 678, 22 786, 22 894, 22 948, 23 164, 23 218, 23 326,  
 23 542, 23 596, 23 650, 23 758, 23 812, 24 028, 24 082, 24 190, 24 244, 24 406, 24 514,  
 24 622, 24 676, 24 892, 24 946, 25 054, 25 108, 25 270, 25 324, 25 378, 25 486, 25 756,  
 25 810, 25 918, 25 972, 26 134, 26 242, 26 350, 26 404, 26 620, 26 674, 26 782, 26 998,  
 27 052, 27 214, 27 268, 27 484, 27 538, 27 646, 27 862, 27 970, 28 078, 28 132, 28 348,  
 28 402, 28 510, 28 564, 28 726, 28 780, 28 834, 28 942, 28 996, 29 212, 29 266, 29 374,  
 29 428, 29 590, 29 698, 29 806, 29 860, 30 076, 30 130, 30 238, 30 454, 30 508, 30 562,  
 30 670, 30 724, 30 940, 30 994, 31 102, 31 156, 31 318, 31 426, 31 534, 31 588, 31 804,  
 31 858, 31 966, 32 020, 32 182, 32 236, 32 290, 32 398, 32 452, 32 668, 32 722, 32 830,  
 32 884, 33 046, 33 154, 33 262, 33 316, 33 532, 33 586, 33 694, 33 910, 33 964, 34 126,  
 34 180, 34 396, 34 450, 34 558, 34 774, 34 882, 34 990, 35 044, 35 260, 35 314, 35 422,  
 35 476, 35 638, 35 692, 35 746, 35 854, 35 908, 36 124, 36 178, 36 286, 36 340, 36 502,  
 36 610, 36 718, 36 772, 36 988, 37 042, 37 150, 37 366, 37 420, 37 474, 37 582, 37 636,  
 37 852, 37 906, 38 014, 38 068, 38 230, 38 338, 38 446, 38 500, 38 716, 38 770, 38 878,  
 38 932, 39 094, 39 148, 39 202, 39 310, 39 580, 39 634, 39 742, 39 796, 39 958, 40 066,  
 40 174, 40 228, 40 444, 40 498, 40 606, 40 822, 40 876, 41 038, 41 092, 41 308, 41 362,  
 41 470, 41 686, 41 794, 41 902, 41 956, 42 172, 42 226, 42 334, 42 388, 42 550, 42 604,  
 42 658, 42 766, 42 820, 43 036, 43 090, 43 198, 43 252, 43 414, 43 522, 43 630, 43 684,  
 43 900, 43 954, 44 062, 44 278, 44 332, 44 386, 44 494, 44 548, 44 764, 44 818, 44 926,  
 44 980, 45 142, 45 250, 45 358, 45 412, 45 628, 45 682, 45 790, 45 844, 46 006, 46 060,  
 46 114, 46 222, 46 276, 46 492, 46 546, 46 654, 46 708, 46 870, 46 978, 47 086, 47 140,  
 47 356, 47 410, 47 518, 47 734, 47 788, 47 950, 48 004, 48 220, 48 274, 48 382, 48 598,  
 48 706, 48 814, 48 868, 49 084, 49 138, 49 246, 49 300, 49 462, 49 516, 49 570, 49 678,  
 49 732, 49 948, 50 002, 50 110, 50 164, 50 326, 50 434, 50 542, 50 596, 50 812, 50 866,  
 50 974, 51 190, 51 244, 51 298, 51 406, 51 460, 51 676, 51 730, 51 838, 51 892, 52 054,  
 52 162, 52 270, 52 324, 52 540, 52 594, 52 702, 52 756, 52 918, 52 972, 53 026, 53 134,  
 53 188, 53 450, 53 504, 53 612, 53 720, 53 774, 53 882, 54 098, 54 152, 54 260, 54 314, 54 422

```

53 404, 53 458, 53 566, 53 620, 53 782, 53 890, 53 998, 54 052, 54 268, 54 322, 54 430,
54 646, 54 700, 54 862, 54 916, 55 132, 55 186, 55 294, 55 510, 55 618, 55 726, 55 780,
55 996, 56 050, 56 158, 56 212, 56 374, 56 428, 56 482, 56 590, 56 644, 56 860, 56 914,
57 022, 57 076, 57 238, 57 346, 57 454, 57 508, 57 724, 57 778, 57 886, 58 102, 58 156,
58 210, 58 318, 58 372, 58 588, 58 642, 58 750, 58 804, 58 966, 59 074, 59 182, 59 236,
59 452, 59 506, 59 614, 59 668, 59 830, 59 884, 59 938, 60 046, 60 100, 60 316, 60 370,
60 478, 60 532, 60 694, 60 802, 60 910, 60 964, 61 180, 61 234, 61 342, 61 558, 61 612,
61 774, 61 828, 62 044, 62 098, 62 206, 62 422, 62 530, 62 638, 62 692, 62 908, 62 962,
63 070, 63 124, 63 286, 63 340, 63 394, 63 502, 63 556, 63 772, 63 826, 63 934, 63 988,
64 150, 64 258, 64 366, 64 420, 64 636, 64 690, 64 798, 65 014, 65 068, 65 122, 65 230,
65 284, 65 500, 65 554, 65 662, 65 716, 65 878, 65 986, 66 094, 66 148, 66 364, 66 418,
66 526, 66 580, 66 742, 66 796, 66 850, 66 958, 67 228, 67 282, 67 390, 67 444, 67 606,
67 714, 67 822, 67 876, 68 092, 68 146, 68 254, 68 470, 68 524, 68 686, 68 740, 68 956,
69 010, 69 118, 69 334, 69 442, 69 550, 69 604, 69 820, 69 874, 69 982, 70 036, 70 198,
70 252, 70 306, 70 414, 70 468, 70 684, 70 738, 70 846, 70 900, 71 062, 71 170, 71 278,
71 332, 71 548, 71 602, 71 710, 71 926, 71 980, 72 034, 72 142, 72 196, 72 412, 72 466,
72 574, 72 628, 72 790, 72 898, 73 006, 73 060, 73 276, 73 330, 73 438, 73 654, 73 708} }

```

The grid for c432k is printed for k=1 only, because it is just the combination of c81k and c351k.

```

In[136]:= Grid[
  Prepend[
    ReplacePart[cNk[c432k, 1], {{1, 1} → "0: T>0 c32", {2, 1} → "1: rightward c432"}],
    {"t>k right nested", "432·13k-1 congruence classes", "cardinality", "periodicity"}],
  Dividers → {False, {True, True}}, Alignment → Left]

```



| $t_{\geq k}$ | right nested | $432 \cdot 13^{k-1}$ | congruence classes                                                                                                                                                                                                                                                                                                                                                                                                                                                                                                                                                                                                                                                                                                                                                                                                                                                                                                                                                                                                                                                                                                                                                                                                                                                                                                                                                                                                                                                                                                                                                                                                                                                                                                                                                                                                                                                                                                                                                                                                                                                                                                                                                                                                                                                                                                                                                                                                                                                                                                                                                                                  | cardinality | periodicity |
|--------------|--------------|----------------------|-----------------------------------------------------------------------------------------------------------------------------------------------------------------------------------------------------------------------------------------------------------------------------------------------------------------------------------------------------------------------------------------------------------------------------------------------------------------------------------------------------------------------------------------------------------------------------------------------------------------------------------------------------------------------------------------------------------------------------------------------------------------------------------------------------------------------------------------------------------------------------------------------------------------------------------------------------------------------------------------------------------------------------------------------------------------------------------------------------------------------------------------------------------------------------------------------------------------------------------------------------------------------------------------------------------------------------------------------------------------------------------------------------------------------------------------------------------------------------------------------------------------------------------------------------------------------------------------------------------------------------------------------------------------------------------------------------------------------------------------------------------------------------------------------------------------------------------------------------------------------------------------------------------------------------------------------------------------------------------------------------------------------------------------------------------------------------------------------------------------------------------------------------------------------------------------------------------------------------------------------------------------------------------------------------------------------------------------------------------------------------------------------------------------------------------------------------------------------------------------------------------------------------------------------------------------------------------------------------|-------------|-------------|
| 0:           | $T_{\geq 0}$ | c32                  | {16, 88, 160, 232, 256, 4, 22, 34, 40, 52, 58, 70, 76, 94, 106, 112, 124, 130, 142, 148, 166, 178, 184, 196, 202, 214, 220, 238, 250, 268, 274, 286}                                                                                                                                                                                                                                                                                                                                                                                                                                                                                                                                                                                                                                                                                                                                                                                                                                                                                                                                                                                                                                                                                                                                                                                                                                                                                                                                                                                                                                                                                                                                                                                                                                                                                                                                                                                                                                                                                                                                                                                                                                                                                                                                                                                                                                                                                                                                                                                                                                                | $2^5$       | 288         |
| 1:           | rightward    | c432                 | {4, 58, 112, 166, 220, 274, 328, 382, 436, 490, 598, 652, 706, 760, 814, 868, 922, 976, 1030, 1084, 1138, 1192, 1246, 1300, 1354, 1462, 1516, 1570, 1624, 1678, 1732, 1786, 1840, 1894, 1948, 2002, 2056, 2110, 2164, 2218, 2326, 2380, 2434, 2488, 2542, 2596, 2650, 2704, 2758, 2812, 2866, 2920, 2974, 3028, 3082, 3190, 3244, 3298, 3352, 3406, 3460, 3514, 3568, 3622, 3676, 3730, 3784, 3838, 3892, 3946, 4054, 4108, 4162, 4216, 4270, 4324, 4378, 4432, 4486, 4540, 4594}, {70, 124, 178, 286, 340, 394, 502, 556, 610, 718, 772, 826, 934, 988, 1042, 1150, 1204, 1258, 1366, 1420, 1474, 1582, 1636, 1690, 1798, 1852, 1906, 2014, 2068, 2122, 2230, 2284, 2338, 2446, 2500, 2554, 2662, 2716, 2770, 2878, 2932, 2986, 3094, 3148, 3202, 3310, 3364, 3418, 3526, 3580, 3634, 3742, 3796, 3850, 3958, 4012, 4066, 4174, 4228, 4282, 4390, 4444, 4498, 4606}, {22, 76, 130, 184, 238, 292, 346, 400, 454, 508, 562, 616, 670, 724, 778, 886, 940, 994, 1048, 1102, 1156, 1210, 1264, 1318, 1372, 1426, 1480, 1534, 1588, 1642, 1750, 1804, 1858, 1912, 1966, 2020, 2074, 2128, 2182, 2236, 2290, 2344, 2398, 2452, 2506, 2614, 2668, 2722, 2776, 2830, 2884, 2938, 2992, 3046, 3100, 3154, 3208, 3262, 3316, 3370, 3478, 3532, 3586, 3640, 3694, 3748, 3802, 3856, 3910, 3964, 4018, 4072, 4126, 4180, 4234, 4342, 4396, 4450, 4504, 4558}, {34, 142, 196, 250, 358, 412, 466, 574, 628, 682, 790, 844, 898, 1006, 1060, 1114, 1222, 1276, 1330, 1438, 1492, 1546, 1654, 1708, 1762, 1870, 1924, 1978, 2086, 2140, 2194, 2302, 2356, 2410, 2518, 2572, 2626, 2734, 2788, 2842, 2950, 3004, 3058, 3166, 3220, 3274, 3382, 3436, 3490, 3598, 3652, 3706, 3814, 3868, 3922, 4030, 4084, 4138, 4246, 4300, 4354, 4462, 4516, 4570}, {40, 94, 148, 202, 310, 364, 418, 472, 526, 580, 634, 688, 742, 796, 850, 904, 958, 1012, 1066, 1174, 1228, 1282, 1336, 1390, 1444, 1498, 1552, 1606, 1660, 1714, 1768, 1822, 1876, 1930, 2038, 2092, 2146, 2200, 2254, 2308, 2362, 2416, 2470, 2524, 2578, 2632, 2686, 2740, 2794, 2902, 2956, 3010, 3064, 3118, 3172, 3226, 3280, 3334, 3388, 3442, 3496, 3550, 3604, 3658, 3766, 3820, 3874, 3928, 3982, 4036, 4090, 4144, 4198, 4252, 4306, 4360, 4414, 4468, 4522}, {52, 106, 214, 268, 322, 430, 484, 538, 646, 700, 754, 862, 916, 970, 1078, 1132, 1186, 1294, 1348, 1402, 1510, 1564, 1618, 1726, 1780, 1834, 1942, 1996, 2050, 2158, 2212, 2266, 2374, 2428, 2482, 2590, 2644, 2698, 2806, 2860, 2914, 3022, 3076, 3130, 3238, 3292, 3346, 3454, 3508, 3562, 3670, 3724, 3778, 3886, 3940, 3994, 4102, 4156, 4210, 4318, 4372, 4426, 4534, 4588}} | $2^4 3^3$   | 4608        |

Out[136]=

## Conjugated upward and rightward functions for nested and disjoint subtrees

$\text{rj}[n, j] = U^j R_0 U^{-j}[n]$  defines the reconnection function in the reconnected tree  $T_{\geq j}$  as the Skolem-Noether map  $U^j R_0 U^{-j}$  of the rightward function  $R_0$  (with  $k=1$  rightward iterations).

see, for example, how  $\text{rj}[\#, 1]$  connects numbers to their conjugated rightward descendant in the nested upward subtree  $T_{\geq 1}$  (main text Figure 4, top left)

```
In[137]:= rj[n_, j_] := Nest[u, r[Nest[d, n, j]], j];
Rule[\#, rj[\#, 1]] & /@ {256, 160, 1024, 2560}
```

```
Out[138]:= {256 → 160, 160 → 832, 1024 → 5440, 2560 → 1696}
```

$\text{uk}[n, k] = R^k U_0 R^{-k}[n]$  defines the reconnection function in the reconnected tree  $T_{\geq 0, k}$  as the Skolem-Noether map  $R^k U_0 R^{-k}$  of the upward function  $U_0$  (with  $k=1$  rightward iterations);

see, for example, how  $\text{uk}[\#, 1]$  connects numbers to their conjugated upward descendant in the nested rightward subtree  $t_{\geq 1} = T_0$  (main text Figure 4, top left)

```
In[139]:= uk[n_, k_] := rk[u[lk[n, k]], k];
Rule[\#, uk[\#, 1]] & /@ {40, 52, 340, 106}
```

```
Out[140]:= {40 → 340, 52 → 106, 340 → 682, 106 → 13 648}
```

$\text{uj1}[n, j]$  gives double conjugate upward child  $U_{j,1}$  of  $n$  in upward cotree  $T_j$

```
In[141]:= uj1[n_, j_] := uj[r[u[lk[dj[n, j], 1]], j]
```

```
In[142]:= uj1[2176, 2]
```

```
Out[142]:= 283 648
```

$\text{rk1}[n, j]$  gives double conjugate rightward child  $R_{k,1}$  of  $n$  in rightward cotree  $t_n$

```
In[143]:= rk1[n_, k_] := rk[u[r[dj[lk[n, k], 1]], k]
```

```
In[144]:= rk1[18 196, 2]
```

```
Out[144]:= 48 208
```

$\text{ujk}[n, j, k]$  connects to conjugated upward descendants in disjoint upward subtrees;

see for example, how  $\text{ujk}[\#]$  connects numbers in rightward trees  $t_1$ ,  $t_2$  and  $t_3$  (main text Figure 4)

```
In[145]:= ujk[n_, j_, k_] := rk[uj[lk[n, k], j], k];
Rule[#, ujk[#, 1, 1]] & /@ {340, 904, 1204}
```

```
Out[146]:= {340 → 682, 904 → 7252, 1204 → 2410}
```

$\text{rrj}[n, j] = U^j R_0 U^{-j}[n]$  defines the iterated reconnection function in the reconnected tree  $T_{\geq j}$  as the Skolem-Noether map  $U^j R_0^k U^{-j}$  of the iterated rightward function  $R_0^k$  with k rightward iterations;  
see for example, how  $\text{rrj}[\#, 2, 1]$  connects numbers in the upward tree  $T_2$  (main text Figure 3) to conjugated rightward descendants

```
In[147]:= rrj[n_, j_, k_] := uj[rk[dj[n, j], k], j];
Rule[#, rrj[#, 2, 1]] & /@ {1024, 10240}
```

```
Out[148]:= {1024 → 2560, 10240 → 6784}
```

$\text{urj}[n, j]$  is the conjugated upward function in  $T_j$ , first upward iteration;  
see for example conjugated upward children by  $\text{urj}[\#, 3]$  in the upward tree  $T_3$  (main text Figure 3)

```
In[149]:= urj[n_, j_] := uj[r[u[l[dj[n, j]]]], j];
Rule[#, urj[#, 3]] & /@ {1024, 10240}
```

```
Out[150]:= {1024 → 10240, 10240 → 348160}
```

upward function in  $T_j$ ,  $i$ 'th upward iteration;  
see for example conjugated upward grandchildren by  $\text{urj}[\#, 3, 2]$  in the upward tree  $T_3$  (main text Figure 3)

```
In[151]:= urji[n_, j_, i_] := uj[r[uj[l[dj[n, j]], i]], j];
Rule[#, urji[#, 3, 2]] & /@ {1024, 10240}
```

```
Out[152]:= {1024 → 348160, 10240 → 698368}
```

$\text{gj}[n, j]$  gives for n in tree  $T_{\geq j}$  the pair of, first, the rightward reconnected child  $R_j[n]$  and, next, the upward child  $U[n]$

```
In[153]:= gj[n_, j_] := List[rj[n, j], u[n]]
```

## 5. Plots of the binary tree and its subtrees

### Auxiliary functions to plot trees

extnSj[n] is a help function that extracts a numerical n from a string "n \n S(n)"

```
In[154]:= extnSj[str_] := If[StringQ[str],
  StringSplit[str, "\nS"] // First // ToExpression, StringSplit[First[str], "\nS"] // First // ToExpression];
```

invisSj[n,j] is a help function that turns nodes in tree  $T_{\geq j}$  white/invisible that do not belong to node subset  $S_j$  that will depart next

```
In[155]:= invisSj[n_, j_] := If[upjQ[extnSj[n], j], Style[n, White], n];
```

invisSgtJ[n,j] is a help function that turns nodes in tree  $T_{\geq j}$  white/invisible that do not belong to node subset  $S_{\geq j+1}$  that will remain; nodes from subset  $S_j$  become invisible

```
In[156]:= invisSgtJ[n_, j_] := If[upjQ[extnSj[n], j], n, Style[n, White]];
```

nExtract[n] extracts the number from a string

```
In[157]:= nExtract[n_] := If[NumberQ[n], n, If[StringQ[n], First[n], First[First[n]]]];
```

addnSj[n] is a help function that adds the upward subset Sj or sj to which n belongs on a new line of a string

```
In[158]:= addnSj[n_] := If[upQ[n], (ToString[n] <> "\nS" <> ToString[sJ[n]]), (ToString[n] <> "\ns" <> ToString[s0K[n]])];
```

addnS0k[n] is a help function that adds the rightward subset S0k to which n belongs on a new line of a string

```
In[159]:= addnS0k[n_] := ToString[n] <> "\ns" <> ToString[s0K[n]];
```

extnSj[n] is a help function that extracts a numerical n from a string with \nS or \ns

```
In[160]:= extnSj[str_] := Module[{string = If[StringQ[str], str, First[str]], string2, string3},
  If[StringContainsQ[string, "S"], StringSplit[str, "\nS"], StringSplit[str, "\ns"]] // First // ToExpression]
```

```
In[161]:= testn[n_] := {addnSj[n], "-----", extnSj[addnSj[n]]}
```

```
In[162]:= testn[4]
```

```
Out[162]:= {4
           s0, -----, 4}
```

extnS0k[n] is a help function that extracts a numerical n from a string with \nt

```
In[163]:= extnS0k[str_] := If[StringQ[str],
    StringSplit[str, "\ns"] // First // ToExpression, StringSplit[First[str], "\ns"] // First // ToExpression];
```

rjQ[a,b,j] tests whether in tree  $T_j$  for  $\{a \rightarrow b\}$  holds  $b = R_j(a) = U^j R U^{-j}(a)$ , i.e. whether b is reconnected by function  $R_j$ , whether  $b=R$

```
In[164]:= rjQ[n1_, n2_, j_] := If[sJ[n2] != j, False, uj[1[dj[n2, j]]], j] == n1]
```

ukQ[a,b,j] tests whether in tree  $T_{0,k}$  for  $\{a \rightarrow b\}$  holds  $b = R_j(a) = R^k U R^{-k}(a)$ , i.e. whether b is reconnected by function  $U_k$

```
In[165]:= ukQ[n1_, n2_, k_] := If[s0K[n2] != k, False, rk[u[1k[n1, k]]], k] == n2]
```

## Labels of edge sets and (sub)trees

The grid below shows the names of the functions to generate the edges that are used in the functions to generate a plot of the corresponding sub(tree).

$T_{\geq j}$  = TreeUPge(0)[j,nk],

$T_j$  = TreeUPeq[j,nk],

$t_{\geq k}$  = TreeRIge[k,nk],

$t_k$  = TreeRI[k,nk],

in which j is the j'th generation of upward successors, k is the k'th generation of rightward successors, and nk is the number of levels of binary splits starting from the root to be generated / plotted.

```
In[166]:= Grid[{{"", "T upward", "", "t rightward", ""},
  {"", "ge≥", "eq=", "ge≥", "eq="},
  {"edges", "EdgesUPge[j,nk]", "EdgesUPeq[j,nk]", "edgesRIge[k,nk]", "edgesRIeq[k,nk]"},
  {"tree", "TreeUPge0[0,nk],TreeUPge[j,nk]", "TreeUPeq[j,nk]", "treeRIge[k,nk]", "treeRIeq[k,nk]"}},
  Dividers → {False, {True, False, True, False, True}},
  Alignment → {1 → Left}]
```

|       | $T$ upward                     |                 | $t$ rightward   |                 |
|-------|--------------------------------|-----------------|-----------------|-----------------|
|       | ge≥                            | eq=             | ge≥             | eq=             |
| edges | EdgesUPge[j,nk]                | EdgesUPeq[j,nk] | edgesRIge[k,nk] | edgesRIeq[k,nk] |
| tree  | TreeUPge0[0,nk],TreeUPge[j,nk] | TreeUPeq[j,nk]  | treeRIge[k,nk]  | treeRIeq[k,nk]  |

## Edge generating functions for trees $T_{\geq j}, T_j$ and $t_{\geq k}, t_k$

The edge generating functions below could have been integrated in one edge generating formula with more parameters.

EdgesUPge[j,nk] gives for tree  $T_{\geq j}$  the edges starting from its root  $n = \Omega_{\geq j} = U^j[4]$  for nk levels

```
In[167]:= EdgesUPge[j_, nk_] := Module[{n, k, gBegin, gResult, cBegin, cResult},
  n = uj[4, j];
  gBegin = {n};
  gResult = If[n > Last[uu[4, j]], {rj[n, j], u[n]}, {u[n]}];
  cResult = {{n, u[n]}, {n, rj[n, j]}};
  For[k = 1, k ≤ nk - 1, k++, {
    gBegin = gResult; cBegin = cResult;
    gResult = Flatten[gj[#, j] & /@ gResult];
    cResult = Partition[Flatten[Prepend[Transpose[{Flatten[List[#, #] & /@ gBegin], gResult}], cBegin]], 2]}}];
  Apply[Rule, cResult, {1}]]
```

EdgesUPeq generates the edges for tree  $T_j$

```

In[168]:= EdgesUPeq[j_, nk_] := Module[{n, k, gBegin, gResult, cBegin, cResult},
  n = uj[4, j];
  gBegin = {n};
  gResult = If[n > Last[uu[4, j]], {rj[n, j], u[n]}, {u[n]}];
  cResult = {{n, u[n]}, {n, rj[n, j]}};
  For[k = 1, k ≤ nk - 1, k++, {
    gBegin = gResult; cBegin = cResult;
    gResult = Flatten[gj[#, j] & /@ gResult];
    cResult = Partition[Flatten[Prepend[Transpose[{Flatten[List[#, #] & /@ gBegin], gResult}], cBegin]], 2]};
  cResult = Map[rj[#, j] &, cResult, {2}];
  Apply[Rule, cResult, {1}]];

```

edgesRIge[k,nk] gives the edges for the tree  $t_{\geq k}$

```

In[169]:= edgesRIge[k_, nk_] := Module[{edge00 = EdgesUPge[0, nk], edgeGEk},
  edgeGEk = Map[rk[#, k] &, edge00, {2}];
  Apply[Rule, edgeGEk, {1}]]

```

edgesRIeq[k,nk] gives the edges for the tree  $t_k$

```

In[170]:= edgesRIeq[k_, nk_] := Module[{edge00 = edgesRIge[k, nk], edgek},
  edgek = Map[uk[#, k] &, edge00, {2}];
  Apply[Rule, edgek, {1}]]

```

## Plot functions for trees $T_{\geq j}, T_j$ and $t_{\geq k}, t_k$

The plot generating functions below could have been integrated in one edge generating formula with more parameters and corresponding colour specifications

TreeUPge0[j,nk] plots nk bifurcations of the nested upward tree  $T_{\geq j}$  starting from its root  $n = \Omega_{\geq j} = U^j[4]$  for nk levels. The function is especially appropriate for plotting  $T_{\geq 0}$  with red and Blue as colours.

```

In[171]:= TreeUPge0[j_, nk_] := GraphPlot[
  Map[addnSj, EdgesUPge[j, nk], {2}],
  PlotRangePadding → 0,
  Method → {"LayeredDigraphEmbedding", "Rotation" → 15 Pi / 16},
  VertexLabels → {Placed[Automatic, Center]},
  VertexShapeFunction → (Text[Framed[#2, FrameStyle → White, Background → Which[
    upjQ[extnSj[#2], j],
    LightBlue,
    True,
    LightRed]], #1] &),
  EdgeShapeFunction → ({Which[
    And[upjQ[extnSj[Last[#2]], j], Mod[extnSj[Last[#2]], 18] == 16],
    Directive[Thickness[0.003], Lighter[Lighter[Blue]]],
    And[upjQ[extnSj[Last[#2]], j], Mod[extnSj[Last[#2]], 18] == 4],
    Directive[Thickness[0.004], Blue],
    extnSj[First[#2]] > extnSj[Last[#2]],
    Directive[Thick, Red],
    True,
    Directive[Thick, Lighter[Lighter[Red]]], Arrowheads[Medium], Arrow[#1, 0.18] &});

```

TreeUPge[j,nk] plots, just like TreeUPge0[j,nk], nk bifurcations of the nested upward tree  $T_{\geq j}$  starting from its root  $n = \Omega_{\geq j} = U^j[4]$  for nk levels. The function is especially appropriate for plotting  $T_{\geq j}$  for  $j > 0$  with two different shades of Blue (of upward numbers)



```

In[172]:= TreeUPge[j_, nk_] := GraphPlot[
  Map[addnSj, EdgesUPge[j, nk], {2}],
  PlotRangePadding → 0,
  Method → {"LayeredDigraphEmbedding", "Rotation" → 15 Pi / 16},
  VertexLabels → {Placed[Automatic, Center]},
  VertexShapeFunction → (Text[Framed[#2, FrameStyle → White, Background → Which[
    upjQ[extnSj[#2], j],
    Lighter[Lighter[Lighter[LightBlue]]],
    True,
    LightBlue]], #1] &),
  EdgeShapeFunction → ({Which[
    And[upjQ[extnSj[Last[#2]], j], Mod[extnSj[Last[#2]], 18] == 16],
    Directive[Thickness[0.003], Lighter[Lighter[Blue]]],
    And[upjQ[extnSj[Last[#2]], j], Mod[extnSj[Last[#2]], 18] == 4],
    Directive[Thickness[0.004], Blue],
    extnSj[First[#2]] > extnSj[Last[#2]],
    Directive[Thick, Red],
    True,
    Directive[Thick, Lighter[Lighter[Red]]], Arrowheads[Medium], Arrow[#1, 0.18] &})]; TreeUPge[1, 4]

```

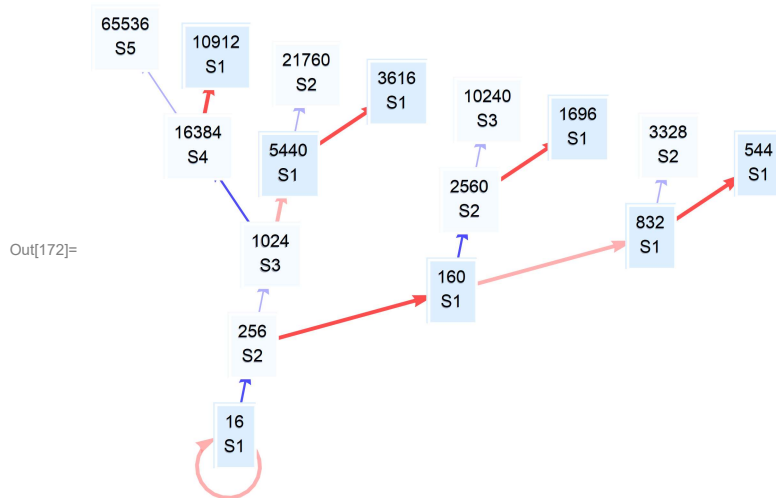

treeUPeq[j,nk] plots nk bifurcations of the disjoint upward tree  $T_j$

```

In[173]:= TreeUPeq[j_, nk_] := Module[{EdgesUPeqnk, assoc},
  EdgesUPeqnk = EdgesUPeq[j, nk];
  assoc = Association[Rule @@ {Last[#], rjQ[First[#], Last[#], j]} & /@ EdgesUPeqnk];
  GraphPlot[
    Map[addnSj, EdgesUPeqnk, {2}],
    PlotRangePadding → 0,
    Method → {"LayeredDigraphEmbedding", "Rotation" → 15 Pi / 16},
    VertexLabels → {Placed[Automatic, Center]},
    VertexShapeFunction → (Text[Framed[#2, FrameStyle → White, Background → Which[
      Lookup[assoc, extnSj[#2]],
      LightBlue,
      True,
      Lighter[Lighter[Lighter[LightBlue]]]], #1] &),
    EdgeShapeFunction → ({Which[
      And[upjQ[extnSj[Last[#2]], j], Mod[extnSj[Last[#2]], 18] == 16],
      Directive[Thickness[0.003], Lighter[Lighter[Blue]]],
      And[upjQ[extnSj[Last[#2]], j], Mod[extnSj[Last[#2]], 18] == 4],
      Directive[Thickness[0.004], Blue],
      extnSj[First[#2]] > extnSj[Last[#2]],
      Directive[Thick, Red],
      True,
      Directive[Thick, Lighter[Lighter[Red]]], Arrowheads[Medium], Arrow[#1, 0.18] &}]];

```

TreeRlge[j,nk] plots nk bifurcations of the nested rightward tree  $t_{\geq k}$  starting from its root  $n = \Omega_{\geq k} = R^k[4]$  for nk levels.

```

In[174]:= TreeRIge[j_, nk_] := GraphPlot[
  Map[addnS0k, edgesRIge[j, nk], {2}],
  PlotRangePadding → 0,
  Method → {"LayeredDigraphEmbedding", "Rotation" → 15 Pi / 16},
  VertexLabels → {Placed[Automatic, Center]},
  VertexShapeFunction → (Text[Framed[#2, FrameStyle → White, Background → Which[
    rkQ[extnS0k[#2], j],
    Lighter[Lighter[Lighter[LightRed]]],
    True,
    LightRed]], #1] &),
  EdgeShapeFunction → ({Which[
    And[rkQ[extnS0k[Last[#2]], j], extnS0k[First[#2]] < extnS0k[Last[#2]]],
    Directive[Thickness[0.003], Lighter[Red]],
    And[rkQ[extnS0k[Last[#2]], j], extnS0k[First[#2]] > extnS0k[Last[#2]]],
    Directive[Thick, Red],
    extnS0k[First[#2]] > extnS0k[Last[#2]],
    Directive[Thick, Red],
    True,
    Directive[Thick, Lighter[Lighter[Red]]]],
  Arrowheads[Medium], Arrow[#1, 0.18] &)]];

```

TreeRIeq[j,nk] plots nk bifurcations of the disjoint rightward tree  $t_k$  starting from its root  $n = \Omega_k = \Omega_{\geq k} = R^k[4]$  for nk levels.

```

In[175]:= TreeRIeq[j_, nk_] := Module[{EdgesUPeqnk, assoc},
  EdgesUPeqnk = edgesRIeq[j, nk];
  assoc = Association[Rule @@ {Last[#], ukQ[First[#], Last[#], j]} & /@ EdgesUPeqnk];
  GraphPlot[
    Map[addnS0k, EdgesUPeqnk, {2}],
    PlotRangePadding → 0,
    Method → {"LayeredDigraphEmbedding", "Rotation" → 15 Pi / 16},
    VertexLabels → {Placed[Automatic, Center]},
    VertexShapeFunction → (Text[Framed[#2, FrameStyle → White, Background → Which[
      Lookup[assoc, extnS0k[#2]],
      LightRed,
      True,
      Lighter[Lighter[LightBrown]]]], #1] &),
    EdgeShapeFunction → ({Which[
      And[rkQ[extnS0k[Last[#2]], j], extnS0k[First[#2]] < extnS0k[Last[#2]]],
      Directive[Thickness[0.003], Lighter[Orange]],
      And[rkQ[extnS0k[Last[#2]], j], extnS0k[First[#2]] > extnS0k[Last[#2]]],
      Directive[Thick, Orange],
      extnS0k[First[#2]] > extnS0k[Last[#2]],
      Directive[Thick, Red],
      True,
      Directive[Thick, Lighter[Lighter[Red]]]],
    Arrowheads[Medium], Arrow[#1, 0.18] &)]];

```

## Plots of subtrees included in the main text and the supplementary materials

Figure 2, reprinted as Figure S1.1 in the Supplementary Materials: tree  $T_{\geq 0}$ , 5 binary splits

In[176]:= **TreeUPge0[0, 5]**

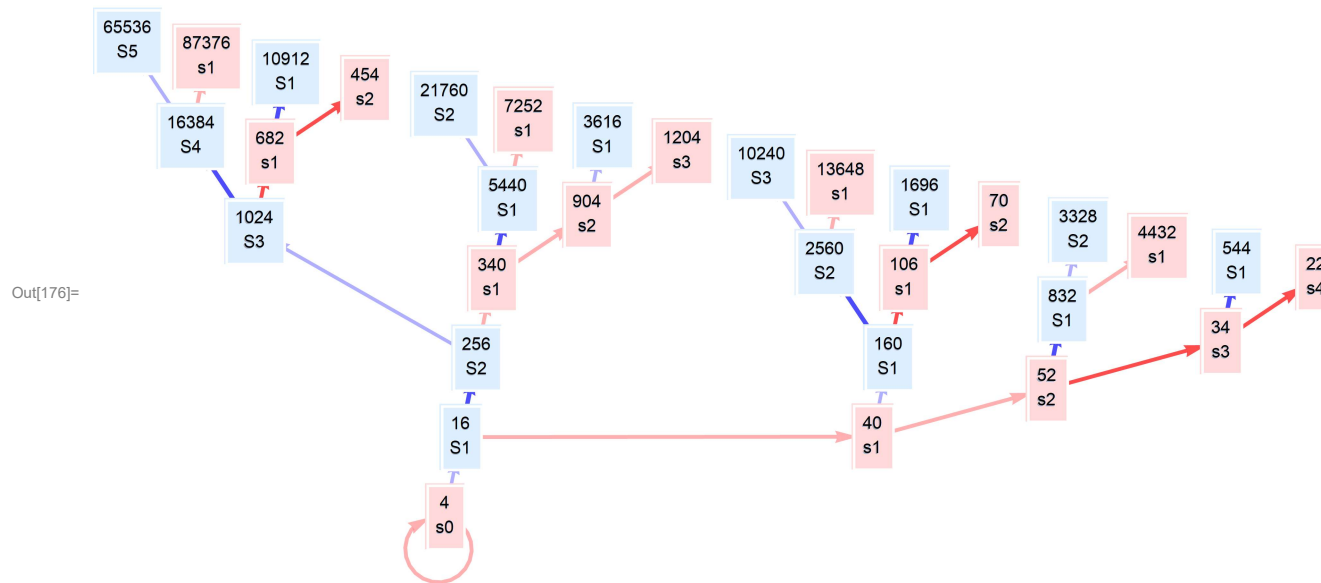

Fig 3 nested subtrees. left  $T_{\geq 1}, T_{\geq 2}$ , right  $t_{\geq 1}, t_{\geq 2}$

In[177]:= **GraphicsRow[{TreeUPge[1, 4], TreeRIge[1, 4]}]**

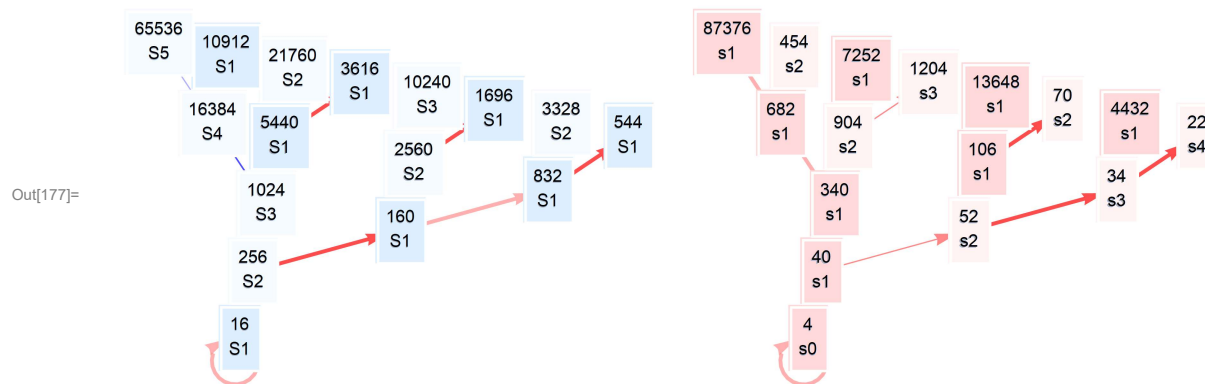

In[178]:= GraphicsRow[{TreeUPge[2, 4], TreeRIge[2, 4]}]

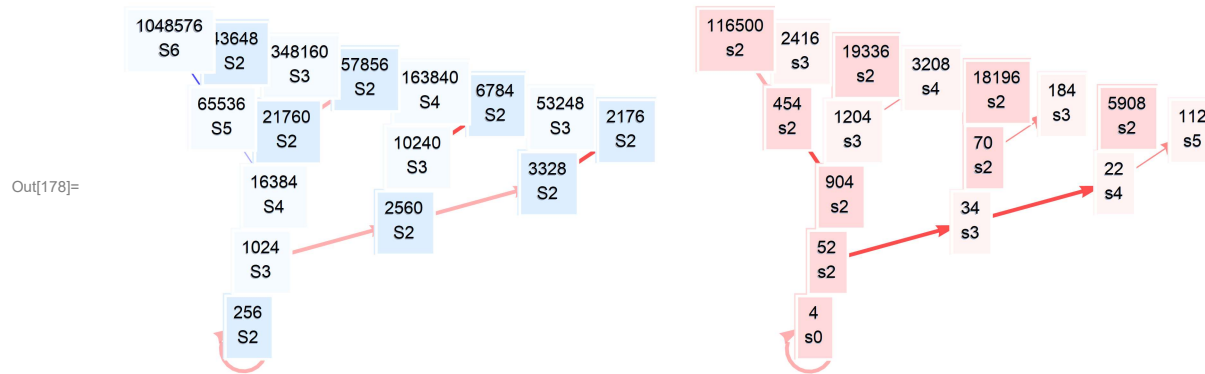

Fig 4 disjoint cotrees. left  $T_1, T_2$ , right  $t_1, t_2$

In[179]:= GraphicsRow[{TreeUPeq[1, 4], TreeRIeq[1, 4]}]

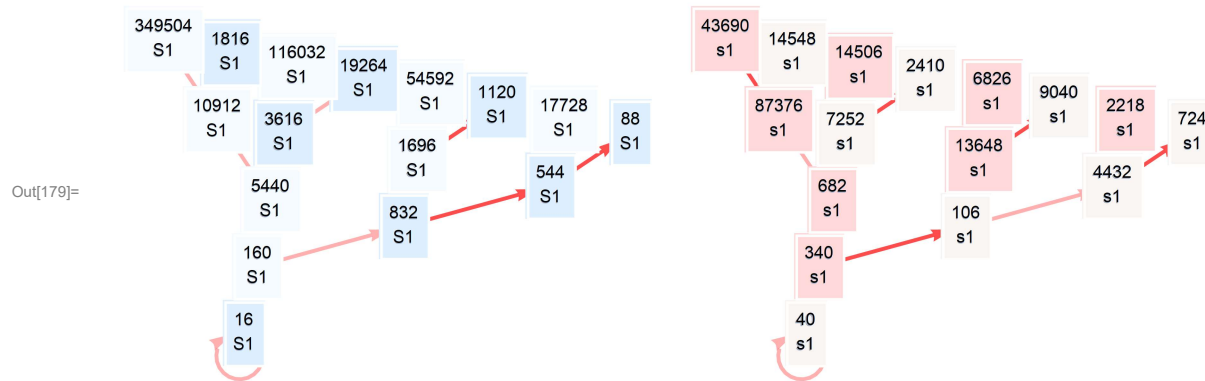

In[180]:= GraphicsRow[{TreeUPeq[2, 4], TreeRIeq[2, 4]}]

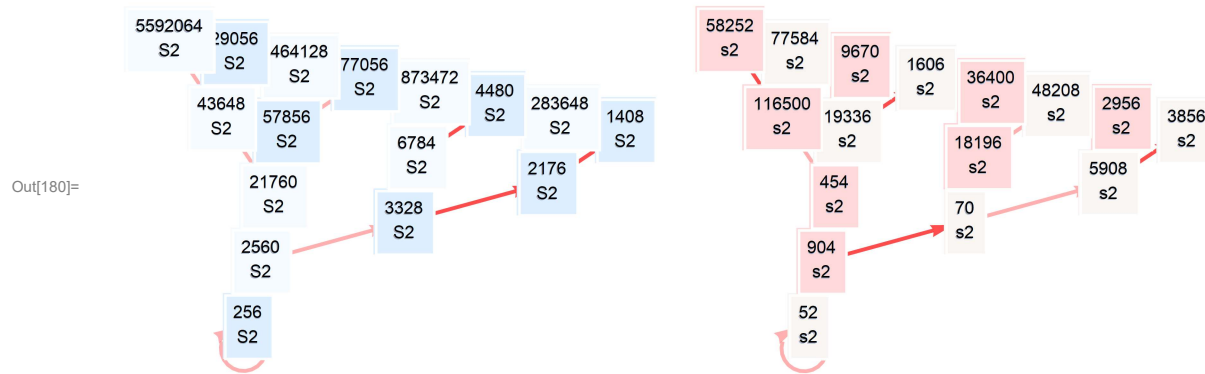

Figure 3 (4 panes), trees  $t_{\geq 1}=T_0, T_1, T_2, T_3$ , 4 binary splits

In[181]:= GraphicsRow[{TreeRIge[1, 4], TreeUPeq[1, 4]}]

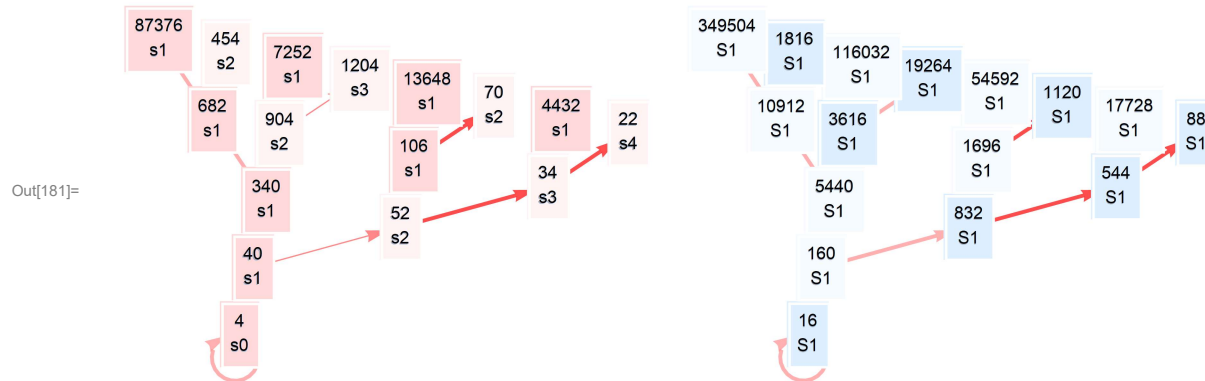

In[182]:= GraphicsRow[{TreeUPeq[2, 4], TreeUPeq[3, 4]}]

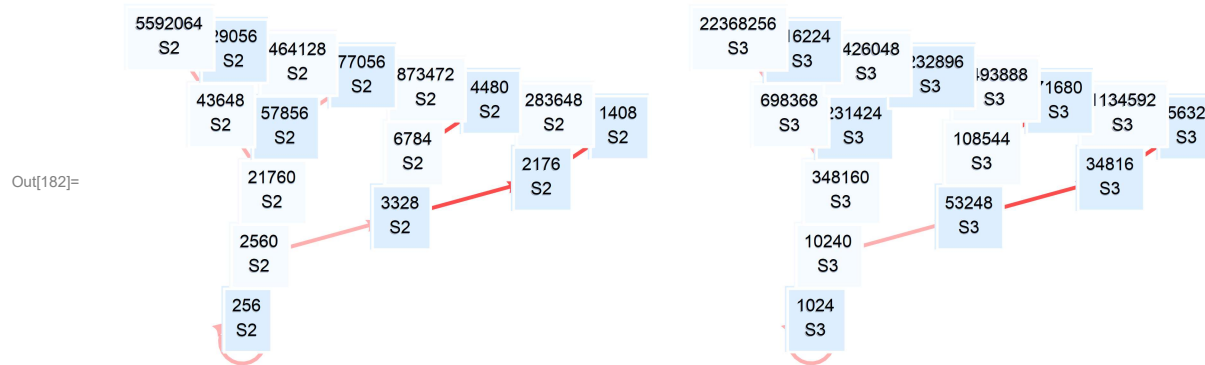

Figure 4 (4 panes), trees  $T_{\geq 1}=t_0, t_1, t_2, t_3$ , 4 binary splits

In[183]:= GraphicsRow[{TreeUPge[1, 4], TreeRIeq[1, 4]}]

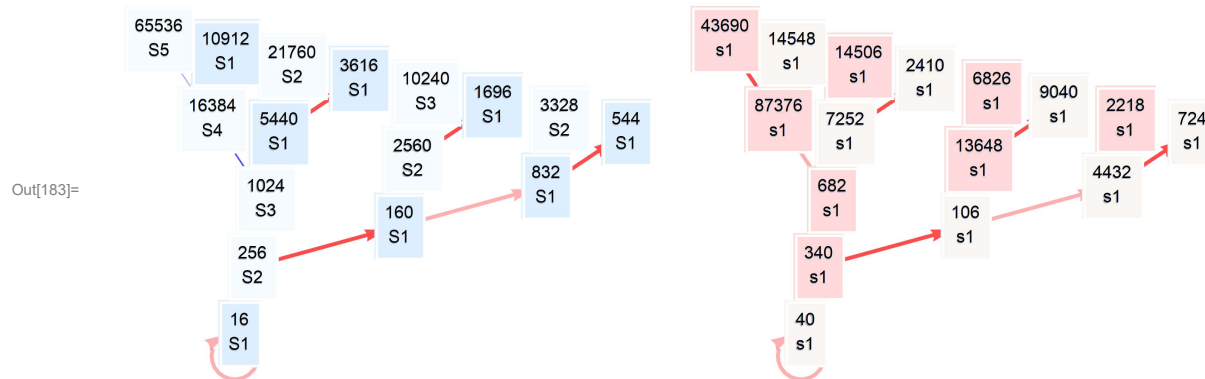



In[184]:= GraphicsRow[{TreeRieq[2, 4], TreeRieq[3, 4]}]

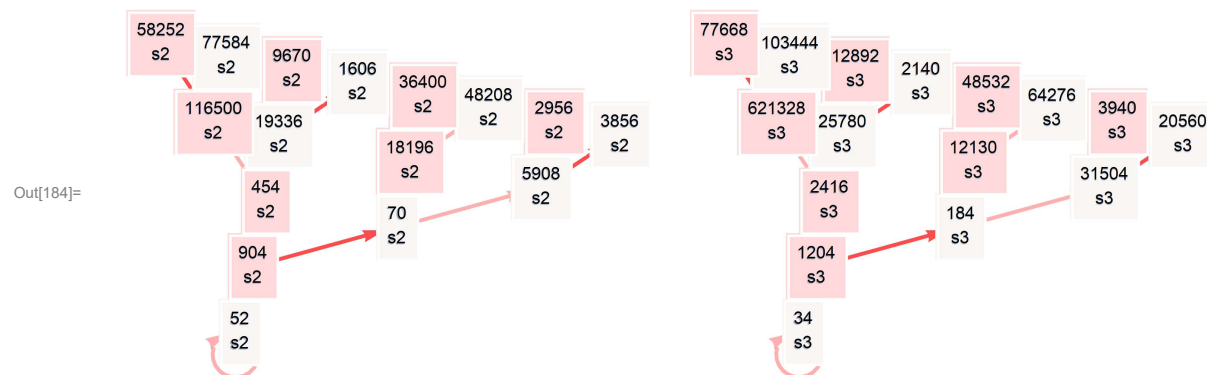

Supplementary Figure S1.2 Tree  $T_{\geq 1}=t_0$ , 5 binary splits

In[185]:= TreeUPge[1, 5]

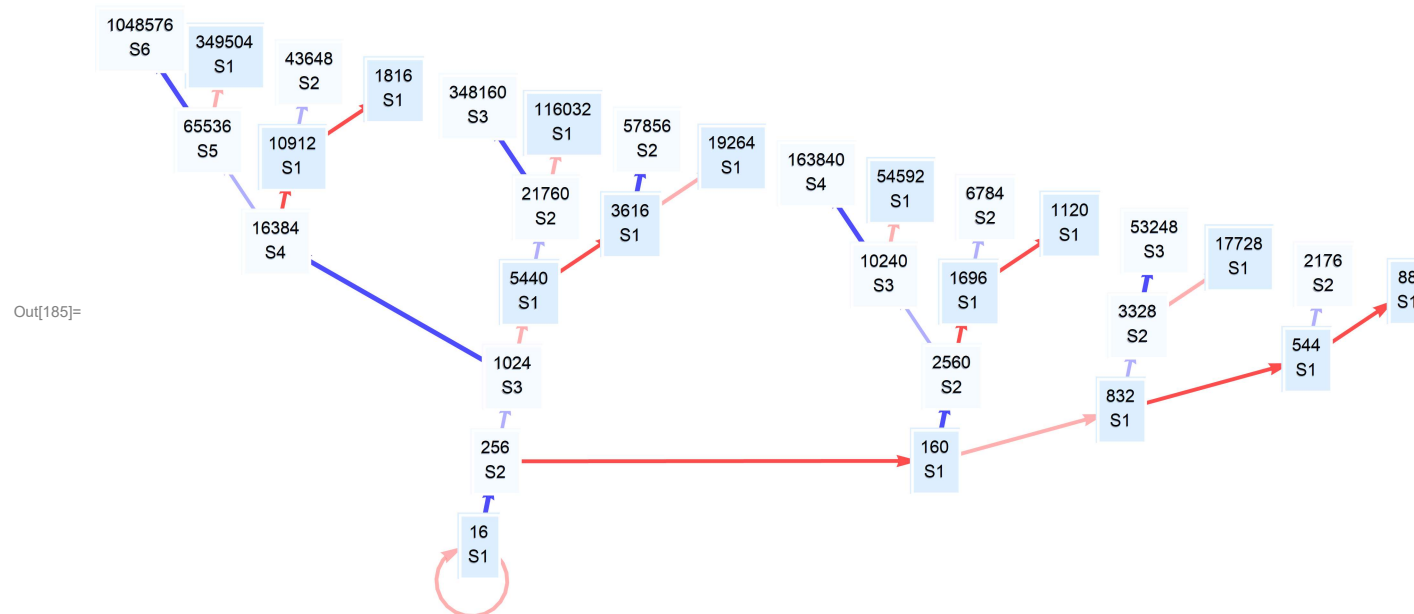

Supplementary Figure S1.3 Tree  $t_{\geq 1}=T_0$ , 5 binary splits

In[186]:= **TreeRige[1, 5]**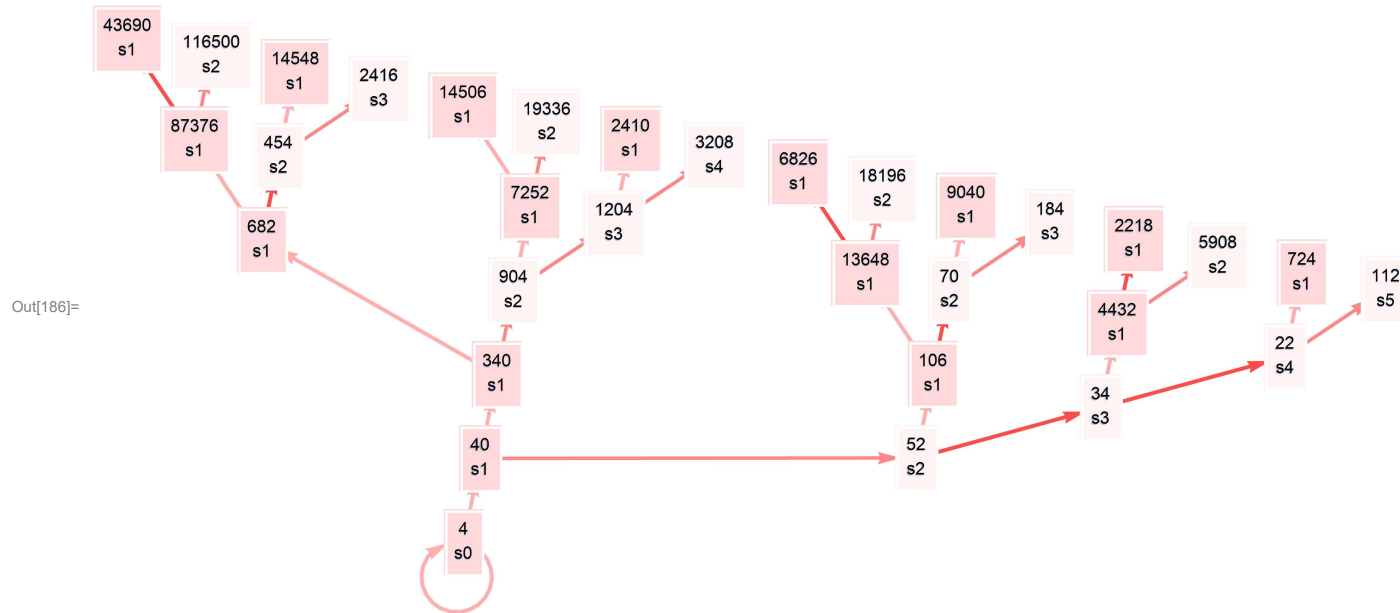

Supplementary Figures S1.4, S1.5, S1.6 (6 panes) nested upward trees  $T_{\geq 1}$ ,  $T_{\geq 2}$ ,  $T_{\geq 3}$  generate disjoint upward subtrees  $T_1$ ,  $T_2$ ,  $T_3$

In[187]:= **GraphicsRow[{TreeUPge[1, 4], TreeUPeq[1, 4]}]**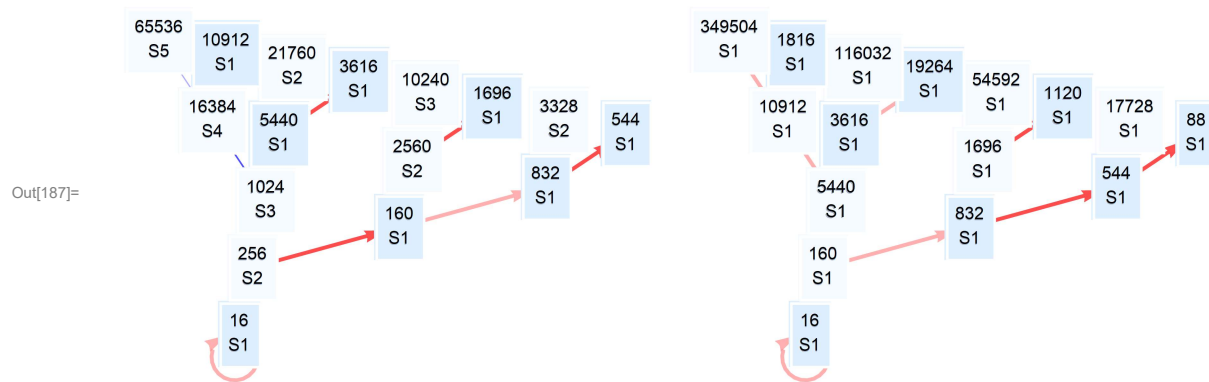

In[188]:= GraphicsRow[{TreeUPge[2, 4], TreeUPeq[2, 4]}]

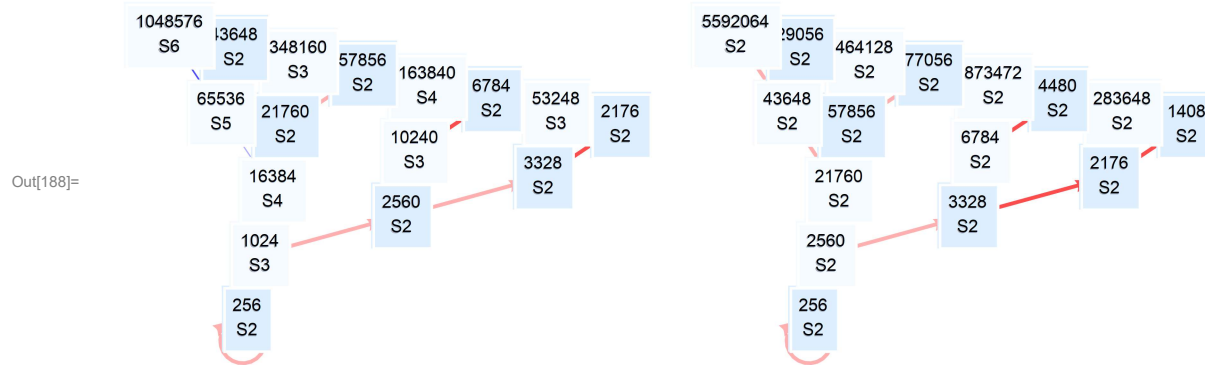

In[189]:= GraphicsRow[{TreeUPge[3, 4], TreeUPeq[3, 4]}]

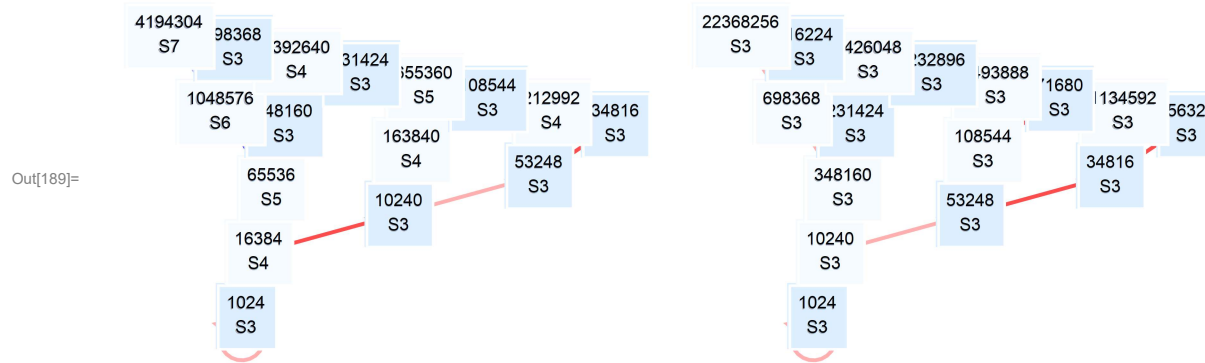

Supplementary Extended Data Figures 1 and 2 (8 panes) of nested upward subtrees  $T_{\geq 1}, T_{\geq 2}, T_{\geq 3}, \dots$  and disjoint upward cotrees  $T_1, T_2, T_3, \dots$

In[190]:= (\*GraphicsGrid[{  
 {TreeUPge[1,4],TreeUPeq[1,4]},  
 {TreeUPge[2,4],TreeUPeq[2,4]},  
 {TreeUPge[3,4],TreeUPeq[3,4]},  
 {TreeUPge[4,4],TreeUPeq[4,4]}}]\*)

Supplementary Extended Data Figures 1 and 2 (8 panes) of nested rightward trees  $t_{\geq 1}, t_{\geq 2}, t_{\geq 3}, \dots$  and disjoint rightward cotrees  $t_1, t_2, t_3, \dots$

```
In[191]:= (*GraphicsGrid[ {
  {TreeRIge[1,4],TreeRIeq[1,4]},
  {TreeRIge[2,4],TreeRIeq[2,4]},
  {TreeRIge[3,4],TreeRIeq[3,4]},
  {TreeRIge[4,4],TreeRIeq[4,4]} } ] *)
```

Supplementary Figures S1.7, S1.8, S1.9 (6 panes) nested rightward trees  $t_{\geq 1}, t_{\geq 2}, t_{\geq 3}$  generate disjoint rightward subtrees  $t_1, t_2, t_3$

tree  $T_{\geq 24}$  of which the lowest number  $\Omega_{\geq 24} = 18\,889\,465\,931\,478\,580\,854\,784 \approx 2^{74}$  is higher than the highest number of roughly  $2^{69.1}$  below all numbers have a verified root path according to computations by David Barina (<http://www.ericr.nl/wondrous/>).

```
In[192]:= Log[2, 18 889 465 931 478 580 854 784]
```

```
Out[192]= 74
```

In[193]:= **TreeUPge0[24, 3]**

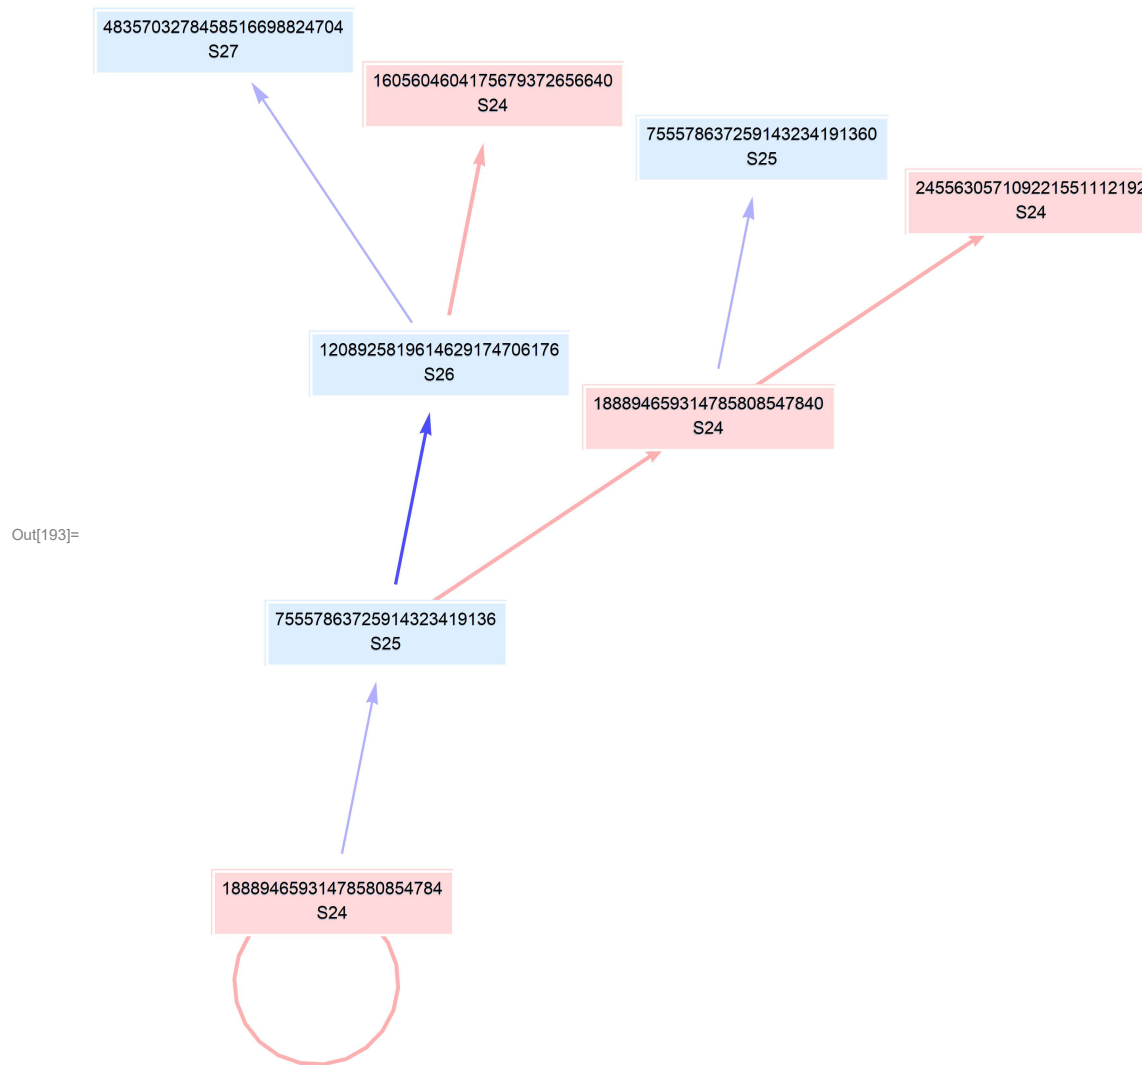

trees Supplementary Materials (Alt / uncomment)

In[194]:= (\*GraphicsColumn[{TreeUPge[1,5],TreeUPeq[1,5]}]\*)

In[195]:= (\*GraphicsColumn[{TreeUPge[2,5],TreeUPeq[2,5]}]\*)

```
In[196]:= (*GraphicsColumn[{TreeUPge[3,5],TreeUPeq[3,5]}]*)  
In[197]:= (*GraphicsColumn[{TreeUPge[4,5],TreeUPeq[4,5]}]*)  
In[198]:= (*GraphicsColumn[{TreeRIge[1,5],TreeRIeq[1,5]}]*)  
In[199]:= (*GraphicsColumn[{TreeRIge[2,5],TreeRIeq[2,5]}]*)  
In[200]:= (*GraphicsColumn[{TreeRIge[3,5],TreeRIeq[3,5]}]*)  
In[201]:= (*GraphicsColumn[{TreeRIge[4,5],TreeRIeq[4,5]}]*)  
In[202]:= (*GraphicsColumn[{TreeUPge0[100,2],TreeUPeq[100,2]}]*)  
In[203]:= (*GraphicsColumn[{TreeRIge[100,3],TreeRIeq[100,3]}]*)
```

## 6. Excursion to the Syracuse tree

The Syracuse tree is discussed in the introduction and the discussion section of the main text.

`syrPath[n]` is a Syracuse tree path based on the function `T[n]` that simply leaves all 2's (and without loss of generalization also all 3's with `syr23Path[n]`) out of the Collatz tree; each remaining node branches infinitely often (this claim from the main text is also shown by the `syrTree` plot and the `syr23Tree` plot below). it's length, or 'stopping time', of 42 is shorter than the stopping time 112 of the original Collatz path

```
In[204]:= syrPath[n_] := Select[colPath[n], OddQ[#] &]
```

```
In[205]:= syrPath[27]
```

```
Out[205]= {27, 41, 31, 47, 71, 107, 161, 121, 91, 137, 103, 155, 233, 175, 263, 395, 593, 445, 167, 251,
          377, 283, 425, 319, 479, 719, 1079, 1619, 2429, 911, 1367, 2051, 3077, 577, 433, 325, 61, 23, 35, 53, 5, 1}
```

```
In[206]:= Length /@ {colPath[27], syrPath[27]}
```

```
Out[206]= {112, 42}
```

`syrEdges[n,nk]` gives the arrows for  $nk$  levels of the Syracuse tree starting from  $n$

- with lightred rightward numbers in  $S_0$

- and lightBlue upward numbers in  $S_{\geq 1}$ .

```
In[207]:= syrEdges[n_, nk_] := Module[{nodes, edges, newNodes, newEdges, k},
  k = nk;
  newNodes = Table[If[OddQ[(2^p # - 1) / 3], (2^p # - 1) / 3, ## &[]], {p, 1, k}] &;
  newEdges = Table[If[OddQ[(2^p # - 1) / 3], # -> (2^p # - 1) / 3, ## &[]], {p, 1, k}] &;
  nodes = {n};
  edges = newEdges /@ nodes;
  For[nk == 1, k <= nk, k++, {
    nodes = DeleteCases[(newNodes /@ nodes) // Flatten, 1];
    edges = Append[edges, newEdges /@ nodes]
  }];
  edges // Flatten]
```

`syr23Edges[n, nk]` gives the arrows for  $nk$  levels of the Syracuse tree starting from  $n$ , with number nodes divisible by 3 omitted also

```

In[208]:= syr23Edges[n_, nk_] := Module[{nodes, edges, newNodes, newEdges, edg2, k},
  k = nk;
  newNodes = Table[If[n23Q[(2^p # - 1) / 3], (2^p # - 1) / 3, ## &[]], {p, 1, k}] &;
  newEdges = Table[If[n23Q[(2^p # - 1) / 3], # -> (2^p # - 1) / 3, ## &[]], {p, 1, k}] &;
  nodes = {n};
  edges = newEdges /@ nodes;
  For[nk == 1, k <= nk, k++, {
    nodes = DeleteCases[(newNodes /@ nodes) // Flatten, 1];
    edges = Append[edges, newEdges /@ nodes]
  }];
  edges // Flatten];

```

syrTree[n, j] plots  $j$  levels of the Syracuse tree starting from number  $n$ , on the basis of syrEdges[n, j]

- with lightred rightward numbers in  $S_0$

- and lightBlue upward numbers in  $S_{\geq 1}$ .

```

In[209]:= syrTree[n_, j_] := TreePlot[syrEdges[n, j], Bottom, n, PlotRangePadding -> 0, VertexLabels -> Placed[Automatic, Center],
  VertexShapeFunction ->
    (Text[Framed[#2, FrameStyle -> White, Background -> Which[Divisible[#2, 3], White, up15Q[#2], LightBlue, True, LightRed]], #1] &),
  EdgeShapeFunction -> (
    {Which[Divisible[Last[#2], 3], Dashed, up15Q[Last[#2]], Blue, True, Red], Arrowheads[Medium], Arrow[#1, 0.10]} &);
syrTree[1, 12]

```

Out[210]=

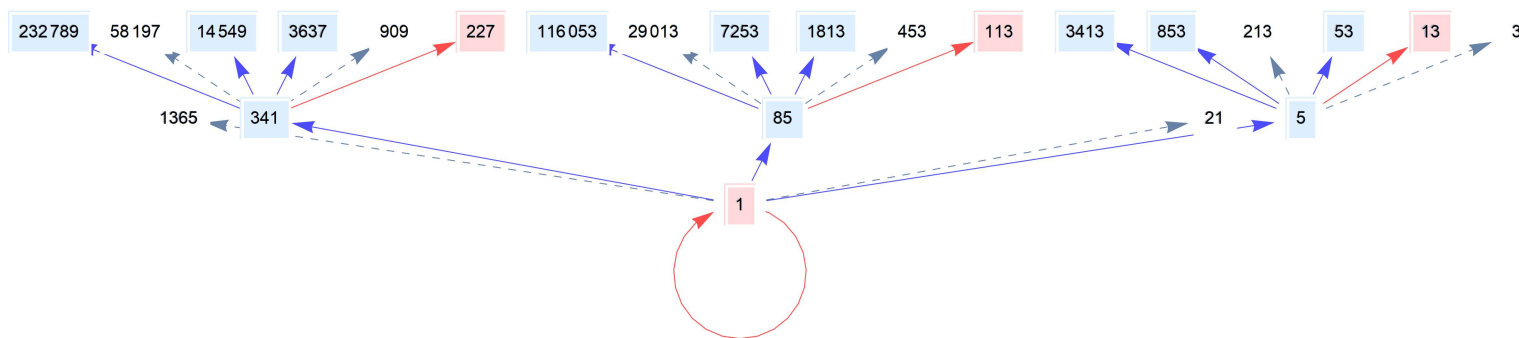

A syrTree shows that numbers divisible by 3 give rise to dead stakes in the Syracuse tree, which are removed in syr23tree below

syr23Tree[n, j] plots  $j$  levels of the Syracuse tree without odd number nodes divisible by 3 starting from number  $n$ , on the basis of syr23Edges[n, j]



- with lightred rightward connected by  $3n+1$  to numbers in  $S_0$
- and lightBlue numbers connected by  $3n+1$  to upward numbers in  $S_{\geq 1}$ .

A syr23tree shows that rightward numbers are minimum numbers in the infinite offspring of each number node. Note that each node splits to infinitely many other nodes, of which only 5 are shown, e.g.  $1 \rightarrow 1, 5, 85, 341, 5461, \dots$ . Note that (exclusively) the utmost right number in any infinite set of descendants is a lightred number connected by  $3n+1$  to numbers in  $S_0$

```

In[211]:= syr23Tree[n_, j_] := TreePlot[syr23Edges[n, j], Bottom, n, PlotRangePadding -> 0, VertexLabels -> Placed[Automatic, Center],
  VertexShapeFunction -> (Text[Framed[#2, FrameStyle -> White, Background -> Which[up15Q[#2], LightBlue, True, LightRed]], #1] &),
  EdgeShapeFunction -> (
    {Which[Divisible[Last[#2], 3], Dashed, up15Q[Last[#2]], Blue, True, Red], Arrowheads[Medium], Arrow[#1, 0.10]} &);
syr23Tree[1, 12]

```

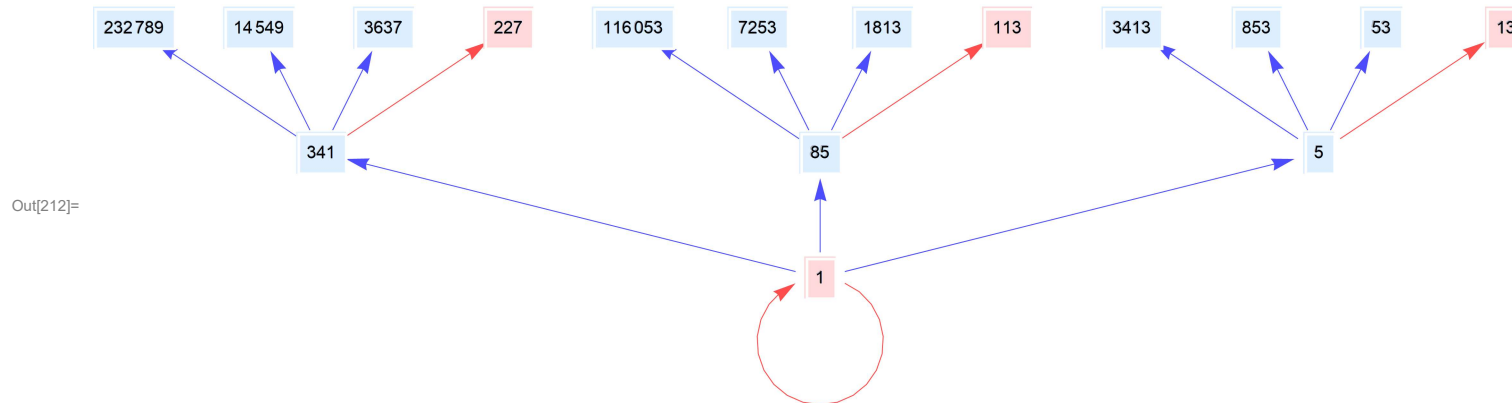

```

In[213]:= syr23Tree[1, 15]

```

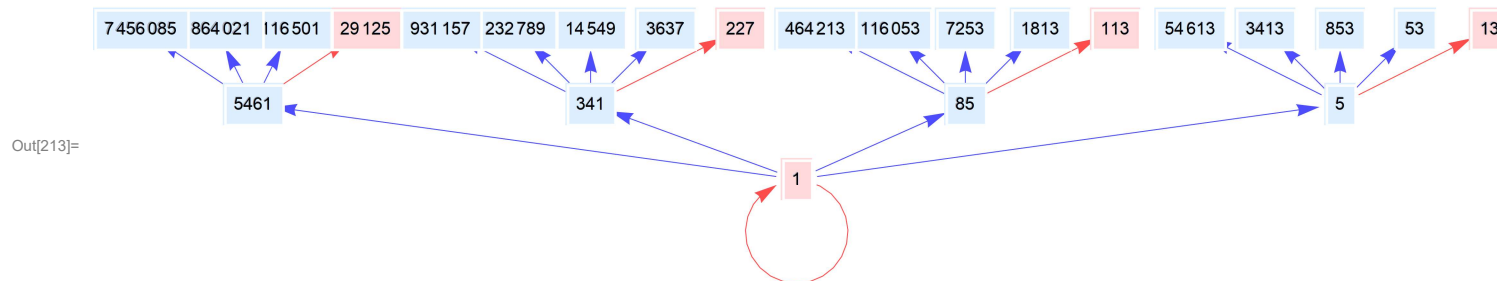

syr23TreeLst assumes (combined) Lst of edges made with syr23Edges[n, j],

```
In[214]:= syr23TreeLst[syr23EdgesLst_] := TreePlot[syr23EdgesLst, Bottom, 1, PlotRangePadding → 0, VertexLabels → Placed[Automatic, Center],
VertexShapeFunction → (Text[Framed[#2, FrameStyle → White, Background → Which[up15Q[#2], LightBlue, True, LightRed]], #1] &),
EdgeShapeFunction → (
{Which[Divisible[Last[#2], 3], Dashed, up15Q[Last[#2]], Blue, True, Red], Line[#1]} &)]
```

```
In[215]:= syr23TreeLst[Flatten[{syr23Edges[1, 10], syr23Edges[113, 10], syr23Edges[51413, 10]}]]
```

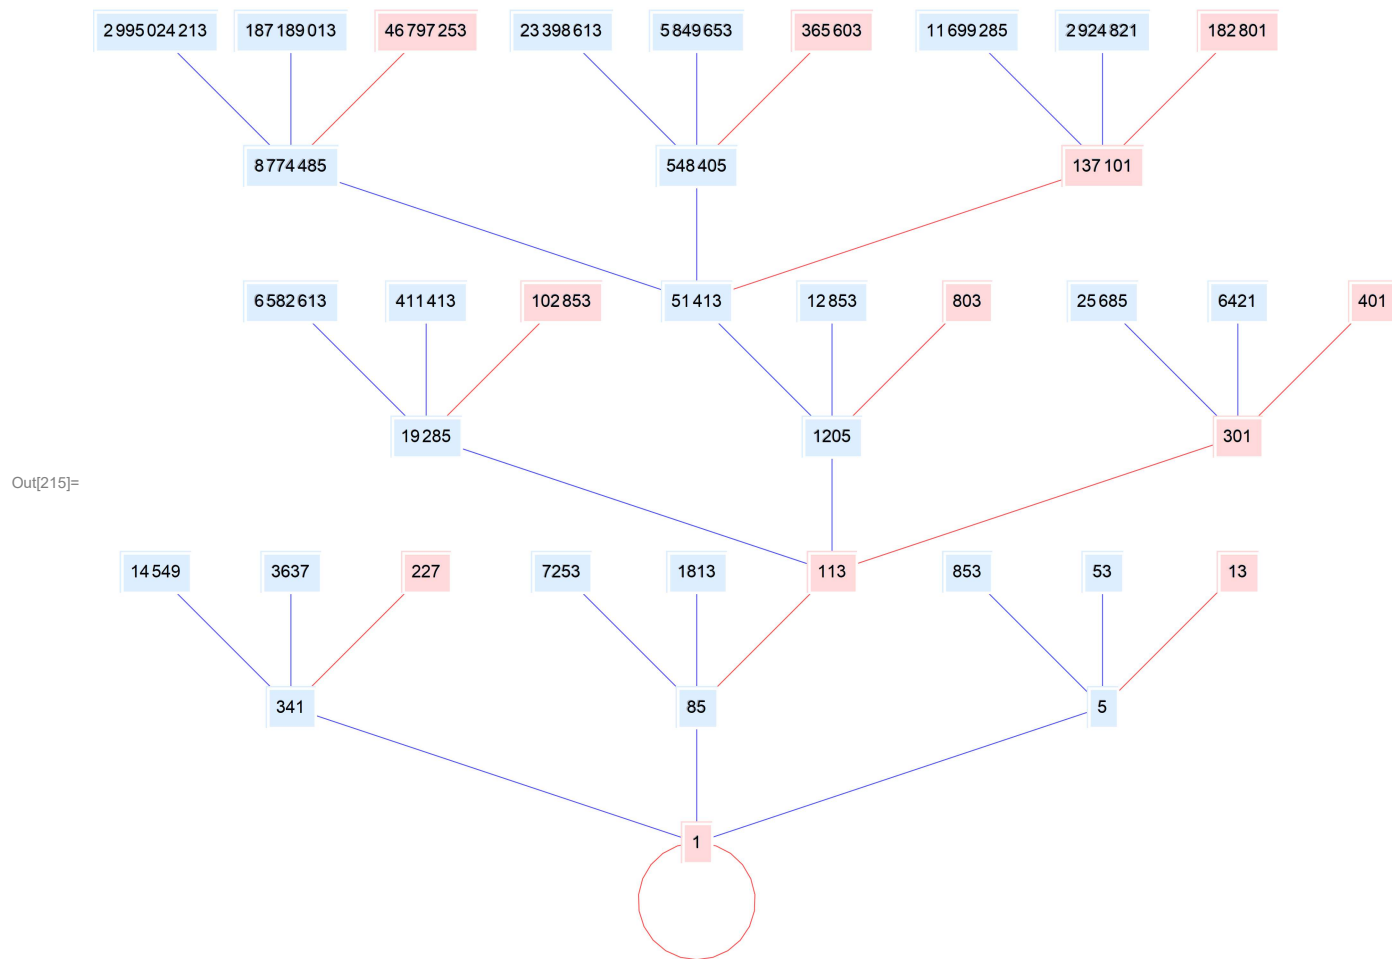

# 7. Densities subtrees and entire Collatz tree

## Plotting periodic rightward iterates

Figure S3.2 (Supplementary Materials) shows that rightward iterates are periodic rather than chaotic.

`perArgR[k]` is the periodicity of upward arguments to enable rightward iteration  $k$

```
In[216]:= perArgR[k_] :=  $2^5 \times 3^{k+2}$ ;
Table[perArgR[i], {i, 1, 8}]
```

```
Out[217]= {864, 2592, 7776, 23328, 69984, 209952, 629856, 1889568}
```

`plotPeriodicity[n,k,u,log,extraRiteration]` plots  $u$  periodic rightward iterations of length  $k$  starting from an upwards argument  $n$  on either a linear ( $\log = 0$ ) or a logarithmic scale with either (1) or not ( $\text{extraRiteration}=0$ ) one extraRiteration rightward iterate with a three times as large periodicity

```
In[218]:= plotPeriodicity[n_, k_, u_, log_, extraRiteration_] := Module[{per, rrtemp},
  per =  $2^5 \times 3^{k+2}$ ; rrtemp = (rr[#, k + extraRiteration] & /@ Table[n + i per, {i, 0, u - 1}]);
  If[log == 0,
    ListPlot[Callout[#, {#}] & /@ rrtemp,
      Ticks -> {FindDivisions[{Floor[#1], Ceiling[#2], 1}, 8] &, Automatic},
      ScalingFunctions -> "Linear", Joined -> True,
      DataRange -> {0, k + extraRiteration}, PlotStyle -> {Red, Lighter[Green], Blue}},
    ListPlot[Callout[#, {#}] & /@ rrtemp,
      Ticks -> {FindDivisions[{Floor[#1], Ceiling[#2], 1}, 8] &, Automatic},
      ScalingFunctions -> "Log", Joined -> True,
      DataRange -> {0, k + extraRiteration}, PlotStyle -> {Red, Lighter[Green], Blue}] ]]
```

In[219]:= **plotPeriodicity[16, 8, 7, 1, 0]**

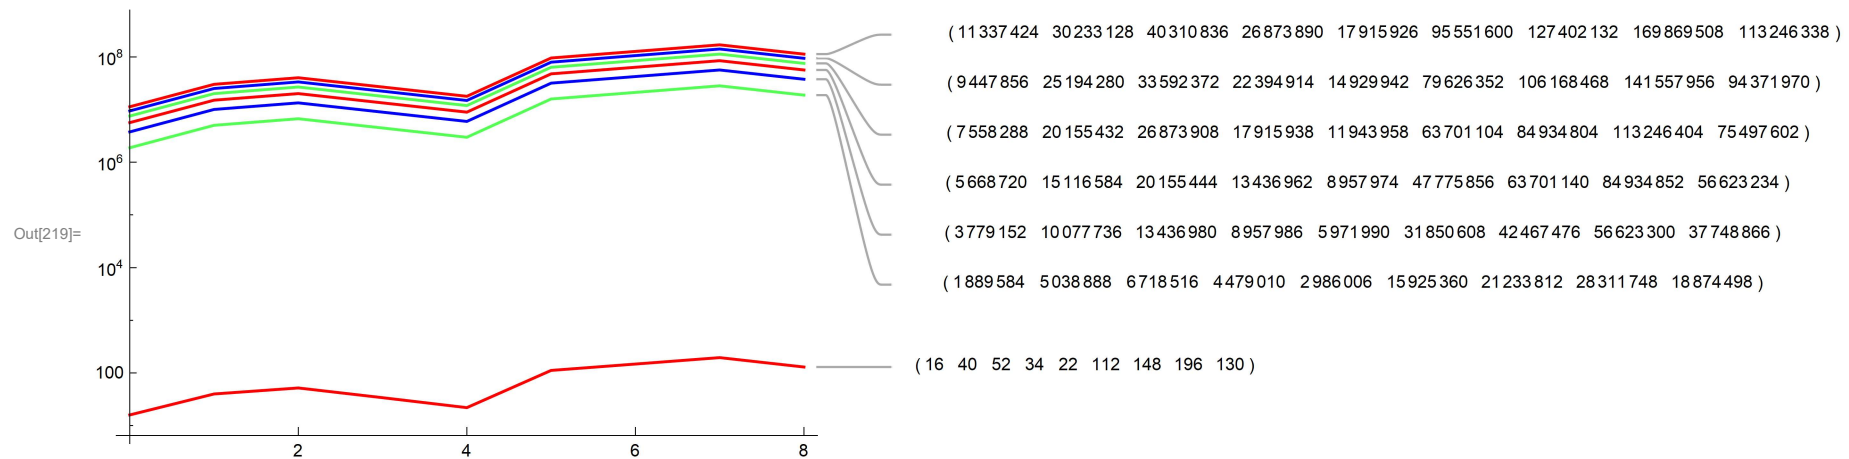

The plot `plotPeriodicity[16,8,7,1,0]` is based on the periodicity of  $j=0..7$  arguments for  $k=8$  iterations thus for `perArgR[8]`, starting from  $n[1]=16$ , until  $n[7]=16+(7-1) \text{ perArgR}[8]=11\,337\,424$ , in which `perArgR[8]=1\,889\,568`.

The `perArgR[8]` table below shows the 7 arguments for 8 periodic rightward iterations starting from 16 in `plotPeriodicity[16,8,7,1,0]`

In[220]:= **Table[16 + i perArgR[8], {i, 0, 7 - 1}]**

Out[220]= {16, 1889584, 3779152, 5668720, 7558288, 9447856, 11337424}

These arguments which deliver periodic iterates until the  $k=8$ th iteration are plotted on the Y-axis in the Figure above, and printed as the most far-left number in the number rows to the right of the Figure.

For one out of 3 successive iterates the iterates are still periodic at the 9' th iteration. Every third iterate that is periodic to the orbit  $R^9(16)$  is depicted in red in the Figure below.

In[221]:= **plotPeriodicity[16, 8, 7, 1, 1]**

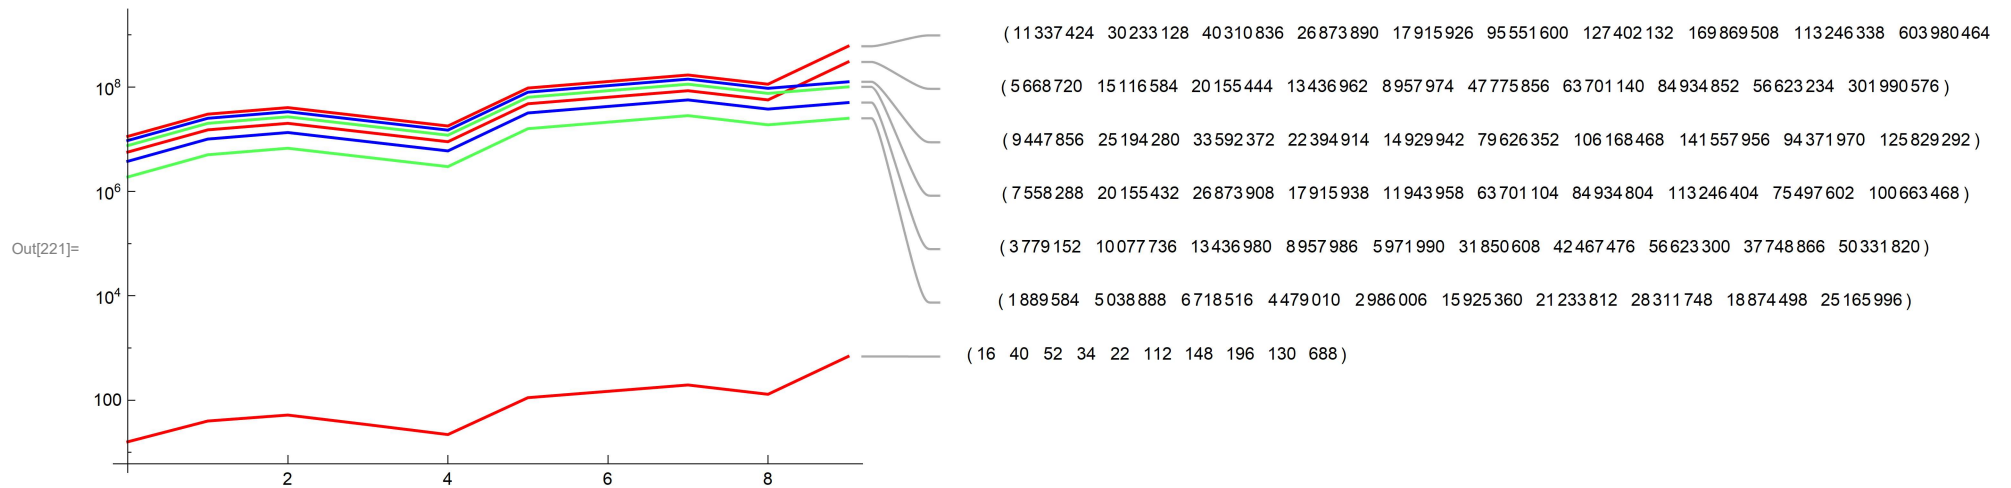

The upward arguments and rightward iterations that are still periodic at iteration 9 can, of course, also be generated directly by  $k=0..9$  rightward iterations  $rk[\#,k]$  applied to each argument  $\#$  from the Table of arguments  $16+j$  perArgR[9]

In[222]:= **Table[rk[#, k], {k, 0, 9}] & /@**

**Table[16 + j perArgR[9], {j, 0, 2}]**

Out[222]= {{16, 40, 52, 34, 22, 112, 148, 196, 130, 688},  
 {5 668 720, 15 116 584, 20 155 444, 13 436 962, 8 957 974, 47 775 856, 63 701 140, 84 934 852, 56 623 234, 301 990 576},  
 {11 337 424, 30 233 128, 40 310 836, 26 873 890, 17 915 926, 95 551 600, 127 402 132, 169 869 508, 113 246 338, 603 980 464}}

## Periodicity, cardinality, density

The grid below lists the labels of functions to assess the periodicity, cardinality and density of upward (odd and even) and rightward subtrees

```
In[223]:= Grid[{{"", "periodicity", "cardinality", "density", "total density"}, {"nonBranchingNodes", "", "", "", "dnsNonBranching"},
  {"upward,Odd", "perUo[i]", "crdUo[i]", "dnsUo[i]", "dnsUpOdd"},
  {"upward,Even", "perUe[j]", "crdUe[j]", "dnsUe[j]", "dnsUpEven"}, {"rightward", "perR[k]", "crdR[k]", "dnsR[k]", "dnsRight"},
  {"Collatz Tree", "", "", "", "dnsCollatzTree"}},
  Dividers → {False, {True, True, False, False, False, True, True}},
  Alignment → {1 → Left}]
```

|                   | periodicity | cardinality | density  | total density   |
|-------------------|-------------|-------------|----------|-----------------|
| nonBranchingNodes |             |             |          | dnsNonBranching |
| upward,Odd        | perUo[i]    | crdUo[i]    | dnsUo[i] | dnsUpOdd        |
| upward,Even       | perUe[j]    | crdUe[j]    | dnsUe[j] | dnsUpEven       |
| rightward         | perR[k]     | crdR[k]     | dnsR[k]  | dnsRight        |
| Collatz Tree      |             |             |          | dnsCollatzTree  |

```
In[224]:= dnsNonBranching = 16 / 18
```

```
Out[224]=  $\frac{8}{9}$ 
```

upward function, even iterations j

```
In[225]:= perUe[j_] := 288 × 23j;
  crdUe[j_] := 27;
  dnsUe[j_] := crdUe[j] / perUe[j];
  dnsUpEven = dnsUe[2] / (1 - (dnsUe[4] / dnsUe[2]))
```

```
Out[227]=  $\frac{1}{672}$ 
```

upward function, odd iterations i

```
In[228]:= perUo[i_] := 4608 × 23(i-1);
  crdUo[i_] := 72;
  dnsUo[i_] := crdUo[i] / perUo[i];
  dnsUpOdd = dnsUo[1] / (1 - (dnsUo[3] / dnsUo[1]))
```

```
Out[230]=  $\frac{1}{63}$ 
```

```
In[231]:= dnsUpCumulative[nj_] := Table[If[EvenQ[j], dnsUe[j], dnsUo[j]], {j, 1, nj}] // Accumulate
```

The table above and the ListPlot below shows that upward density convergence to the limit with  $r=1/64$  is much faster than rightward density convergence with  $r=13/16$

```
In[232]:= convergencePlotS = ListPlot[{dnsUpCumulative[4],
  Table[
    5 / 288, {i, 4}]],
  AxesOrigin → {1, 0}, PlotRange → {0, 0.02}, Joined → True,
  Ticks → {{1, 2, 3, 4}, Automatic},
  Epilog → {Text["5/288 = 0.0173611", {3.5, 0.0182}]}],
  AxesLabel → {"k", "Density"},
  PlotStyle → {Blue, {Black, Dotted}}]
```

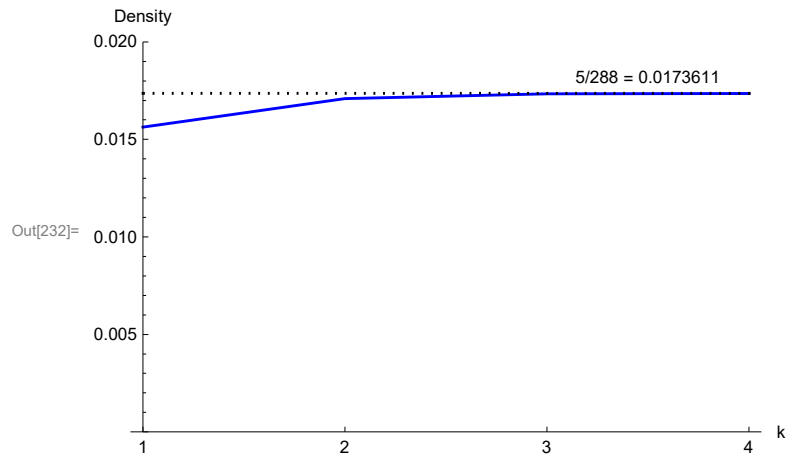

rightward function, iterations  $k$

```
In[233]:= perR[k_] := 4608 × 24(k-1);
  crdR[k_] := 81 × 13k-1;
  dnsR[k_] := crdR[k] / perR[k];
  dnsRight = dnsR[1] / (1 - (dnsR[2] / dnsR[1]))
```

```
Out[235]:= 3/32
```

```
In[236]:= dnsOutRcumulative[nk_] := Table[dnsRight[k], {k, 1, nk}] // Accumulate
```

The table above and the ListPlot below shows that upward density convergence to the limit with  $r=1/64$  is much faster than rightward density convergence
